# Supplementary material for: Accelerated simulation of Boltzmann-BGK equations near the diffusive limit with asymptotic-preserving multilevel Monte Carlo
Source: arXiv:2205.12130 source file (2023-02-25)
Supplement: Supplementary file 1 [file supplementarytables.pdf]

# Tables corresponding with the simulations for Figures 4 and 5 in "Accelerated simulation of Boltzmann-BGK equations near the diffusive limit with asymptotic-preserving multilevel Monte Carlo"

Emil Løvbak    Giovanni Samaey

May 24, 2022

## Contents

**1 Tables corresponding with Figure 4** **1**
1.1 Term-by-term correlation, $\varepsilon = 0.5$ . . . . . 1
1.2 Term-by-term correlation, $\varepsilon = 0.1$ . . . . . 4
1.3 Term-by-term correlation, $\varepsilon = 0.05$ . . . . . 8
1.4 Combined correlation, $\varepsilon = 0.5$ . . . . . 12
1.5 Combined correlation, $\varepsilon = 0.1$ . . . . . 15
1.6 Combined correlation, $\varepsilon = 0.05$ . . . . . 18

**2 Tables corresponding with Figure 5** **22**
2.1 Term-by-term correlation, $\varepsilon = 0.5$ . . . . . 22
2.2 Term-by-term correlation, $\varepsilon = 0.1$ . . . . . 25
2.3 Term-by-term correlation, $\varepsilon = 0.05$ . . . . . 29
2.4 Combined correlation, $\varepsilon = 0.5$ . . . . . 33
2.5 Combined correlation, $\varepsilon = 0.1$ . . . . . 36
2.6 Combined correlation, $\varepsilon = 0.05$ . . . . . 40

# 1 Tables corresponding with Figure 4

## 1.1 Term-by-term correlation, $\varepsilon = 0.5$

Table 1: $\varepsilon = 0.5$, $\Delta t_1 = 2.50 \times 10^{-1}$

| $\ell$ | $\Delta t_\ell$ | $P_\ell$ | $\mathbb{E}[\hat{F}_\ell - \hat{F}_{\ell-1}]$ | $\mathbb{V}[\hat{F}_\ell - \hat{F}_{\ell-1}]$ | $\mathbb{V}[\hat{Y}_\ell]$ | $P_\ell C_\ell$ |
|---|---|---|---|---|---|---|
| 0 | $5.0\times10^{-1}$ | $3.1\times10^{7}$ | $7.78\times10^{-1}$ | $1.2\times10^{0}$ | $3.9\times10^{-8}$ | $6.2\times10^{5}$ |
| 1 | $2.5\times10^{-1}$ | $6.5\times10^{6}$ | $-9.01\times10^{-2}$ | $1.6\times10^{-1}$ | $2.5\times10^{-8}$ | $3.9\times10^{5}$ |
| 2 | $1.2\times10^{-1}$ | $4.2\times10^{6}$ | $-6.61\times10^{-2}$ | $1.3\times10^{-1}$ | $3.1\times10^{-8}$ | $5.0\times10^{5}$ |
| 3 | $6.2\times10^{-2}$ | $2.4\times10^{6}$ | $-3.41\times10^{-2}$ | $8.7\times10^{-2}$ | $3.6\times10^{-8}$ | $5.8\times10^{5}$ |
| 4 | $3.1\times10^{-2}$ | $1.3\times10^{6}$ | $-1.31\times10^{-2}$ | $5.1\times10^{-2}$ | $3.9\times10^{-8}$ | $6.3\times10^{5}$ |
| 5 | $1.6\times10^{-2}$ | $6.9\times10^{5}$ | $-4.20\times10^{-3}$ | $2.8\times10^{-2}$ | $4.1\times10^{-8}$ | $6.6\times10^{5}$ |
| 6 | $7.8\times10^{-3}$ | $3.6\times10^{5}$ | $-1.22\times10^{-3}$ | $1.5\times10^{-2}$ | $4.3\times10^{-8}$ | $6.8\times10^{5}$ |
| 7 | $3.9\times10^{-3}$ | $1.8\times10^{5}$ | $-4.99\times10^{-4}$ | $8.0\times10^{-3}$ | $4.4\times10^{-8}$ | $7.0\times10^{5}$ |
| 8 | $2.0\times10^{-3}$ | $9.1\times10^{4}$ | $-1.64\times10^{-4}$ | $4.0\times10^{-3}$ | $4.4\times10^{-8}$ | $7.0\times10^{5}$ |
| 9 | $9.8\times10^{-4}$ | $4.6\times10^{4}$ | $-4.44\times10^{-5}$ | $2.1\times10^{-3}$ | $4.5\times10^{-8}$ | $7.1\times10^{5}$ |
| 10 | $4.9\times10^{-4}$ | $2.8\times10^{4}$ | $-2.37\times10^{-4}$ | $1.1\times10^{-3}$ | $4.0\times10^{-8}$ | $8.5\times10^{5}$ |
| 11 | $2.4\times10^{-4}$ | $1.8\times10^{4}$ | $-9.39\times10^{-5}$ | $5.0\times10^{-4}$ | $2.8\times10^{-8}$ | $1.1\times10^{6}$ |
| 12 | $1.2\times10^{-4}$ | $1.0\times10^{3}$ | $2.68\times10^{-4}$ | $1.9\times10^{-4}$ | $1.9\times10^{-7}$ | $1.2\times10^{5}$ |
| $\sum$ | | | $5.68\times10^{-1}$ | | $6.4\times10^{-7}$ | $8.2\times10^{6}$ |

Table 2: $\varepsilon = 0.5$, $\Delta t_1 = 1.25 \times 10^{-1}$

| $\ell$ | $\Delta t_\ell$ | $P_\ell$ | $\mathbb{E}[\hat{F}_\ell - \hat{F}_{\ell-1}]$ | $\mathbb{V}[\hat{F}_\ell - \hat{F}_{\ell-1}]$ | $\mathbb{V}[\hat{Y}_\ell]$ | $P_\ell C_\ell$ |
|---|---|---|---|---|---|---|
| 0 | $5.0\times10^{-1}$ | $2.3\times10^{7}$ | $7.78\times10^{-1}$ | $1.2\times10^{0}$ | $5.1\times10^{-8}$ | $4.6\times10^{5}$ |
| 1 | $1.2\times10^{-1}$ | $6.2\times10^{6}$ | $-1.57\times10^{-1}$ | $4.3\times10^{-1}$ | $6.9\times10^{-8}$ | $6.2\times10^{5}$ |
| 2 | $6.2\times10^{-2}$ | $1.8\times10^{6}$ | $-3.44\times10^{-2}$ | $8.7\times10^{-2}$ | $4.8\times10^{-8}$ | $4.3\times10^{5}$ |
| 3 | $3.1\times10^{-2}$ | $9.9\times10^{5}$ | $-1.36\times10^{-2}$ | $5.2\times10^{-2}$ | $5.3\times10^{-8}$ | $4.7\times10^{5}$ |
| 4 | $1.6\times10^{-2}$ | $5.2\times10^{5}$ | $-4.12\times10^{-3}$ | $2.9\times10^{-2}$ | $5.5\times10^{-8}$ | $5.0\times10^{5}$ |
| 5 | $7.8\times10^{-3}$ | $2.7\times10^{5}$ | $-1.33\times10^{-3}$ | $1.5\times10^{-2}$ | $5.7\times10^{-8}$ | $5.1\times10^{5}$ |
| 6 | $3.9\times10^{-3}$ | $1.4\times10^{5}$ | $-3.40\times10^{-4}$ | $8.0\times10^{-3}$ | $5.9\times10^{-8}$ | $5.3\times10^{5}$ |
| 7 | $2.0\times10^{-3}$ | $6.8\times10^{4}$ | $-3.19\times10^{-4}$ | $4.0\times10^{-3}$ | $5.9\times10^{-8}$ | $5.2\times10^{5}$ |
| 8 | $9.8\times10^{-4}$ | $2.9\times10^{4}$ | $3.45\times10^{-5}$ | $2.0\times10^{-3}$ | $6.7\times10^{-8}$ | $4.5\times10^{5}$ |
| 9 | $4.9\times10^{-4}$ | $1.0\times10^{3}$ | $8.36\times10^{-5}$ | $7.8\times10^{-4}$ | $7.8\times10^{-7}$ | $3.1\times10^{4}$ |
| $\sum$ | | | $5.67\times10^{-1}$ | | $1.3\times10^{-6}$ | $4.5\times10^{6}$ |

Table 3: $\varepsilon = 0.5$, $\Delta t_1 = 6.25 \times 10^{-2}$

| $\ell$ | $\Delta t_\ell$ | $P_\ell$ | $\mathbb{E}[\hat{F}_\ell - \hat{F}_{\ell-1}]$ | $\mathbb{V}[\hat{F}_\ell - \hat{F}_{\ell-1}]$ | $\mathbb{V}[\hat{Y}_\ell]$ | $P_\ell C_\ell$ |
|---|---|---|---|---|---|---|
| 0 | $5.0\times10^{-1}$ | $2.8\times10^{7}$ | $7.77\times10^{-1}$ | $1.2\times10^{0}$ | $4.2\times10^{-8}$ | $5.7\times10^{5}$ |
| 1 | $6.2\times10^{-2}$ | $7.3\times10^{6}$ | $-1.91\times10^{-1}$ | $7.0\times10^{-1}$ | $9.6\times10^{-8}$ | $1.3\times10^{6}$ |
| 2 | $3.1\times10^{-2}$ | $1.2\times10^{6}$ | $-1.39\times10^{-2}$ | $5.2\times10^{-2}$ | $4.3\times10^{-8}$ | $5.8\times10^{5}$ |
| 3 | $1.6\times10^{-2}$ | $6.4\times10^{5}$ | $-4.26\times10^{-3}$ | $2.8\times10^{-2}$ | $4.5\times10^{-8}$ | $6.1\times10^{5}$ |
| 4 | $7.8\times10^{-3}$ | $3.3\times10^{5}$ | $-1.27\times10^{-3}$ | $1.5\times10^{-2}$ | $4.6\times10^{-8}$ | $6.3\times10^{5}$ |
| 5 | $3.9\times10^{-3}$ | $1.7\times10^{5}$ | $-3.28\times10^{-4}$ | $7.8\times10^{-3}$ | $4.7\times10^{-8}$ | $6.4\times10^{5}$ |
| 6 | $2.0\times10^{-3}$ | $8.4\times10^{4}$ | $-3.19\times10^{-4}$ | $4.0\times10^{-3}$ | $4.8\times10^{-8}$ | $6.5\times10^{5}$ |
| 7 | $9.8\times10^{-4}$ | $4.1\times10^{4}$ | $1.35\times10^{-4}$ | $1.9\times10^{-3}$ | $4.7\times10^{-8}$ | $6.4\times10^{5}$ |
| 8 | $4.9\times10^{-4}$ | $2.2\times10^{4}$ | $2.18\times10^{-4}$ | $9.2\times10^{-4}$ | $4.2\times10^{-8}$ | $6.7\times10^{5}$ |
| 9 | $2.4\times10^{-4}$ | $9.3\times10^{3}$ | $-1.24\times10^{-4}$ | $4.9\times10^{-4}$ | $5.3\times10^{-8}$ | $5.7\times10^{5}$ |
| 10 | $1.2\times10^{-4}$ | $1.0\times10^{3}$ | $-1.13\times10^{-4}$ | $1.9\times10^{-4}$ | $1.9\times10^{-7}$ | $1.2\times10^{5}$ |
| $\sum$ | | | $5.67\times10^{-1}$ | | $7.0\times10^{-7}$ | $7.0\times10^{6}$ |

Table 4: $\varepsilon = 0.5$, $\Delta t_1 = 3.12 \times 10^{-2}$

| $\ell$ | $\Delta t_\ell$ | $P_\ell$ | $\mathbb{E}[\hat{F}_\ell - \hat{F}_{\ell-1}]$ | $\mathbb{V}[\hat{F}_\ell - \hat{F}_{\ell-1}]$ | $\mathbb{V}[\hat{Y}_\ell]$ | $P_\ell C_\ell$ |
|---|---|---|---|---|---|---|
| 0 | $5.0\times10^{-1}$ | $2.2\times10^{7}$ | $7.78\times10^{-1}$ | $1.2\times10^{0}$ | $5.3\times10^{-8}$ | $4.5\times10^{5}$ |
| 1 | $3.1\times10^{-2}$ | $4.7\times10^{6}$ | $-2.04\times10^{-1}$ | $9.1\times10^{-1}$ | $1.9\times10^{-7}$ | $1.6\times10^{6}$ |
| 2 | $1.6\times10^{-2}$ | $5.0\times10^{5}$ | $-3.90\times10^{-3}$ | $2.8\times10^{-2}$ | $5.7\times10^{-8}$ | $4.8\times10^{5}$ |
| 3 | $7.8\times10^{-3}$ | $2.6\times10^{5}$ | $-9.06\times10^{-4}$ | $1.5\times10^{-2}$ | $5.9\times10^{-8}$ | $4.9\times10^{5}$ |
| 4 | $3.9\times10^{-3}$ | $1.3\times10^{5}$ | $-5.53\times10^{-4}$ | $8.0\times10^{-3}$ | $6.1\times10^{-8}$ | $5.0\times10^{5}$ |
| 5 | $2.0\times10^{-3}$ | $8.4\times10^{4}$ | $8.78\times10^{-5}$ | $3.9\times10^{-3}$ | $4.7\times10^{-8}$ | $6.4\times10^{5}$ |
| 6 | $9.8\times10^{-4}$ | $1.0\times10^{3}$ | $1.12\times10^{-4}$ | $1.6\times10^{-3}$ | $1.6\times10^{-6}$ | $1.5\times10^{4}$ |
| $\sum$ | | | $5.69\times10^{-1}$ | | $2.1\times10^{-6}$ | $4.2\times10^{6}$ |

Table 5: $\varepsilon = 0.5$, $\Delta t_1 = 1.56 \times 10^{-2}$

| $\ell$ | $\Delta t_\ell$ | $P_\ell$ | $\mathbb{E}[\hat{F}_\ell - \hat{F}_{\ell-1}]$ | $\mathbb{V}[\hat{F}_\ell - \hat{F}_{\ell-1}]$ | $\mathbb{V}[\hat{Y}_\ell]$ | $P_\ell C_\ell$ |
|---|---|---|---|---|---|---|
| 0 | $5.0\times10^{-1}$ | $2.3\times10^{7}$ | $7.77\times10^{-1}$ | $1.2\times10^{0}$ | $5.2\times10^{-8}$ | $4.6\times10^{5}$ |
| 1 | $1.6\times10^{-2}$ | $3.8\times10^{6}$ | $-2.09\times10^{-1}$ | $1.1\times10^{0}$ | $2.8\times10^{-7}$ | $2.5\times10^{6}$ |
| 2 | $7.8\times10^{-3}$ | $2.6\times10^{5}$ | $-1.25\times10^{-3}$ | $1.5\times10^{-2}$ | $5.7\times10^{-8}$ | $5.0\times10^{5}$ |
| 3 | $3.9\times10^{-3}$ | $1.3\times10^{5}$ | $-2.42\times10^{-4}$ | $7.9\times10^{-3}$ | $5.9\times10^{-8}$ | $5.2\times10^{5}$ |
| 4 | $2.0\times10^{-3}$ | $5.6\times10^{4}$ | $1.99\times10^{-4}$ | $4.0\times10^{-3}$ | $7.2\times10^{-8}$ | $4.3\times10^{5}$ |
| 5 | $9.8\times10^{-4}$ | $1.0\times10^{3}$ | $9.38\times10^{-5}$ | $1.6\times10^{-3}$ | $1.6\times10^{-6}$ | $1.5\times10^{4}$ |
| $\sum$ | | | $5.67\times10^{-1}$ | | $2.1\times10^{-6}$ | $4.4\times10^{6}$ |

Table 6: $\varepsilon = 0.5$, $\Delta t_1 = 7.81 \times 10^{-3}$

| $\ell$ | $\Delta t_\ell$ | $P_\ell$ | $\mathbb{E}[\hat{F}_\ell - \hat{F}_{\ell-1}]$ | $\mathbb{V}[\hat{F}_\ell - \hat{F}_{\ell-1}]$ | $\mathbb{V}[\hat{Y}_\ell]$ | $P_\ell C_\ell$ |
|---|---|---|---|---|---|---|
| 0 | $5.0\times10^{-1}$ | $3.2\times10^{7}$ | $7.78\times10^{-1}$ | $1.2\times10^{0}$ | $3.7\times10^{-8}$ | $6.4\times10^{5}$ |
| 1 | $7.8\times10^{-3}$ | $3.9\times10^{6}$ | $-2.10\times10^{-1}$ | $1.2\times10^{0}$ | $2.9\times10^{-7}$ | $5.1\times10^{6}$ |
| 2 | $3.9\times10^{-3}$ | $1.9\times10^{5}$ | $-4.45\times10^{-4}$ | $7.9\times10^{-3}$ | $4.2\times10^{-8}$ | $7.3\times10^{5}$ |
| 3 | $2.0\times10^{-3}$ | $9.5\times10^{4}$ | $2.36\times10^{-4}$ | $3.9\times10^{-3}$ | $4.1\times10^{-8}$ | $7.3\times10^{5}$ |
| 4 | $9.8\times10^{-4}$ | $4.9\times10^{4}$ | $3.80\times10^{-5}$ | $2.1\times10^{-3}$ | $4.3\times10^{-8}$ | $7.5\times10^{5}$ |
| 5 | $4.9\times10^{-4}$ | $2.5\times10^{4}$ | $5.25\times10^{-6}$ | $1.0\times10^{-3}$ | $4.1\times10^{-8}$ | $7.6\times10^{5}$ |
| 6 | $2.4\times10^{-4}$ | $1.0\times10^{3}$ | $-5.89\times10^{-4}$ | $7.9\times10^{-4}$ | $7.9\times10^{-7}$ | $6.1\times10^{4}$ |
| $\sum$ | | | $5.68\times10^{-1}$ | | $1.3\times10^{-6}$ | $8.8\times10^{6}$ |

Table 7: $\varepsilon = 0.5$, $\Delta t_1 = 3.91 \times 10^{-3}$

| $\ell$ | $\Delta t_\ell$ | $P_\ell$ | $\mathbb{E}[\hat{F}_\ell - \hat{F}_{\ell-1}]$ | $\mathbb{V}[\hat{F}_\ell - \hat{F}_{\ell-1}]$ | $\mathbb{V}[\hat{Y}_\ell]$ | $P_\ell C_\ell$ |
|---|---|---|---|---|---|---|
| 0 | $5.0\times10^{-1}$ | $3.8\times10^{7}$ | $7.78\times10^{-1}$ | $1.2\times10^{0}$ | $3.1\times10^{-8}$ | $7.6\times10^{5}$ |
| 1 | $3.9\times10^{-3}$ | $3.4\times10^{6}$ | $-2.10\times10^{-1}$ | $1.2\times10^{0}$ | $3.6\times10^{-7}$ | $8.7\times10^{6}$ |
| 2 | $2.0\times10^{-3}$ | $1.1\times10^{5}$ | $-2.02\times10^{-5}$ | $4.1\times10^{-3}$ | $3.6\times10^{-8}$ | $8.7\times10^{5}$ |
| 3 | $9.8\times10^{-4}$ | $5.7\times10^{4}$ | $-7.57\times10^{-7}$ | $2.1\times10^{-3}$ | $3.7\times10^{-8}$ | $8.8\times10^{5}$ |
| 4 | $4.9\times10^{-4}$ | $3.1\times10^{4}$ | $-4.33\times10^{-5}$ | $1.2\times10^{-3}$ | $3.8\times10^{-8}$ | $9.4\times10^{5}$ |
| 5 | $2.4\times10^{-4}$ | $1.0\times10^{3}$ | $3.12\times10^{-5}$ | $3.9\times10^{-4}$ | $3.9\times10^{-7}$ | $6.1\times10^{4}$ |
| $\sum$ | | | $5.68\times10^{-1}$ | | $8.9\times10^{-7}$ | $1.2\times10^{7}$ |

Table 8: $\varepsilon = 0.5$, $\Delta t_1 = 1.95 \times 10^{-3}$

| $\ell$ | $\Delta t_\ell$ | $P_\ell$ | $\mathbb{E}[\hat{F}_\ell - \hat{F}_{\ell-1}]$ | $\mathbb{V}[\hat{F}_\ell - \hat{F}_{\ell-1}]$ | $\mathbb{V}[\hat{Y}_\ell]$ | $P_\ell C_\ell$ |
|---|---|---|---|---|---|---|
| 0 | $5.0\times10^{-1}$ | $4.7\times10^{7}$ | $7.78\times10^{-1}$ | $1.2\times10^{0}$ | $2.5\times10^{-8}$ | $9.5\times10^{5}$ |
| 1 | $2.0\times10^{-3}$ | $3.0\times10^{6}$ | $-2.10\times10^{-1}$ | $1.3\times10^{0}$ | $4.1\times10^{-7}$ | $1.6\times10^{7}$ |
| 2 | $9.8\times10^{-4}$ | $8.5\times10^{4}$ | $-3.08\times10^{-5}$ | $2.0\times10^{-3}$ | $2.4\times10^{-8}$ | $1.3\times10^{6}$ |
| 3 | $4.9\times10^{-4}$ | $4.1\times10^{4}$ | $-1.60\times10^{-4}$ | $1.1\times10^{-3}$ | $2.6\times10^{-8}$ | $1.3\times10^{6}$ |
| 4 | $2.4\times10^{-4}$ | $1.0\times10^{3}$ | $-1.54\times10^{-4}$ | $3.8\times10^{-4}$ | $3.8\times10^{-7}$ | $6.1\times10^{4}$ |
| $\sum$ | | | $5.68\times10^{-1}$ | | $8.7\times10^{-7}$ | $1.9\times10^{7}$ |

Table 9: $\varepsilon = 0.5$, $\Delta t_1 = 9.77 \times 10^{-4}$

| $\ell$ | $\Delta t_\ell$ | $P_\ell$ | $\mathbb{E}[\hat{F}_\ell - \hat{F}_{\ell-1}]$ | $\mathbb{V}[\hat{F}_\ell - \hat{F}_{\ell-1}]$ | $\mathbb{V}[\hat{Y}_\ell]$ | $P_\ell C_\ell$ |
|---|---|---|---|---|---|---|
| 0 | $5.0\times10^{-1}$ | $6.3\times10^{7}$ | $7.78\times10^{-1}$ | $1.2\times10^{0}$ | $1.9\times10^{-8}$ | $1.3\times10^{6}$ |
| 1 | $9.8\times10^{-4}$ | $2.9\times10^{6}$ | $-2.11\times10^{-1}$ | $1.3\times10^{0}$ | $4.4\times10^{-7}$ | $3.0\times10^{7}$ |
| 2 | $4.9\times10^{-4}$ | $4.9\times10^{4}$ | $1.35\times10^{-4}$ | $1.0\times10^{-3}$ | $2.1\times10^{-8}$ | $1.5\times10^{6}$ |
| 3 | $2.4\times10^{-4}$ | $2.0\times10^{4}$ | $-1.49\times10^{-4}$ | $4.5\times10^{-4}$ | $2.2\times10^{-8}$ | $1.3\times10^{6}$ |
| 4 | $1.2\times10^{-4}$ | $1.0\times10^{3}$ | $1.83\times10^{-5}$ | $1.9\times10^{-4}$ | $1.9\times10^{-7}$ | $1.2\times10^{5}$ |
| $\sum$ | | | $5.67\times10^{-1}$ | | $6.9\times10^{-7}$ | $3.4\times10^{7}$ |

Table 10: $\varepsilon = 0.5$, $\Delta t_1 = 4.88 \times 10^{-4}$

| $\ell$ | $\Delta t_\ell$ | $P_\ell$ | $\mathbb{E}[\hat{F}_\ell - \hat{F}_{\ell-1}]$ | $\mathbb{V}[\hat{F}_\ell - \hat{F}_{\ell-1}]$ | $\mathbb{V}[\hat{Y}_\ell]$ | $P_\ell C_\ell$ |
|---|---|---|---|---|---|---|
| 0 | $5.0\times10^{-1}$ | $8.7\times10^{7}$ | $7.78\times10^{-1}$ | $1.2\times10^{0}$ | $1.4\times10^{-8}$ | $1.7\times10^{6}$ |
| 1 | $4.9\times10^{-4}$ | $2.8\times10^{6}$ | $-2.09\times10^{-1}$ | $1.3\times10^{0}$ | $4.6\times10^{-7}$ | $5.8\times10^{7}$ |
| 2 | $2.4\times10^{-4}$ | $3.4\times10^{4}$ | $-6.96\times10^{-6}$ | $5.3\times10^{-4}$ | $1.6\times10^{-8}$ | $2.1\times10^{6}$ |
| 3 | $1.2\times10^{-4}$ | $1.4\times10^{4}$ | $-1.13\times10^{-4}$ | $3.1\times10^{-4}$ | $2.2\times10^{-8}$ | $1.7\times10^{6}$ |
| 4 | $6.1\times10^{-5}$ | $1.0\times10^{3}$ | $-9.14\times10^{-5}$ | $8.4\times10^{-5}$ | $8.4\times10^{-8}$ | $2.5\times10^{5}$ |
| $\sum$ | | | $5.69\times10^{-1}$ | | $5.9\times10^{-7}$ | $6.4\times10^{7}$ |

## 1.2 Term-by-term correlation, $\varepsilon = 0.1$

Table 11: $\varepsilon = 0.1$, $\Delta t_1 = 1.00 \times 10^{-2}$

| $\ell$ | $\Delta t_\ell$ | $P_\ell$ | $\mathbb{E}[\hat{F}_\ell - \hat{F}_{\ell-1}]$ | $\mathbb{V}[\hat{F}_\ell - \hat{F}_{\ell-1}]$ | $\mathbb{V}[\hat{Y}_\ell]$ | $P_\ell C_\ell$ |
|---|---|---|---|---|---|---|
| 0 | $5.0\times10^{-1}$ | $6.2\times10^{8}$ | $9.90\times10^{-1}$ | $2.0\times10^{0}$ | $3.1\times10^{-9}$ | $1.2\times10^{7}$ |
| 1 | $1.0\times10^{-2}$ | $7.4\times10^{7}$ | $-1.25\times10^{-1}$ | $1.4\times10^{0}$ | $1.9\times10^{-8}$ | $7.6\times10^{7}$ |
| 2 | $5.0\times10^{-3}$ | $2.4\times10^{7}$ | $1.02\times10^{-2}$ | $4.4\times10^{-1}$ | $1.8\times10^{-8}$ | $7.2\times10^{7}$ |
| 3 | $2.5\times10^{-3}$ | $1.6\times10^{7}$ | $2.86\times10^{-2}$ | $4.0\times10^{-1}$ | $2.5\times10^{-8}$ | $9.8\times10^{7}$ |
| 4 | $1.3\times10^{-3}$ | $1.0\times10^{7}$ | $2.85\times10^{-2}$ | $3.0\times10^{-1}$ | $3.0\times10^{-8}$ | $1.2\times10^{8}$ |
| 5 | $6.3\times10^{-4}$ | $5.7\times10^{6}$ | $2.07\times10^{-2}$ | $2.0\times10^{-1}$ | $3.4\times10^{-8}$ | $1.4\times10^{8}$ |
| 6 | $3.1\times10^{-4}$ | $3.0\times10^{6}$ | $1.22\times10^{-2}$ | $1.1\times10^{-1}$ | $3.7\times10^{-8}$ | $1.5\times10^{8}$ |
| 7 | $1.6\times10^{-4}$ | $1.6\times10^{6}$ | $6.91\times10^{-3}$ | $6.0\times10^{-2}$ | $3.8\times10^{-8}$ | $1.5\times10^{8}$ |
| 8 | $7.8\times10^{-5}$ | $7.9\times10^{5}$ | $3.74\times10^{-3}$ | $3.0\times10^{-2}$ | $3.8\times10^{-8}$ | $1.5\times10^{8}$ |
| 9 | $3.9\times10^{-5}$ | $4.0\times10^{5}$ | $1.70\times10^{-3}$ | $1.5\times10^{-2}$ | $3.8\times10^{-8}$ | $1.5\times10^{8}$ |
| 10 | $2.0\times10^{-5}$ | $2.0\times10^{5}$ | $1.11\times10^{-3}$ | $7.7\times10^{-3}$ | $3.9\times10^{-8}$ | $1.5\times10^{8}$ |
| 11 | $9.8\times10^{-6}$ | $1.0\times10^{5}$ | $9.87\times10^{-4}$ | $4.0\times10^{-3}$ | $3.9\times10^{-8}$ | $1.6\times10^{8}$ |
| 12 | $4.9\times10^{-6}$ | $4.9\times10^{4}$ | $2.43\times10^{-4}$ | $2.0\times10^{-3}$ | $4.1\times10^{-8}$ | $1.5\times10^{8}$ |
| 13 | $2.4\times10^{-6}$ | $2.8\times10^{4}$ | $2.90\times10^{-4}$ | $6.9\times10^{-4}$ | $2.5\times10^{-8}$ | $1.7\times10^{8}$ |
| 14 | $1.2\times10^{-6}$ | $2.2\times10^{4}$ | $8.64\times10^{-5}$ | $4.9\times10^{-4}$ | $2.2\times10^{-8}$ | $2.7\times10^{8}$ |
| 15 | $6.1\times10^{-7}$ | $1.0\times10^{3}$ | $2.04\times10^{-4}$ | $3.9\times10^{-5}$ | $3.9\times10^{-8}$ | $2.5\times10^{7}$ |
| $\sum$ | | | $9.81\times10^{-1}$ | | $4.9\times10^{-7}$ | $2.0\times10^{9}$ |

Table 12: $\varepsilon = 0.1$, $\Delta t_1 = 5.00 \times 10^{-3}$

| $\ell$ | $\Delta t_\ell$ | $P_\ell$ | $\mathbb{E}[\hat{F}_\ell - \hat{F}_{\ell-1}]$ | $\mathbb{V}[\hat{F}_\ell - \hat{F}_{\ell-1}]$ | $\mathbb{V}[\hat{Y}_\ell]$ | $P_\ell C_\ell$ |
|---|---|---|---|---|---|---|
| 0 | $5.0\times10^{-1}$ | $6.2\times10^{8}$ | $9.90\times10^{-1}$ | $2.0\times10^{0}$ | $3.1\times10^{-9}$ | $1.2\times10^{7}$ |
| 1 | $5.0\times10^{-3}$ | $6.4\times10^{7}$ | $-1.14\times10^{-1}$ | $2.1\times10^{0}$ | $3.3\times10^{-8}$ | $1.3\times10^{8}$ |
| 2 | $2.5\times10^{-3}$ | $1.6\times10^{7}$ | $2.84\times10^{-2}$ | $4.0\times10^{-1}$ | $2.5\times10^{-8}$ | $9.8\times10^{7}$ |
| 3 | $1.3\times10^{-3}$ | $1.0\times10^{7}$ | $2.91\times10^{-2}$ | $3.0\times10^{-1}$ | $3.0\times10^{-8}$ | $1.2\times10^{8}$ |
| 4 | $6.3\times10^{-4}$ | $5.7\times10^{6}$ | $2.05\times10^{-2}$ | $1.9\times10^{-1}$ | $3.4\times10^{-8}$ | $1.4\times10^{8}$ |
| 5 | $3.1\times10^{-4}$ | $3.0\times10^{6}$ | $1.21\times10^{-2}$ | $1.1\times10^{-1}$ | $3.7\times10^{-8}$ | $1.5\times10^{8}$ |
| 6 | $1.6\times10^{-4}$ | $1.6\times10^{6}$ | $6.77\times10^{-3}$ | $6.0\times10^{-2}$ | $3.8\times10^{-8}$ | $1.5\times10^{8}$ |
| 7 | $7.8\times10^{-5}$ | $8.0\times10^{5}$ | $3.35\times10^{-3}$ | $3.1\times10^{-2}$ | $3.8\times10^{-8}$ | $1.5\times10^{8}$ |
| 8 | $3.9\times10^{-5}$ | $4.0\times10^{5}$ | $1.91\times10^{-3}$ | $1.6\times10^{-2}$ | $3.9\times10^{-8}$ | $1.5\times10^{8}$ |
| 9 | $2.0\times10^{-5}$ | $2.0\times10^{5}$ | $9.11\times10^{-4}$ | $7.9\times10^{-3}$ | $4.0\times10^{-8}$ | $1.5\times10^{8}$ |
| 10 | $9.8\times10^{-6}$ | $1.4\times10^{5}$ | $2.53\times10^{-4}$ | $4.2\times10^{-3}$ | $3.1\times10^{-8}$ | $2.1\times10^{8}$ |
| 11 | $4.9\times10^{-6}$ | $4.7\times10^{4}$ | $-1.92\times10^{-4}$ | $3.1\times10^{-3}$ | $6.6\times10^{-8}$ | $1.4\times10^{8}$ |
| 12 | $2.4\times10^{-6}$ | $7.0\times10^{4}$ | $-2.45\times10^{-5}$ | $1.3\times10^{-3}$ | $1.9\times10^{-8}$ | $4.3\times10^{8}$ |
| 13 | $1.2\times10^{-6}$ | $1.0\times10^{3}$ | $1.84\times10^{-4}$ | $1.7\times10^{-4}$ | $1.7\times10^{-7}$ | $1.2\times10^{7}$ |
| $\sum$ | | | $9.79\times10^{-1}$ | | $6.0\times10^{-7}$ | $2.1\times10^{9}$ |

Table 13: $\varepsilon = 0.1$, $\Delta t_1 = 2.50 \times 10^{-3}$

| $\ell$ | $\Delta t_\ell$ | $P_\ell$ | $\mathbb{E}[\hat{F}_\ell - \hat{F}_{\ell-1}]$ | $\mathbb{V}[\hat{F}_\ell - \hat{F}_{\ell-1}]$ | $\mathbb{V}[\hat{Y}_\ell]$ | $P_\ell C_\ell$ |
|---|---|---|---|---|---|---|
| 0 | $5.0\times10^{-1}$ | $4.6\times10^{8}$ | $9.90\times10^{-1}$ | $2.0\times10^{0}$ | $4.2\times10^{-9}$ | $9.2\times10^{6}$ |
| 1 | $2.5\times10^{-3}$ | $3.8\times10^{7}$ | $-8.58\times10^{-2}$ | $2.7\times10^{0}$ | $7.1\times10^{-8}$ | $1.5\times10^{8}$ |
| 2 | $1.3\times10^{-3}$ | $7.4\times10^{6}$ | $2.88\times10^{-2}$ | $3.0\times10^{-1}$ | $4.1\times10^{-8}$ | $8.9\times10^{7}$ |
| 3 | $6.3\times10^{-4}$ | $4.2\times10^{6}$ | $2.07\times10^{-2}$ | $2.0\times10^{-1}$ | $4.6\times10^{-8}$ | $1.0\times10^{8}$ |
| 4 | $3.1\times10^{-4}$ | $2.3\times10^{6}$ | $1.24\times10^{-2}$ | $1.1\times10^{-1}$ | $5.0\times10^{-8}$ | $1.1\times10^{8}$ |
| 5 | $1.6\times10^{-4}$ | $1.2\times10^{6}$ | $6.78\times10^{-3}$ | $6.0\times10^{-2}$ | $5.1\times10^{-8}$ | $1.1\times10^{8}$ |
| 6 | $7.8\times10^{-5}$ | $5.9\times10^{5}$ | $3.71\times10^{-3}$ | $3.0\times10^{-2}$ | $5.2\times10^{-8}$ | $1.1\times10^{8}$ |
| 7 | $3.9\times10^{-5}$ | $2.9\times10^{5}$ | $1.60\times10^{-3}$ | $1.5\times10^{-2}$ | $5.2\times10^{-8}$ | $1.1\times10^{8}$ |
| 8 | $2.0\times10^{-5}$ | $1.5\times10^{5}$ | $1.22\times10^{-3}$ | $8.4\times10^{-3}$ | $5.5\times10^{-8}$ | $1.2\times10^{8}$ |
| 9 | $9.8\times10^{-6}$ | $7.6\times10^{4}$ | $4.20\times10^{-4}$ | $3.8\times10^{-3}$ | $5.1\times10^{-8}$ | $1.2\times10^{8}$ |
| 10 | $4.9\times10^{-6}$ | $1.9\times10^{4}$ | $7.61\times10^{-5}$ | $2.1\times10^{-3}$ | $1.1\times10^{-7}$ | $5.9\times10^{7}$ |
| 11 | $2.4\times10^{-6}$ | $1.0\times10^{3}$ | $-7.71\times10^{-5}$ | $2.2\times10^{-4}$ | $2.2\times10^{-7}$ | $6.1\times10^{6}$ |
| $\sum$ | | | $9.80\times10^{-1}$ | | $8.0\times10^{-7}$ | $1.1\times10^{9}$ |

Table 14: $\varepsilon = 0.1$, $\Delta t_1 = 1.25 \times 10^{-3}$

| $\ell$ | $\Delta t_\ell$ | $P_\ell$ | $\mathbb{E}[\hat{F}_\ell - \hat{F}_{\ell-1}]$ | $\mathbb{V}[\hat{F}_\ell - \hat{F}_{\ell-1}]$ | $\mathbb{V}[\hat{Y}_\ell]$ | $P_\ell C_\ell$ |
|---|---|---|---|---|---|---|
| 0 | $5.0\times10^{-1}$ | $5.5\times10^{8}$ | $9.90\times10^{-1}$ | $2.0\times10^{0}$ | $3.6\times10^{-9}$ | $1.1\times10^{7}$ |
| 1 | $1.3\times10^{-3}$ | $3.5\times10^{7}$ | $-5.69\times10^{-2}$ | $3.2\times10^{0}$ | $9.1\times10^{-8}$ | $2.8\times10^{8}$ |
| 2 | $6.3\times10^{-4}$ | $5.0\times10^{6}$ | $2.04\times10^{-2}$ | $1.9\times10^{-1}$ | $3.9\times10^{-8}$ | $1.2\times10^{8}$ |
| 3 | $3.1\times10^{-4}$ | $2.7\times10^{6}$ | $1.24\times10^{-2}$ | $1.1\times10^{-1}$ | $4.2\times10^{-8}$ | $1.3\times10^{8}$ |
| 4 | $1.6\times10^{-4}$ | $1.4\times10^{6}$ | $6.57\times10^{-3}$ | $6.0\times10^{-2}$ | $4.3\times10^{-8}$ | $1.3\times10^{8}$ |
| 5 | $7.8\times10^{-5}$ | $7.0\times10^{5}$ | $3.08\times10^{-3}$ | $3.1\times10^{-2}$ | $4.4\times10^{-8}$ | $1.4\times10^{8}$ |
| 6 | $3.9\times10^{-5}$ | $3.5\times10^{5}$ | $1.91\times10^{-3}$ | $1.6\times10^{-2}$ | $4.5\times10^{-8}$ | $1.4\times10^{8}$ |
| 7 | $2.0\times10^{-5}$ | $1.8\times10^{5}$ | $7.11\times10^{-4}$ | $7.9\times10^{-3}$ | $4.4\times10^{-8}$ | $1.4\times10^{8}$ |
| 8 | $9.8\times10^{-6}$ | $1.3\times10^{5}$ | $3.20\times10^{-4}$ | $3.7\times10^{-3}$ | $2.8\times10^{-8}$ | $2.0\times10^{8}$ |
| 9 | $4.9\times10^{-6}$ | $6.0\times10^{4}$ | $-1.48\times10^{-4}$ | $2.2\times10^{-3}$ | $3.6\times10^{-8}$ | $1.8\times10^{8}$ |
| 10 | $2.4\times10^{-6}$ | $2.8\times10^{4}$ | $2.68\times10^{-4}$ | $1.3\times10^{-3}$ | $4.5\times10^{-8}$ | $1.7\times10^{8}$ |
| 11 | $1.2\times10^{-6}$ | $1.0\times10^{3}$ | $-1.46\times10^{-5}$ | $8.2\times10^{-5}$ | $8.2\times10^{-8}$ | $1.2\times10^{7}$ |
| $\sum$ | | | $9.78\times10^{-1}$ | | $5.4\times10^{-7}$ | $1.7\times10^{9}$ |

Table 15: $\varepsilon = 0.1$, $\Delta t_1 = 6.25 \times 10^{-4}$

| $\ell$ | $\Delta t_\ell$ | $P_\ell$ | $\mathbb{E}[\hat{F}_\ell - \hat{F}_{\ell-1}]$ | $\mathbb{V}[\hat{F}_\ell - \hat{F}_{\ell-1}]$ | $\mathbb{V}[\hat{Y}_\ell]$ | $P_\ell C_\ell$ |
|---|---|---|---|---|---|---|
| 0 | $5.0\times10^{-1}$ | $4.7\times10^{8}$ | $9.90\times10^{-1}$ | $2.0\times10^{0}$ | $4.2\times10^{-9}$ | $9.3\times10^{6}$ |
| 1 | $6.3\times10^{-4}$ | $2.2\times10^{7}$ | $-3.67\times10^{-2}$ | $3.4\times10^{0}$ | $1.6\times10^{-7}$ | $3.5\times10^{8}$ |
| 2 | $3.1\times10^{-4}$ | $2.3\times10^{6}$ | $1.23\times10^{-2}$ | $1.1\times10^{-1}$ | $4.9\times10^{-8}$ | $1.1\times10^{8}$ |
| 3 | $1.6\times10^{-4}$ | $1.2\times10^{6}$ | $6.51\times10^{-3}$ | $5.9\times10^{-2}$ | $5.1\times10^{-8}$ | $1.1\times10^{8}$ |
| 4 | $7.8\times10^{-5}$ | $6.0\times10^{5}$ | $3.73\times10^{-3}$ | $3.1\times10^{-2}$ | $5.2\times10^{-8}$ | $1.1\times10^{8}$ |
| 5 | $3.9\times10^{-5}$ | $3.0\times10^{5}$ | $1.78\times10^{-3}$ | $1.6\times10^{-2}$ | $5.2\times10^{-8}$ | $1.2\times10^{8}$ |
| 6 | $2.0\times10^{-5}$ | $1.6\times10^{5}$ | $7.40\times10^{-4}$ | $8.5\times10^{-3}$ | $5.4\times10^{-8}$ | $1.2\times10^{8}$ |
| 7 | $9.8\times10^{-6}$ | $7.8\times10^{4}$ | $4.22\times10^{-4}$ | $3.8\times10^{-3}$ | $4.8\times10^{-8}$ | $1.2\times10^{8}$ |
| 8 | $4.9\times10^{-6}$ | $2.0\times10^{4}$ | $4.12\times10^{-4}$ | $1.9\times10^{-3}$ | $9.3\times10^{-8}$ | $6.2\times10^{7}$ |
| 9 | $2.4\times10^{-6}$ | $1.0\times10^{3}$ | $1.55\times10^{-4}$ | $1.5\times10^{-4}$ | $1.5\times10^{-7}$ | $6.1\times10^{6}$ |
| $\sum$ | | | $9.79\times10^{-1}$ | | $7.2\times10^{-7}$ | $1.1\times10^{9}$ |

Table 16: $\varepsilon = 0.1$, $\Delta t_1 = 3.13 \times 10^{-4}$

| $\ell$ | $\Delta t_\ell$ | $P_\ell$ | $\mathbb{E}[\hat{F}_\ell - \hat{F}_{\ell-1}]$ | $\mathbb{V}[\hat{F}_\ell - \hat{F}_{\ell-1}]$ | $\mathbb{V}[\hat{Y}_\ell]$ | $P_\ell C_\ell$ |
|---|---|---|---|---|---|---|
| 0 | $5.0\times10^{-1}$ | $5.6\times10^{8}$ | $9.90\times10^{-1}$ | $2.0\times10^{0}$ | $3.5\times10^{-9}$ | $1.1\times10^{7}$ |
| 1 | $3.1\times10^{-4}$ | $1.9\times10^{7}$ | $-2.40\times10^{-2}$ | $3.6\times10^{0}$ | $1.9\times10^{-7}$ | $6.0\times10^{8}$ |
| 2 | $1.6\times10^{-4}$ | $1.4\times10^{6}$ | $6.93\times10^{-3}$ | $6.0\times10^{-2}$ | $4.3\times10^{-8}$ | $1.3\times10^{8}$ |
| 3 | $7.8\times10^{-5}$ | $7.3\times10^{5}$ | $3.20\times10^{-3}$ | $3.2\times10^{-2}$ | $4.4\times10^{-8}$ | $1.4\times10^{8}$ |
| 4 | $3.9\times10^{-5}$ | $3.6\times10^{5}$ | $1.56\times10^{-3}$ | $1.6\times10^{-2}$ | $4.4\times10^{-8}$ | $1.4\times10^{8}$ |
| 5 | $2.0\times10^{-5}$ | $1.8\times10^{5}$ | $6.85\times10^{-4}$ | $7.7\times10^{-3}$ | $4.3\times10^{-8}$ | $1.4\times10^{8}$ |
| 6 | $9.8\times10^{-6}$ | $8.7\times10^{4}$ | $3.70\times10^{-4}$ | $3.7\times10^{-3}$ | $4.2\times10^{-8}$ | $1.3\times10^{8}$ |
| 7 | $4.9\times10^{-6}$ | $4.8\times10^{4}$ | $-1.71\times10^{-4}$ | $2.2\times10^{-3}$ | $4.6\times10^{-8}$ | $1.5\times10^{8}$ |
| 8 | $2.4\times10^{-6}$ | $2.2\times10^{4}$ | $-1.42\times10^{-4}$ | $9.1\times10^{-4}$ | $4.1\times10^{-8}$ | $1.4\times10^{8}$ |
| 9 | $1.2\times10^{-6}$ | $1.0\times10^{3}$ | $3.43\times10^{-4}$ | $8.9\times10^{-5}$ | $8.9\times10^{-8}$ | $1.2\times10^{7}$ |
| $\sum$ | | | $9.79\times10^{-1}$ | | $5.8\times10^{-7}$ | $1.6\times10^{9}$ |

Table 17: $\varepsilon = 0.1$, $\Delta t_1 = 1.56 \times 10^{-4}$

| $\ell$ | $\Delta t_\ell$ | $P_\ell$ | $\mathbb{E}[\hat{F}_\ell - \hat{F}_{\ell-1}]$ | $\mathbb{V}[\hat{F}_\ell - \hat{F}_{\ell-1}]$ | $\mathbb{V}[\hat{Y}_\ell]$ | $P_\ell C_\ell$ |
|---|---|---|---|---|---|---|
| 0 | $5.0\times10^{-1}$ | $6.5\times10^{8}$ | $9.90\times10^{-1}$ | $2.0\times10^{0}$ | $3.0\times10^{-9}$ | $1.3\times10^{7}$ |
| 1 | $1.6\times10^{-4}$ | $1.6\times10^{7}$ | $-1.72\times10^{-2}$ | $3.7\times10^{0}$ | $2.3\times10^{-7}$ | $1.0\times10^{9}$ |
| 2 | $7.8\times10^{-5}$ | $8.4\times10^{5}$ | $3.48\times10^{-3}$ | $3.2\times10^{-2}$ | $3.8\times10^{-8}$ | $1.6\times10^{8}$ |
| 3 | $3.9\times10^{-5}$ | $4.2\times10^{5}$ | $1.65\times10^{-3}$ | $1.6\times10^{-2}$ | $3.7\times10^{-8}$ | $1.6\times10^{8}$ |
| 4 | $2.0\times10^{-5}$ | $2.1\times10^{5}$ | $1.00\times10^{-3}$ | $7.7\times10^{-3}$ | $3.7\times10^{-8}$ | $1.6\times10^{8}$ |
| 5 | $9.8\times10^{-6}$ | $2.5\times10^{5}$ | $6.06\times10^{-4}$ | $4.2\times10^{-3}$ | $1.7\times10^{-8}$ | $3.8\times10^{8}$ |
| 6 | $4.9\times10^{-6}$ | $5.5\times10^{4}$ | $3.18\times10^{-4}$ | $1.8\times10^{-3}$ | $3.3\times10^{-8}$ | $1.7\times10^{8}$ |
| 7 | $2.4\times10^{-6}$ | $5.1\times10^{4}$ | $1.64\times10^{-4}$ | $7.0\times10^{-4}$ | $1.4\times10^{-8}$ | $3.2\times10^{8}$ |
| 8 | $1.2\times10^{-6}$ | $1.0\times10^{3}$ | $1.93\times10^{-4}$ | $7.5\times10^{-5}$ | $7.5\times10^{-8}$ | $1.2\times10^{7}$ |
| $\sum$ | | | $9.80\times10^{-1}$ | | $4.9\times10^{-7}$ | $2.4\times10^{9}$ |

Table 18: $\varepsilon = 0.1$, $\Delta t_1 = 7.81 \times 10^{-5}$

| $\ell$ | $\Delta t_\ell$ | $P_\ell$ | $\mathbb{E}[\hat{F}_\ell - \hat{F}_{\ell-1}]$ | $\mathbb{V}[\hat{F}_\ell - \hat{F}_{\ell-1}]$ | $\mathbb{V}[\hat{Y}_\ell]$ | $P_\ell C_\ell$ |
|---|---|---|---|---|---|---|
| 0 | $5.0\times10^{-1}$ | $7.2\times10^{8}$ | $9.90\times10^{-1}$ | $2.0\times10^{0}$ | $2.7\times10^{-9}$ | $1.4\times10^{7}$ |
| 1 | $7.8\times10^{-5}$ | $1.2\times10^{7}$ | $-1.51\times10^{-2}$ | $3.7\times10^{0}$ | $3.0\times10^{-7}$ | $1.6\times10^{9}$ |
| 2 | $3.9\times10^{-5}$ | $4.7\times10^{5}$ | $2.06\times10^{-3}$ | $1.6\times10^{-2}$ | $3.4\times10^{-8}$ | $1.8\times10^{8}$ |
| 3 | $2.0\times10^{-5}$ | $2.3\times10^{5}$ | $9.88\times10^{-4}$ | $7.9\times10^{-3}$ | $3.4\times10^{-8}$ | $1.8\times10^{8}$ |
| 4 | $9.8\times10^{-6}$ | $1.2\times10^{5}$ | $1.74\times10^{-4}$ | $3.4\times10^{-3}$ | $2.9\times10^{-8}$ | $1.8\times10^{8}$ |
| 5 | $4.9\times10^{-6}$ | $5.7\times10^{4}$ | $1.80\times10^{-4}$ | $1.9\times10^{-3}$ | $3.4\times10^{-8}$ | $1.8\times10^{8}$ |
| 6 | $2.4\times10^{-6}$ | $5.3\times10^{4}$ | $-1.66\times10^{-5}$ | $1.6\times10^{-3}$ | $3.0\times10^{-8}$ | $3.2\times10^{8}$ |
| 7 | $1.2\times10^{-6}$ | $1.0\times10^{3}$ | $-1.21\times10^{-4}$ | $8.4\times10^{-5}$ | $8.4\times10^{-8}$ | $1.2\times10^{7}$ |
| $\sum$ | | | $9.78\times10^{-1}$ | | $5.5\times10^{-7}$ | $2.6\times10^{9}$ |

Table 19: $\varepsilon = 0.1$, $\Delta t_1 = 3.91 \times 10^{-5}$

| $\ell$ | $\Delta t_\ell$ | $P_\ell$ | $\mathbb{E}[\hat{F}_\ell - \hat{F}_{\ell-1}]$ | $\mathbb{V}[\hat{F}_\ell - \hat{F}_{\ell-1}]$ | $\mathbb{V}[\hat{Y}_\ell]$ | $P_\ell C_\ell$ |
|---|---|---|---|---|---|---|
| 0 | $5.0\times10^{-1}$ | $7.4\times10^{8}$ | $9.90\times10^{-1}$ | $2.0\times10^{0}$ | $2.6\times10^{-9}$ | $1.5\times10^{7}$ |
| 1 | $3.9\times10^{-5}$ | $9.0\times10^{6}$ | $-1.17\times10^{-2}$ | $3.7\times10^{0}$ | $4.1\times10^{-7}$ | $2.3\times10^{9}$ |
| 2 | $2.0\times10^{-5}$ | $2.5\times10^{5}$ | $9.66\times10^{-4}$ | $8.6\times10^{-3}$ | $3.4\times10^{-8}$ | $1.9\times10^{8}$ |
| 3 | $9.8\times10^{-6}$ | $1.2\times10^{5}$ | $2.84\times10^{-4}$ | $4.1\times10^{-3}$ | $3.3\times10^{-8}$ | $1.9\times10^{8}$ |
| 4 | $4.9\times10^{-6}$ | $2.8\times10^{4}$ | $-3.18\times10^{-4}$ | $2.0\times10^{-3}$ | $6.9\times10^{-8}$ | $8.7\times10^{7}$ |
| 5 | $2.4\times10^{-6}$ | $1.0\times10^{3}$ | $-2.51\times10^{-4}$ | $7.6\times10^{-4}$ | $7.6\times10^{-7}$ | $6.1\times10^{6}$ |
| $\sum$ | | | $9.79\times10^{-1}$ | | $1.3\times10^{-6}$ | $2.8\times10^{9}$ |

Table 20: $\varepsilon = 0.1$, $\Delta t_1 = 1.95 \times 10^{-5}$

| $\ell$ | $\Delta t_\ell$ | $P_\ell$ | $\mathbb{E}[\hat{F}_\ell - \hat{F}_{\ell-1}]$ | $\mathbb{V}[\hat{F}_\ell - \hat{F}_{\ell-1}]$ | $\mathbb{V}[\hat{Y}_\ell]$ | $P_\ell C_\ell$ |
|---|---|---|---|---|---|---|
| 0 | $5.0\times10^{-1}$ | $1.0\times10^{9}$ | $9.90\times10^{-1}$ | $2.0\times10^{0}$ | $1.9\times10^{-9}$ | $2.0\times10^{7}$ |
| 1 | $2.0\times10^{-5}$ | $8.8\times10^{6}$ | $-1.14\times10^{-2}$ | $3.8\times10^{0}$ | $4.3\times10^{-7}$ | $4.5\times10^{9}$ |
| 2 | $9.8\times10^{-6}$ | $1.7\times10^{5}$ | $5.83\times10^{-4}$ | $4.3\times10^{-3}$ | $2.5\times10^{-8}$ | $2.6\times10^{8}$ |
| 3 | $4.9\times10^{-6}$ | $1.5\times10^{5}$ | $1.59\times10^{-4}$ | $2.0\times10^{-3}$ | $1.3\times10^{-8}$ | $4.8\times10^{8}$ |
| 4 | $2.4\times10^{-6}$ | $1.0\times10^{3}$ | $2.74\times10^{-4}$ | $5.3\times10^{-4}$ | $5.3\times10^{-7}$ | $6.1\times10^{6}$ |
| $\sum$ | | | $9.80\times10^{-1}$ | | $1.0\times10^{-6}$ | $5.3\times10^{9}$ |

## 1.3 Term-by-term correlation, $\varepsilon = 0.05$

Table 21: $\varepsilon = 0.05$, $\Delta t_1 = 2.50 \times 10^{-3}$

| $\ell$ | $\Delta t_\ell$ | $P_\ell$ | $\mathbb{E}[\hat{F}_\ell - \hat{F}_{\ell-1}]$ | $\mathbb{V}[\hat{F}_\ell - \hat{F}_{\ell-1}]$ | $\mathbb{V}[\hat{Y}_\ell]$ | $P_\ell C_\ell$ |
|---|---|---|---|---|---|---|
| 0 | $5.0\times10^{-1}$ | $2.2\times10^{8}$ | $1.63\times10^{0}$ | $5.2\times10^{0}$ | $2.4\times10^{-8}$ | $4.4\times10^{6}$ |
| 1 | $2.5\times10^{-3}$ | $1.6\times10^{7}$ | $-1.25\times10^{-1}$ | $6.5\times10^{0}$ | $4.0\times10^{-7}$ | $8.4\times10^{7}$ |
| 2 | $1.3\times10^{-3}$ | $1.5\times10^{5}$ | $-1.60\times10^{-5}$ | $1.9\times10^{-3}$ | $1.3\times10^{-8}$ | $2.3\times10^{6}$ |
| 3 | $6.3\times10^{-4}$ | $7.9\times10^{4}$ | $-4.15\times10^{-5}$ | $1.0\times10^{-3}$ | $1.3\times10^{-8}$ | $2.4\times10^{6}$ |
| 4 | $3.1\times10^{-4}$ | $4.1\times10^{4}$ | $1.03\times10^{-5}$ | $5.5\times10^{-4}$ | $1.4\times10^{-8}$ | $2.5\times10^{6}$ |
| 5 | $1.6\times10^{-4}$ | $1.6\times10^{4}$ | $1.02\times10^{-4}$ | $1.9\times10^{-4}$ | $1.2\times10^{-8}$ | $2.0\times10^{6}$ |
| 6 | $7.8\times10^{-5}$ | $1.0\times10^{3}$ | $-2.09\times10^{-4}$ | $9.7\times10^{-5}$ | $9.7\times10^{-8}$ | $2.5\times10^{5}$ |
| $\sum$ | | | $1.50\times10^{0}$ | | $5.7\times10^{-7}$ | $9.8\times10^{7}$ |

Table 22: $\varepsilon = 0.05$, $\Delta t_1 = 1.25 \times 10^{-3}$

| $\ell$ | $\Delta t_\ell$ | $P_\ell$ | $\mathbb{E}[\hat{F}_\ell - \hat{F}_{\ell-1}]$ | $\mathbb{V}[\hat{F}_\ell - \hat{F}_{\ell-1}]$ | $\mathbb{V}[\hat{Y}_\ell]$ | $P_\ell C_\ell$ |
|---|---|---|---|---|---|---|
| 0 | $5.0\times10^{-1}$ | $1.2\times10^{9}$ | $9.97\times10^{-1}$ | $2.0\times10^{0}$ | $1.7\times10^{-9}$ | $2.4\times10^{7}$ |
| 1 | $1.3\times10^{-3}$ | $6.2\times10^{7}$ | $-1.12\times10^{-1}$ | $2.2\times10^{0}$ | $3.5\times10^{-8}$ | $5.0\times10^{8}$ |
| 2 | $6.3\times10^{-4}$ | $1.6\times10^{7}$ | $3.08\times10^{-2}$ | $4.4\times10^{-1}$ | $2.7\times10^{-8}$ | $3.9\times10^{8}$ |
| 3 | $3.1\times10^{-4}$ | $9.9\times10^{6}$ | $3.00\times10^{-2}$ | $3.3\times10^{-1}$ | $3.3\times10^{-8}$ | $4.7\times10^{8}$ |
| 4 | $1.6\times10^{-4}$ | $5.6\times10^{6}$ | $2.10\times10^{-2}$ | $2.1\times10^{-1}$ | $3.8\times10^{-8}$ | $5.4\times10^{8}$ |
| 5 | $7.8\times10^{-5}$ | $3.0\times10^{6}$ | $1.28\times10^{-2}$ | $1.2\times10^{-1}$ | $4.1\times10^{-8}$ | $5.8\times10^{8}$ |
| 6 | $3.9\times10^{-5}$ | $1.6\times10^{6}$ | $7.06\times10^{-3}$ | $6.5\times10^{-2}$ | $4.2\times10^{-8}$ | $6.0\times10^{8}$ |
| 7 | $2.0\times10^{-5}$ | $8.0\times10^{5}$ | $3.84\times10^{-3}$ | $3.4\times10^{-2}$ | $4.3\times10^{-8}$ | $6.1\times10^{8}$ |
| 8 | $9.8\times10^{-6}$ | $4.0\times10^{5}$ | $2.09\times10^{-3}$ | $1.7\times10^{-2}$ | $4.3\times10^{-8}$ | $6.1\times10^{8}$ |
| 9 | $4.9\times10^{-6}$ | $2.1\times10^{5}$ | $8.38\times10^{-4}$ | $9.0\times10^{-3}$ | $4.4\times10^{-8}$ | $6.3\times10^{8}$ |
| 10 | $2.4\times10^{-6}$ | $1.0\times10^{5}$ | $5.47\times10^{-4}$ | $4.8\times10^{-3}$ | $4.6\times10^{-8}$ | $6.4\times10^{8}$ |
| 11 | $1.2\times10^{-6}$ | $4.9\times10^{4}$ | $2.40\times10^{-4}$ | $2.2\times10^{-3}$ | $4.4\times10^{-8}$ | $6.0\times10^{8}$ |
| 12 | $6.1\times10^{-7}$ | $3.6\times10^{4}$ | $2.46\times10^{-4}$ | $9.9\times10^{-4}$ | $2.7\times10^{-8}$ | $8.9\times10^{8}$ |
| 13 | $3.1\times10^{-7}$ | $1.0\times10^{3}$ | $5.30\times10^{-4}$ | $1.3\times10^{-4}$ | $1.3\times10^{-7}$ | $4.9\times10^{7}$ |
| $\sum$ | | | $9.95\times10^{-1}$ | | $5.9\times10^{-7}$ | $7.1\times10^{9}$ |

Table 23: $\varepsilon = 0.05$, $\Delta t_1 = 6.25 \times 10^{-4}$

| $\ell$ | $\Delta t_\ell$ | $P_\ell$ | $\mathbb{E}[\hat{F}_\ell - \hat{F}_{\ell-1}]$ | $\mathbb{V}[\hat{F}_\ell - \hat{F}_{\ell-1}]$ | $\mathbb{V}[\hat{Y}_\ell]$ | $P_\ell C_\ell$ |
|---|---|---|---|---|---|---|
| 0 | $5.0\times10^{-1}$ | $9.9\times10^{8}$ | $9.97\times10^{-1}$ | $2.0\times10^{0}$ | $2.0\times10^{-9}$ | $2.0\times10^{7}$ |
| 1 | $6.3\times10^{-4}$ | $4.2\times10^{7}$ | $-8.12\times10^{-2}$ | $2.8\times10^{0}$ | $6.8\times10^{-8}$ | $6.7\times10^{8}$ |
| 2 | $3.1\times10^{-4}$ | $8.2\times10^{6}$ | $3.04\times10^{-2}$ | $3.3\times10^{-1}$ | $4.0\times10^{-8}$ | $3.9\times10^{8}$ |
| 3 | $1.6\times10^{-4}$ | $4.7\times10^{6}$ | $2.16\times10^{-2}$ | $2.1\times10^{-1}$ | $4.6\times10^{-8}$ | $4.5\times10^{8}$ |
| 4 | $7.8\times10^{-5}$ | $2.5\times10^{6}$ | $1.27\times10^{-2}$ | $1.2\times10^{-1}$ | $4.9\times10^{-8}$ | $4.8\times10^{8}$ |
| 5 | $3.9\times10^{-5}$ | $1.3\times10^{6}$ | $7.18\times10^{-3}$ | $6.6\times10^{-2}$ | $5.1\times10^{-8}$ | $5.0\times10^{8}$ |
| 6 | $2.0\times10^{-5}$ | $6.6\times10^{5}$ | $3.93\times10^{-3}$ | $3.4\times10^{-2}$ | $5.1\times10^{-8}$ | $5.0\times10^{8}$ |
| 7 | $9.8\times10^{-6}$ | $3.3\times10^{5}$ | $1.78\times10^{-3}$ | $1.7\times10^{-2}$ | $5.2\times10^{-8}$ | $5.1\times10^{8}$ |
| 8 | $4.9\times10^{-6}$ | $1.7\times10^{5}$ | $8.71\times10^{-4}$ | $8.6\times10^{-3}$ | $5.2\times10^{-8}$ | $5.1\times10^{8}$ |
| 9 | $2.4\times10^{-6}$ | $8.5\times10^{4}$ | $4.77\times10^{-4}$ | $4.3\times10^{-3}$ | $5.0\times10^{-8}$ | $5.2\times10^{8}$ |
| 10 | $1.2\times10^{-6}$ | $2.9\times10^{4}$ | $2.92\times10^{-4}$ | $2.3\times10^{-3}$ | $7.8\times10^{-8}$ | $3.6\times10^{8}$ |
| 11 | $6.1\times10^{-7}$ | $1.0\times10^{3}$ | $4.73\times10^{-4}$ | $6.6\times10^{-4}$ | $6.6\times10^{-7}$ | $2.5\times10^{7}$ |
| $\sum$ | | | $9.96\times10^{-1}$ | | $1.2\times10^{-6}$ | $4.9\times10^{9}$ |

Table 24: $\varepsilon = 0.05$, $\Delta t_1 = 3.13 \times 10^{-4}$

| $\ell$ | $\Delta t_\ell$ | $P_\ell$ | $\mathbb{E}[\hat{F}_\ell - \hat{F}_{\ell-1}]$ | $\mathbb{V}[\hat{F}_\ell - \hat{F}_{\ell-1}]$ | $\mathbb{V}[\hat{Y}_\ell]$ | $P_\ell C_\ell$ |
|---|---|---|---|---|---|---|
| 0 | $5.0\times10^{-1}$ | $1.2\times10^{9}$ | $9.98\times10^{-1}$ | $2.0\times10^{0}$ | $1.6\times10^{-9}$ | $2.5\times10^{7}$ |
| 1 | $3.1\times10^{-4}$ | $4.0\times10^{7}$ | $-5.14\times10^{-2}$ | $3.3\times10^{0}$ | $8.3\times10^{-8}$ | $1.3\times10^{9}$ |
| 2 | $1.6\times10^{-4}$ | $5.8\times10^{6}$ | $2.16\times10^{-2}$ | $2.1\times10^{-1}$ | $3.7\times10^{-8}$ | $5.6\times10^{8}$ |
| 3 | $7.8\times10^{-5}$ | $3.1\times10^{6}$ | $1.25\times10^{-2}$ | $1.2\times10^{-1}$ | $3.9\times10^{-8}$ | $6.0\times10^{8}$ |
| 4 | $3.9\times10^{-5}$ | $1.6\times10^{6}$ | $7.18\times10^{-3}$ | $6.6\times10^{-2}$ | $4.1\times10^{-8}$ | $6.2\times10^{8}$ |
| 5 | $2.0\times10^{-5}$ | $8.3\times10^{5}$ | $3.64\times10^{-3}$ | $3.4\times10^{-2}$ | $4.2\times10^{-8}$ | $6.4\times10^{8}$ |
| 6 | $9.8\times10^{-6}$ | $4.2\times10^{5}$ | $1.84\times10^{-3}$ | $1.8\times10^{-2}$ | $4.2\times10^{-8}$ | $6.5\times10^{8}$ |
| 7 | $4.9\times10^{-6}$ | $2.1\times10^{5}$ | $7.32\times10^{-4}$ | $8.8\times10^{-3}$ | $4.2\times10^{-8}$ | $6.5\times10^{8}$ |
| 8 | $2.4\times10^{-6}$ | $1.1\times10^{5}$ | $2.67\times10^{-4}$ | $4.6\times10^{-3}$ | $4.3\times10^{-8}$ | $6.6\times10^{8}$ |
| 9 | $1.2\times10^{-6}$ | $5.1\times10^{4}$ | $7.04\times10^{-5}$ | $2.7\times10^{-3}$ | $5.2\times10^{-8}$ | $6.3\times10^{8}$ |
| 10 | $6.1\times10^{-7}$ | $2.7\times10^{4}$ | $-1.83\times10^{-4}$ | $1.3\times10^{-3}$ | $4.6\times10^{-8}$ | $6.7\times10^{8}$ |
| 11 | $3.1\times10^{-7}$ | $1.4\times10^{4}$ | $1.43\times10^{-4}$ | $5.7\times10^{-4}$ | $4.2\times10^{-8}$ | $6.7\times10^{8}$ |
| 12 | $1.5\times10^{-7}$ | $1.0\times10^{3}$ | $-1.16\times10^{-4}$ | $5.2\times10^{-5}$ | $5.2\times10^{-8}$ | $9.8\times10^{7}$ |
| $\sum$ | | | $9.94\times10^{-1}$ | | $5.6\times10^{-7}$ | $7.7\times10^{9}$ |

Table 25: $\varepsilon = 0.05$, $\Delta t_1 = 1.56 \times 10^{-4}$

| $\ell$ | $\Delta t_\ell$ | $P_\ell$ | $\mathbb{E}[\hat{F}_\ell - \hat{F}_{\ell-1}]$ | $\mathbb{V}[\hat{F}_\ell - \hat{F}_{\ell-1}]$ | $\mathbb{V}[\hat{Y}_\ell]$ | $P_\ell C_\ell$ |
|---|---|---|---|---|---|---|
| 0 | $5.0\times10^{-1}$ | $1.1\times10^{9}$ | $9.98\times10^{-1}$ | $2.0\times10^{0}$ | $1.9\times10^{-9}$ | $2.2\times10^{7}$ |
| 1 | $1.6\times10^{-4}$ | $2.6\times10^{7}$ | $-2.94\times10^{-2}$ | $3.6\times10^{0}$ | $1.4\times10^{-7}$ | $1.6\times10^{9}$ |
| 2 | $7.8\times10^{-5}$ | $2.7\times10^{6}$ | $1.29\times10^{-2}$ | $1.2\times10^{-1}$ | $4.5\times10^{-8}$ | $5.2\times10^{8}$ |
| 3 | $3.9\times10^{-5}$ | $1.4\times10^{6}$ | $7.13\times10^{-3}$ | $6.6\times10^{-2}$ | $4.7\times10^{-8}$ | $5.4\times10^{8}$ |
| 4 | $2.0\times10^{-5}$ | $7.2\times10^{5}$ | $3.91\times10^{-3}$ | $3.4\times10^{-2}$ | $4.8\times10^{-8}$ | $5.5\times10^{8}$ |
| 5 | $9.8\times10^{-6}$ | $3.6\times10^{5}$ | $2.36\times10^{-3}$ | $1.8\times10^{-2}$ | $4.8\times10^{-8}$ | $5.6\times10^{8}$ |
| 6 | $4.9\times10^{-6}$ | $1.9\times10^{5}$ | $1.03\times10^{-3}$ | $9.2\times10^{-3}$ | $4.9\times10^{-8}$ | $5.7\times10^{8}$ |
| 7 | $2.4\times10^{-6}$ | $9.4\times10^{4}$ | $4.12\times10^{-4}$ | $4.5\times10^{-3}$ | $4.9\times10^{-8}$ | $5.7\times10^{8}$ |
| 8 | $1.2\times10^{-6}$ | $4.3\times10^{4}$ | $2.08\times10^{-4}$ | $2.2\times10^{-3}$ | $5.2\times10^{-8}$ | $5.3\times10^{8}$ |
| 9 | $6.1\times10^{-7}$ | $1.2\times10^{4}$ | $3.11\times10^{-4}$ | $1.5\times10^{-3}$ | $1.2\times10^{-7}$ | $3.0\times10^{8}$ |
| 10 | $3.1\times10^{-7}$ | $1.0\times10^{3}$ | $1.02\times10^{-4}$ | $2.6\times10^{-4}$ | $2.6\times10^{-7}$ | $4.9\times10^{7}$ |
| $\sum$ | | | $9.96\times10^{-1}$ | | $8.6\times10^{-7}$ | $5.9\times10^{9}$ |

Table 26: $\varepsilon = 0.05$, $\Delta t_1 = 7.81 \times 10^{-5}$

| $\ell$ | $\Delta t_\ell$ | $P_\ell$ | $\mathbb{E}[\hat{F}_\ell - \hat{F}_{\ell-1}]$ | $\mathbb{V}[\hat{F}_\ell - \hat{F}_{\ell-1}]$ | $\mathbb{V}[\hat{Y}_\ell]$ | $P_\ell C_\ell$ |
|---|---|---|---|---|---|---|
| 0 | $5.0\times10^{-1}$ | $1.1\times10^{9}$ | $9.98\times10^{-1}$ | $2.0\times10^{0}$ | $1.7\times10^{-9}$ | $2.3\times10^{7}$ |
| 1 | $7.8\times10^{-5}$ | $2.0\times10^{7}$ | $-1.64\times10^{-2}$ | $3.8\times10^{0}$ | $1.9\times10^{-7}$ | $2.5\times10^{9}$ |
| 2 | $3.9\times10^{-5}$ | $1.5\times10^{6}$ | $7.31\times10^{-3}$ | $6.6\times10^{-2}$ | $4.4\times10^{-8}$ | $5.8\times10^{8}$ |
| 3 | $2.0\times10^{-5}$ | $7.6\times10^{5}$ | $3.44\times10^{-3}$ | $3.4\times10^{-2}$ | $4.4\times10^{-8}$ | $5.8\times10^{8}$ |
| 4 | $9.8\times10^{-6}$ | $3.9\times10^{5}$ | $1.99\times10^{-3}$ | $1.8\times10^{-2}$ | $4.5\times10^{-8}$ | $5.9\times10^{8}$ |
| 5 | $4.9\times10^{-6}$ | $1.9\times10^{5}$ | $1.14\times10^{-3}$ | $8.7\times10^{-3}$ | $4.5\times10^{-8}$ | $5.9\times10^{8}$ |
| 6 | $2.4\times10^{-6}$ | $9.6\times10^{4}$ | $8.24\times10^{-4}$ | $4.2\times10^{-3}$ | $4.4\times10^{-8}$ | $5.9\times10^{8}$ |
| 7 | $1.2\times10^{-6}$ | $4.8\times10^{4}$ | $1.67\times10^{-4}$ | $2.3\times10^{-3}$ | $4.9\times10^{-8}$ | $5.9\times10^{8}$ |
| 8 | $6.1\times10^{-7}$ | $2.1\times10^{4}$ | $7.60\times10^{-5}$ | $1.1\times10^{-3}$ | $5.3\times10^{-8}$ | $5.2\times10^{8}$ |
| 9 | $3.1\times10^{-7}$ | $1.0\times10^{3}$ | $7.45\times10^{-7}$ | $9.8\times10^{-5}$ | $9.8\times10^{-8}$ | $4.9\times10^{7}$ |
| $\sum$ | | | $9.96\times10^{-1}$ | | $6.2\times10^{-7}$ | $6.6\times10^{9}$ |

Table 27: $\varepsilon = 0.05$, $\Delta t_1 = 3.91 \times 10^{-5}$

| $\ell$ | $\Delta t_\ell$ | $P_\ell$ | $\mathbb{E}[\hat{F}_\ell - \hat{F}_{\ell-1}]$ | $\mathbb{V}[\hat{F}_\ell - \hat{F}_{\ell-1}]$ | $\mathbb{V}[\hat{Y}_\ell]$ | $P_\ell C_\ell$ |
|---|---|---|---|---|---|---|
| 0 | $5.0\times10^{-1}$ | $1.1\times10^{9}$ | $9.98\times10^{-1}$ | $2.0\times10^{0}$ | $1.8\times10^{-9}$ | $2.3\times10^{7}$ |
| 1 | $3.9\times10^{-5}$ | $1.4\times10^{7}$ | $-1.04\times10^{-2}$ | $3.8\times10^{0}$ | $2.8\times10^{-7}$ | $3.6\times10^{9}$ |
| 2 | $2.0\times10^{-5}$ | $7.5\times10^{5}$ | $3.63\times10^{-3}$ | $3.4\times10^{-2}$ | $4.5\times10^{-8}$ | $5.8\times10^{8}$ |
| 3 | $9.8\times10^{-6}$ | $3.8\times10^{5}$ | $1.33\times10^{-3}$ | $1.8\times10^{-2}$ | $4.6\times10^{-8}$ | $5.9\times10^{8}$ |
| 4 | $4.9\times10^{-6}$ | $1.9\times10^{5}$ | $5.05\times10^{-4}$ | $8.7\times10^{-3}$ | $4.5\times10^{-8}$ | $5.9\times10^{8}$ |
| 5 | $2.4\times10^{-6}$ | $9.6\times10^{4}$ | $5.55\times10^{-4}$ | $4.2\times10^{-3}$ | $4.4\times10^{-8}$ | $5.9\times10^{8}$ |
| 6 | $1.2\times10^{-6}$ | $4.1\times10^{4}$ | $4.05\times10^{-4}$ | $2.2\times10^{-3}$ | $5.5\times10^{-8}$ | $5.0\times10^{8}$ |
| 7 | $6.1\times10^{-7}$ | $1.0\times10^{3}$ | $2.83\times10^{-4}$ | $2.6\times10^{-3}$ | $2.6\times10^{-6}$ | $2.5\times10^{7}$ |
| $\sum$ | | | $9.94\times10^{-1}$ | | $3.1\times10^{-6}$ | $6.4\times10^{9}$ |

Table 28: $\varepsilon = 0.05$, $\Delta t_1 = 1.95 \times 10^{-5}$

| $\ell$ | $\Delta t_\ell$ | $P_\ell$ | $\mathbb{E}[\hat{F}_\ell - \hat{F}_{\ell-1}]$ | $\mathbb{V}[\hat{F}_\ell - \hat{F}_{\ell-1}]$ | $\mathbb{V}[\hat{Y}_\ell]$ | $P_\ell C_\ell$ |
|---|---|---|---|---|---|---|
| 0 | $5.0\times10^{-1}$ | $1.3\times10^{9}$ | $9.97\times10^{-1}$ | $2.0\times10^{0}$ | $1.5\times10^{-9}$ | $2.6\times10^{7}$ |
| 1 | $2.0\times10^{-5}$ | $1.1\times10^{7}$ | $-5.89\times10^{-3}$ | $3.9\times10^{0}$ | $3.4\times10^{-7}$ | $5.8\times10^{9}$ |
| 2 | $9.8\times10^{-6}$ | $4.4\times10^{5}$ | $1.63\times10^{-3}$ | $1.7\times10^{-2}$ | $4.0\times10^{-8}$ | $6.8\times10^{8}$ |
| 3 | $4.9\times10^{-6}$ | $2.3\times10^{5}$ | $8.95\times10^{-4}$ | $9.3\times10^{-3}$ | $4.1\times10^{-8}$ | $7.0\times10^{8}$ |
| 4 | $2.4\times10^{-6}$ | $1.0\times10^{5}$ | $4.25\times10^{-4}$ | $4.0\times10^{-3}$ | $3.8\times10^{-8}$ | $6.4\times10^{8}$ |
| 5 | $1.2\times10^{-6}$ | $5.2\times10^{4}$ | $3.93\times10^{-4}$ | $2.1\times10^{-3}$ | $4.0\times10^{-8}$ | $6.4\times10^{8}$ |
| 6 | $6.1\times10^{-7}$ | $1.0\times10^{3}$ | $1.07\times10^{-4}$ | $6.3\times10^{-4}$ | $6.3\times10^{-7}$ | $2.5\times10^{7}$ |
| $\sum$ | | | $9.95\times10^{-1}$ | | $1.1\times10^{-6}$ | $8.5\times10^{9}$ |

Table 29: $\varepsilon = 0.05$, $\Delta t_1 = 9.77 \times 10^{-6}$

| $\ell$ | $\Delta t_\ell$ | $P_\ell$ | $\mathbb{E}[\hat{F}_\ell - \hat{F}_{\ell-1}]$ | $\mathbb{V}[\hat{F}_\ell - \hat{F}_{\ell-1}]$ | $\mathbb{V}[\hat{Y}_\ell]$ | $P_\ell C_\ell$ |
|---|---|---|---|---|---|---|
| 0 | $5.0\times10^{-1}$ | $1.8\times10^{9}$ | $9.98\times10^{-1}$ | $2.0\times10^{0}$ | $1.1\times10^{-9}$ | $3.7\times10^{7}$ |
| 1 | $9.8\times10^{-6}$ | $1.1\times10^{7}$ | $-4.31\times10^{-3}$ | $3.9\times10^{0}$ | $3.4\times10^{-7}$ | $1.2\times10^{10}$ |
| 2 | $4.9\times10^{-6}$ | $3.1\times10^{5}$ | $8.25\times10^{-4}$ | $8.8\times10^{-3}$ | $2.8\times10^{-8}$ | $9.6\times10^{8}$ |
| 3 | $2.4\times10^{-6}$ | $1.6\times10^{5}$ | $6.16\times10^{-4}$ | $4.4\times10^{-3}$ | $2.8\times10^{-8}$ | $9.6\times10^{8}$ |
| 4 | $1.2\times10^{-6}$ | $7.8\times10^{4}$ | $2.51\times10^{-4}$ | $2.2\times10^{-3}$ | $2.8\times10^{-8}$ | $9.6\times10^{8}$ |
| 5 | $6.1\times10^{-7}$ | $5.8\times10^{4}$ | $2.04\times10^{-4}$ | $1.1\times10^{-3}$ | $1.9\times10^{-8}$ | $1.4\times10^{9}$ |
| 6 | $3.1\times10^{-7}$ | $3.0\times10^{4}$ | $1.12\times10^{-4}$ | $5.4\times10^{-4}$ | $1.8\times10^{-8}$ | $1.5\times10^{9}$ |
| 7 | $1.5\times10^{-7}$ | $1.0\times10^{3}$ | $3.60\times10^{-4}$ | $1.5\times10^{-4}$ | $1.5\times10^{-7}$ | $9.8\times10^{7}$ |
| $\sum$ | | | $9.96\times10^{-1}$ | | $6.2\times10^{-7}$ | $1.8\times10^{10}$ |

Table 30: $\varepsilon = 0.05$, $\Delta t_1 = 4.88 \times 10^{-6}$

| $\ell$ | $\Delta t_\ell$ | $P_\ell$ | $\mathbb{E}[\hat{F}_\ell - \hat{F}_{\ell-1}]$ | $\mathbb{V}[\hat{F}_\ell - \hat{F}_{\ell-1}]$ | $\mathbb{V}[\hat{Y}_\ell]$ | $P_\ell C_\ell$ |
|---|---|---|---|---|---|---|
| 0 | $5.0\times10^{-1}$ | $2.1\times10^{9}$ | $9.97\times10^{-1}$ | $2.0\times10^{0}$ | $9.6\times10^{-10}$ | $4.2\times10^{7}$ |
| 1 | $4.9\times10^{-6}$ | $9.1\times10^{6}$ | $-3.48\times10^{-3}$ | $3.9\times10^{0}$ | $4.3\times10^{-7}$ | $1.9\times10^{10}$ |
| 2 | $2.4\times10^{-6}$ | $1.7\times10^{5}$ | $4.52\times10^{-4}$ | $4.3\times10^{-3}$ | $2.5\times10^{-8}$ | $1.1\times10^{9}$ |
| 3 | $1.2\times10^{-6}$ | $8.9\times10^{4}$ | $1.09\times10^{-4}$ | $2.3\times10^{-3}$ | $2.5\times10^{-8}$ | $1.1\times10^{9}$ |
| 4 | $6.1\times10^{-7}$ | $3.5\times10^{4}$ | $-1.44\times10^{-4}$ | $9.3\times10^{-4}$ | $2.6\times10^{-8}$ | $8.7\times10^{8}$ |
| 5 | $3.1\times10^{-7}$ | $1.0\times10^{3}$ | $-3.19\times10^{-4}$ | $9.6\times10^{-5}$ | $9.6\times10^{-8}$ | $4.9\times10^{7}$ |
| $\sum$ | | | $9.94\times10^{-1}$ | | $6.0\times10^{-7}$ | $2.2\times10^{10}$ |

Table 31: $\varepsilon = 0.05$, $\Delta t_1 = 2.44 \times 10^{-6}$

| $\ell$ | $\Delta t_\ell$ | $P_\ell$ | $\mathbb{E}[\hat{F}_\ell - \hat{F}_{\ell-1}]$ | $\mathbb{V}[\hat{F}_\ell - \hat{F}_{\ell-1}]$ | $\mathbb{V}[\hat{Y}_\ell]$ | $P_\ell C_\ell$ |
|---|---|---|---|---|---|---|
| 0 | $5.0\times10^{-1}$ | $2.8\times10^{9}$ | $9.98\times10^{-1}$ | $2.0\times10^{0}$ | $7.2\times10^{-10}$ | $5.5\times10^{7}$ |
| 1 | $2.4\times10^{-6}$ | $8.6\times10^{6}$ | $-3.39\times10^{-3}$ | $3.9\times10^{0}$ | $4.6\times10^{-7}$ | $3.5\times10^{10}$ |
| 2 | $1.2\times10^{-6}$ | $1.2\times10^{5}$ | $1.67\times10^{-4}$ | $2.4\times10^{-3}$ | $2.0\times10^{-8}$ | $1.5\times10^{9}$ |
| 3 | $6.1\times10^{-7}$ | $6.9\times10^{4}$ | $-5.48\times10^{-6}$ | $1.2\times10^{-3}$ | $1.8\times10^{-8}$ | $1.7\times10^{9}$ |
| 4 | $3.1\times10^{-7}$ | $1.0\times10^{3}$ | $-2.52\times10^{-4}$ | $1.3\times10^{-4}$ | $1.3\times10^{-7}$ | $4.9\times10^{7}$ |
| $\sum$ | | | $9.94\times10^{-1}$ | | $6.2\times10^{-7}$ | $3.9\times10^{10}$ |

Table 32: $\varepsilon = 0.05$, $\Delta t_1 = 1.22 \times 10^{-6}$

| $\ell$ | $\Delta t_\ell$ | $P_\ell$ | $\mathbb{E}[\hat{F}_\ell - \hat{F}_{\ell-1}]$ | $\mathbb{V}[\hat{F}_\ell - \hat{F}_{\ell-1}]$ | $\mathbb{V}[\hat{Y}_\ell]$ | $P_\ell C_\ell$ |
|---|---|---|---|---|---|---|
| 0 | $5.0\times10^{-1}$ | $3.9\times10^{9}$ | $9.97\times10^{-1}$ | $2.0\times10^{0}$ | $5.2\times10^{-10}$ | $7.7\times10^{7}$ |
| 1 | $1.2\times10^{-6}$ | $8.5\times10^{6}$ | $-2.70\times10^{-3}$ | $3.9\times10^{0}$ | $4.7\times10^{-7}$ | $6.9\times10^{10}$ |
| 2 | $6.1\times10^{-7}$ | $7.9\times10^{4}$ | $7.29\times10^{-5}$ | $1.1\times10^{-3}$ | $1.4\times10^{-8}$ | $1.9\times10^{9}$ |
| 3 | $3.1\times10^{-7}$ | $6.4\times10^{4}$ | $-3.48\times10^{-5}$ | $5.6\times10^{-4}$ | $8.8\times10^{-9}$ | $3.1\times10^{9}$ |
| 4 | $1.5\times10^{-7}$ | $1.0\times10^{3}$ | $-9.59\times10^{-5}$ | $6.6\times10^{-5}$ | $6.6\times10^{-8}$ | $9.8\times10^{7}$ |
| $\sum$ | | | $9.95\times10^{-1}$ | | $5.5\times10^{-7}$ | $7.5\times10^{10}$ |

## 1.4 Combined correlation, $\varepsilon = 0.5$

Table 33: $\varepsilon = 0.5$, $\Delta t_1 = 2.50 \times 10^{-1}$

| $\ell$ | $\Delta t_\ell$ | $P_\ell$ | $\mathbb{E}[\hat{F}_\ell - \hat{F}_{\ell-1}]$ | $\mathbb{V}[\hat{F}_\ell - \hat{F}_{\ell-1}]$ | $\mathbb{V}[\hat{Y}_\ell]$ | $P_\ell C_\ell$ |
|---|---|---|---|---|---|---|
| 0 | $5.0\times10^{-1}$ | $2.9\times10^{7}$ | $7.78\times10^{-1}$ | $1.2\times10^{0}$ | $4.1\times10^{-8}$ | $5.8\times10^{5}$ |
| 1 | $2.5\times10^{-1}$ | $6.1\times10^{6}$ | $-9.03\times10^{-2}$ | $1.6\times10^{-1}$ | $2.6\times10^{-8}$ | $3.6\times10^{5}$ |
| 2 | $1.2\times10^{-1}$ | $3.9\times10^{6}$ | $-6.60\times10^{-2}$ | $1.3\times10^{-1}$ | $3.4\times10^{-8}$ | $4.7\times10^{5}$ |
| 3 | $6.2\times10^{-2}$ | $2.3\times10^{6}$ | $-3.43\times10^{-2}$ | $8.7\times10^{-2}$ | $3.9\times10^{-8}$ | $5.4\times10^{5}$ |
| 4 | $3.1\times10^{-2}$ | $1.2\times10^{6}$ | $-1.37\times10^{-2}$ | $5.2\times10^{-2}$ | $4.2\times10^{-8}$ | $5.9\times10^{5}$ |
| 5 | $1.6\times10^{-2}$ | $6.4\times10^{5}$ | $-4.22\times10^{-3}$ | $2.9\times10^{-2}$ | $4.4\times10^{-8}$ | $6.2\times10^{5}$ |
| 6 | $7.8\times10^{-3}$ | $3.3\times10^{5}$ | $-1.31\times10^{-3}$ | $1.5\times10^{-2}$ | $4.6\times10^{-8}$ | $6.4\times10^{5}$ |
| 7 | $3.9\times10^{-3}$ | $1.7\times10^{5}$ | $-3.74\times10^{-4}$ | $7.8\times10^{-3}$ | $4.6\times10^{-8}$ | $6.5\times10^{5}$ |
| 8 | $2.0\times10^{-3}$ | $8.5\times10^{4}$ | $1.40\times10^{-4}$ | $3.9\times10^{-3}$ | $4.6\times10^{-8}$ | $6.5\times10^{5}$ |
| 9 | $9.8\times10^{-4}$ | $4.2\times10^{4}$ | $-2.04\times10^{-4}$ | $2.0\times10^{-3}$ | $4.7\times10^{-8}$ | $6.5\times10^{5}$ |
| 10 | $4.9\times10^{-4}$ | $2.4\times10^{4}$ | $-6.28\times10^{-5}$ | $9.9\times10^{-4}$ | $4.1\times10^{-8}$ | $7.4\times10^{5}$ |
| 11 | $2.4\times10^{-4}$ | $9.7\times10^{3}$ | $8.67\times10^{-5}$ | $6.0\times10^{-4}$ | $6.2\times10^{-8}$ | $5.9\times10^{5}$ |
| 12 | $1.2\times10^{-4}$ | $1.0\times10^{3}$ | $7.02\times10^{-4}$ | $1.8\times10^{-4}$ | $1.8\times10^{-7}$ | $1.2\times10^{5}$ |
| $\sum$ | | | $5.68\times10^{-1}$ | | $6.9\times10^{-7}$ | $7.2\times10^{6}$ |

Table 34: $\varepsilon = 0.5$, $\Delta t_1 = 1.25 \times 10^{-1}$

| $\ell$ | $\Delta t_\ell$ | $P_\ell$ | $\mathbb{E}[\hat{F}_\ell - \hat{F}_{\ell-1}]$ | $\mathbb{V}[\hat{F}_\ell - \hat{F}_{\ell-1}]$ | $\mathbb{V}[\hat{Y}_\ell]$ | $P_\ell C_\ell$ |
|---|---|---|---|---|---|---|
| 0 | $5.0\times10^{-1}$ | $2.0\times10^{7}$ | $7.78\times10^{-1}$ | $1.2\times10^{0}$ | $5.8\times10^{-8}$ | $4.1\times10^{5}$ |
| 1 | $1.2\times10^{-1}$ | $5.4\times10^{6}$ | $-1.56\times10^{-1}$ | $4.2\times10^{-1}$ | $7.7\times10^{-8}$ | $5.4\times10^{5}$ |
| 2 | $6.2\times10^{-2}$ | $1.6\times10^{6}$ | $-3.42\times10^{-2}$ | $8.7\times10^{-2}$ | $5.4\times10^{-8}$ | $3.8\times10^{5}$ |
| 3 | $3.1\times10^{-2}$ | $8.7\times10^{5}$ | $-1.30\times10^{-2}$ | $5.2\times10^{-2}$ | $5.9\times10^{-8}$ | $4.2\times10^{5}$ |
| 4 | $1.6\times10^{-2}$ | $4.6\times10^{5}$ | $-3.63\times10^{-3}$ | $2.8\times10^{-2}$ | $6.2\times10^{-8}$ | $4.4\times10^{5}$ |
| 5 | $7.8\times10^{-3}$ | $2.4\times10^{5}$ | $-1.26\times10^{-3}$ | $1.5\times10^{-2}$ | $6.4\times10^{-8}$ | $4.6\times10^{5}$ |
| 6 | $3.9\times10^{-3}$ | $1.4\times10^{5}$ | $-3.54\times10^{-4}$ | $7.8\times10^{-3}$ | $5.6\times10^{-8}$ | $5.3\times10^{5}$ |
| 7 | $2.0\times10^{-3}$ | $5.6\times10^{4}$ | $7.39\times10^{-5}$ | $3.9\times10^{-3}$ | $7.0\times10^{-8}$ | $4.3\times10^{5}$ |
| 8 | $9.8\times10^{-4}$ | $1.0\times10^{3}$ | $-1.16\times10^{-4}$ | $2.4\times10^{-3}$ | $2.4\times10^{-6}$ | $1.5\times10^{4}$ |
| $\sum$ | | | $5.69\times10^{-1}$ | | $2.9\times10^{-6}$ | $3.6\times10^{6}$ |

Table 35: $\varepsilon = 0.5$, $\Delta t_1 = 6.25 \times 10^{-2}$

| $\ell$ | $\Delta t_\ell$ | $P_\ell$ | $\mathbb{E}[\hat{F}_\ell - \hat{F}_{\ell-1}]$ | $\mathbb{V}[\hat{F}_\ell - \hat{F}_{\ell-1}]$ | $\mathbb{V}[\hat{Y}_\ell]$ | $P_\ell C_\ell$ |
|---|---|---|---|---|---|---|
| 0 | $5.0\times10^{-1}$ | $2.6\times10^{7}$ | $7.77\times10^{-1}$ | $1.2\times10^{0}$ | $4.6\times10^{-8}$ | $5.1\times10^{5}$ |
| 1 | $6.2\times10^{-2}$ | $6.5\times10^{6}$ | $-1.91\times10^{-1}$ | $6.7\times10^{-1}$ | $1.0\times10^{-7}$ | $1.2\times10^{6}$ |
| 2 | $3.1\times10^{-2}$ | $1.1\times10^{6}$ | $-1.33\times10^{-2}$ | $5.2\times10^{-2}$ | $4.7\times10^{-8}$ | $5.2\times10^{5}$ |
| 3 | $1.6\times10^{-2}$ | $5.8\times10^{5}$ | $-4.39\times10^{-3}$ | $2.9\times10^{-2}$ | $5.0\times10^{-8}$ | $5.5\times10^{5}$ |
| 4 | $7.8\times10^{-3}$ | $3.0\times10^{5}$ | $-1.25\times10^{-3}$ | $1.5\times10^{-2}$ | $5.1\times10^{-8}$ | $5.7\times10^{5}$ |
| 5 | $3.9\times10^{-3}$ | $1.5\times10^{5}$ | $-3.18\times10^{-4}$ | $7.7\times10^{-3}$ | $5.2\times10^{-8}$ | $5.7\times10^{5}$ |
| 6 | $2.0\times10^{-3}$ | $7.9\times10^{4}$ | $-4.36\times10^{-5}$ | $4.3\times10^{-3}$ | $5.4\times10^{-8}$ | $6.1\times10^{5}$ |
| 7 | $9.8\times10^{-4}$ | $3.9\times10^{4}$ | $1.20\times10^{-4}$ | $1.9\times10^{-3}$ | $4.9\times10^{-8}$ | $6.0\times10^{5}$ |
| 8 | $4.9\times10^{-4}$ | $1.6\times10^{4}$ | $-2.11\times10^{-4}$ | $1.0\times10^{-3}$ | $6.7\times10^{-8}$ | $4.8\times10^{5}$ |
| 9 | $2.4\times10^{-4}$ | $1.0\times10^{3}$ | $-2.60\times10^{-4}$ | $3.8\times10^{-4}$ | $3.8\times10^{-7}$ | $6.1\times10^{4}$ |
| $\sum$ | | | $5.67\times10^{-1}$ | | $9.0\times10^{-7}$ | $5.7\times10^{6}$ |

Table 36: $\varepsilon = 0.5$, $\Delta t_1 = 3.12 \times 10^{-2}$

| $\ell$ | $\Delta t_\ell$ | $P_\ell$ | $\mathbb{E}[\hat{F}_\ell - \hat{F}_{\ell-1}]$ | $\mathbb{V}[\hat{F}_\ell - \hat{F}_{\ell-1}]$ | $\mathbb{V}[\hat{Y}_\ell]$ | $P_\ell C_\ell$ |
|---|---|---|---|---|---|---|
| 0 | $5.0\times10^{-1}$ | $2.1\times10^{7}$ | $7.78\times10^{-1}$ | $1.2\times10^{0}$ | $5.6\times10^{-8}$ | $4.3\times10^{5}$ |
| 1 | $3.1\times10^{-2}$ | $4.4\times10^{6}$ | $-2.04\times10^{-1}$ | $8.6\times10^{-1}$ | $2.0\times10^{-7}$ | $1.5\times10^{6}$ |
| 2 | $1.6\times10^{-2}$ | $4.8\times10^{5}$ | $-4.30\times10^{-3}$ | $2.9\times10^{-2}$ | $6.0\times10^{-8}$ | $4.6\times10^{5}$ |
| 3 | $7.8\times10^{-3}$ | $2.5\times10^{5}$ | $-1.05\times10^{-3}$ | $1.5\times10^{-2}$ | $6.2\times10^{-8}$ | $4.7\times10^{5}$ |
| 4 | $3.9\times10^{-3}$ | $1.2\times10^{5}$ | $-1.01\times10^{-4}$ | $7.8\times10^{-3}$ | $6.2\times10^{-8}$ | $4.8\times10^{5}$ |
| 5 | $2.0\times10^{-3}$ | $6.4\times10^{4}$ | $2.88\times10^{-5}$ | $3.9\times10^{-3}$ | $6.1\times10^{-8}$ | $4.9\times10^{5}$ |
| 6 | $9.8\times10^{-4}$ | $1.0\times10^{3}$ | $-6.05\times10^{-4}$ | $2.3\times10^{-3}$ | $2.3\times10^{-6}$ | $1.5\times10^{4}$ |
| $\sum$ | | | $5.67\times10^{-1}$ | | $2.8\times10^{-6}$ | $3.8\times10^{6}$ |

Table 37: $\varepsilon = 0.5$, $\Delta t_1 = 1.56 \times 10^{-2}$

| $\ell$ | $\Delta t_\ell$ | $P_\ell$ | $\mathbb{E}[\hat{F}_\ell - \hat{F}_{\ell-1}]$ | $\mathbb{V}[\hat{F}_\ell - \hat{F}_{\ell-1}]$ | $\mathbb{V}[\hat{Y}_\ell]$ | $P_\ell C_\ell$ |
|---|---|---|---|---|---|---|
| 0 | $5.0\times10^{-1}$ | $2.8\times10^{7}$ | $7.78\times10^{-1}$ | $1.2\times10^{0}$ | $4.2\times10^{-8}$ | $5.6\times10^{5}$ |
| 1 | $1.6\times10^{-2}$ | $4.4\times10^{6}$ | $-2.09\times10^{-1}$ | $9.6\times10^{-1}$ | $2.2\times10^{-7}$ | $2.9\times10^{6}$ |
| 2 | $7.8\times10^{-3}$ | $3.2\times10^{5}$ | $-1.23\times10^{-3}$ | $1.5\times10^{-2}$ | $4.7\times10^{-8}$ | $6.2\times10^{5}$ |
| 3 | $3.9\times10^{-3}$ | $1.7\times10^{5}$ | $-5.08\times10^{-4}$ | $8.2\times10^{-3}$ | $4.8\times10^{-8}$ | $6.5\times10^{5}$ |
| 4 | $2.0\times10^{-3}$ | $8.1\times10^{4}$ | $-3.77\times10^{-4}$ | $3.8\times10^{-3}$ | $4.7\times10^{-8}$ | $6.3\times10^{5}$ |
| 5 | $9.8\times10^{-4}$ | $4.0\times10^{4}$ | $7.91\times10^{-5}$ | $1.9\times10^{-3}$ | $4.6\times10^{-8}$ | $6.2\times10^{5}$ |
| 6 | $4.9\times10^{-4}$ | $2.2\times10^{4}$ | $9.36\times10^{-5}$ | $9.0\times10^{-4}$ | $4.2\times10^{-8}$ | $6.6\times10^{5}$ |
| 7 | $2.4\times10^{-4}$ | $1.0\times10^{3}$ | $-3.37\times10^{-4}$ | $3.8\times10^{-4}$ | $3.8\times10^{-7}$ | $6.1\times10^{4}$ |
| $\sum$ | | | $5.67\times10^{-1}$ | | $8.7\times10^{-7}$ | $6.7\times10^{6}$ |

Table 38: $\varepsilon = 0.5$, $\Delta t_1 = 7.81 \times 10^{-3}$

| $\ell$ | $\Delta t_\ell$ | $P_\ell$ | $\mathbb{E}[\hat{F}_\ell - \hat{F}_{\ell-1}]$ | $\mathbb{V}[\hat{F}_\ell - \hat{F}_{\ell-1}]$ | $\mathbb{V}[\hat{Y}_\ell]$ | $P_\ell C_\ell$ |
|---|---|---|---|---|---|---|
| 0 | $5.0\times10^{-1}$ | $2.7\times10^{7}$ | $7.78\times10^{-1}$ | $1.2\times10^{0}$ | $4.3\times10^{-8}$ | $5.5\times10^{5}$ |
| 1 | $7.8\times10^{-3}$ | $3.1\times10^{6}$ | $-2.09\times10^{-1}$ | $9.7\times10^{-1}$ | $3.2\times10^{-7}$ | $4.0\times10^{6}$ |
| 2 | $3.9\times10^{-3}$ | $1.6\times10^{5}$ | $-1.65\times10^{-4}$ | $7.9\times10^{-3}$ | $4.9\times10^{-8}$ | $6.2\times10^{5}$ |
| 3 | $2.0\times10^{-3}$ | $8.0\times10^{4}$ | $-2.99\times10^{-4}$ | $4.0\times10^{-3}$ | $4.9\times10^{-8}$ | $6.2\times10^{5}$ |
| 4 | $9.8\times10^{-4}$ | $3.4\times10^{4}$ | $-3.05\times10^{-4}$ | $2.0\times10^{-3}$ | $5.9\times10^{-8}$ | $5.3\times10^{5}$ |
| 5 | $4.9\times10^{-4}$ | $1.0\times10^{3}$ | $-5.00\times10^{-4}$ | $7.2\times10^{-4}$ | $7.2\times10^{-7}$ | $3.1\times10^{4}$ |
| $\sum$ | | | $5.67\times10^{-1}$ | | $1.2\times10^{-6}$ | $6.3\times10^{6}$ |

Table 39: $\varepsilon = 0.5$, $\Delta t_1 = 3.91 \times 10^{-3}$

| $\ell$ | $\Delta t_\ell$ | $P_\ell$ | $\mathbb{E}[\hat{F}_\ell - \hat{F}_{\ell-1}]$ | $\mathbb{V}[\hat{F}_\ell - \hat{F}_{\ell-1}]$ | $\mathbb{V}[\hat{Y}_\ell]$ | $P_\ell C_\ell$ |
|---|---|---|---|---|---|---|
| 0 | $5.0\times10^{-1}$ | $3.4\times10^{7}$ | $7.78\times10^{-1}$ | $1.2\times10^{0}$ | $3.5\times10^{-8}$ | $6.7\times10^{5}$ |
| 1 | $3.9\times10^{-3}$ | $2.6\times10^{6}$ | $-2.11\times10^{-1}$ | $9.0\times10^{-1}$ | $3.5\times10^{-7}$ | $6.6\times10^{6}$ |
| 2 | $2.0\times10^{-3}$ | $9.9\times10^{4}$ | $1.72\times10^{-4}$ | $4.0\times10^{-3}$ | $4.0\times10^{-8}$ | $7.6\times10^{5}$ |
| 3 | $9.8\times10^{-4}$ | $7.2\times10^{4}$ | $-1.26\times10^{-4}$ | $2.0\times10^{-3}$ | $2.8\times10^{-8}$ | $1.1\times10^{6}$ |
| 4 | $4.9\times10^{-4}$ | $2.2\times10^{4}$ | $-1.59\times10^{-4}$ | $1.0\times10^{-3}$ | $4.7\times10^{-8}$ | $6.6\times10^{5}$ |
| 5 | $2.4\times10^{-4}$ | $1.0\times10^{3}$ | $1.02\times10^{-5}$ | $4.2\times10^{-4}$ | $4.2\times10^{-7}$ | $6.1\times10^{4}$ |
| $\sum$ | | | $5.68\times10^{-1}$ | | $9.2\times10^{-7}$ | $9.9\times10^{6}$ |

Table 40: $\varepsilon = 0.5$, $\Delta t_1 = 1.95 \times 10^{-3}$

| $\ell$ | $\Delta t_\ell$ | $P_\ell$ | $\mathbb{E}[\hat{F}_\ell - \hat{F}_{\ell-1}]$ | $\mathbb{V}[\hat{F}_\ell - \hat{F}_{\ell-1}]$ | $\mathbb{V}[\hat{Y}_\ell]$ | $P_\ell C_\ell$ |
|---|---|---|---|---|---|---|
| 0 | $5.0\times10^{-1}$ | $3.8\times10^{7}$ | $7.78\times10^{-1}$ | $1.2\times10^{0}$ | $3.1\times10^{-8}$ | $7.7\times10^{5}$ |
| 1 | $2.0\times10^{-3}$ | $1.9\times10^{6}$ | $-2.10\times10^{-1}$ | $7.8\times10^{-1}$ | $4.0\times10^{-7}$ | $1.0\times10^{7}$ |
| 2 | $9.8\times10^{-4}$ | $5.7\times10^{4}$ | $2.51\times10^{-5}$ | $2.0\times10^{-3}$ | $3.5\times10^{-8}$ | $8.8\times10^{5}$ |
| 3 | $4.9\times10^{-4}$ | $2.4\times10^{4}$ | $-1.21\times10^{-4}$ | $1.0\times10^{-3}$ | $4.3\times10^{-8}$ | $7.4\times10^{5}$ |
| 4 | $2.4\times10^{-4}$ | $1.0\times10^{3}$ | $5.40\times10^{-4}$ | $3.9\times10^{-4}$ | $3.9\times10^{-7}$ | $6.1\times10^{4}$ |
| $\sum$ | | | $5.68\times10^{-1}$ | | $9.1\times10^{-7}$ | $1.2\times10^{7}$ |

Table 41: $\varepsilon = 0.5$, $\Delta t_1 = 9.77 \times 10^{-4}$

| $\ell$ | $\Delta t_\ell$ | $P_\ell$ | $\mathbb{E}[\hat{F}_\ell - \hat{F}_{\ell-1}]$ | $\mathbb{V}[\hat{F}_\ell - \hat{F}_{\ell-1}]$ | $\mathbb{V}[\hat{Y}_\ell]$ | $P_\ell C_\ell$ |
|---|---|---|---|---|---|---|
| 0 | $5.0\times10^{-1}$ | $5.2\times10^{7}$ | $7.78\times10^{-1}$ | $1.2\times10^{0}$ | $2.3\times10^{-8}$ | $1.0\times10^{6}$ |
| 1 | $9.8\times10^{-4}$ | $1.9\times10^{6}$ | $-2.10\times10^{-1}$ | $8.0\times10^{-1}$ | $4.3\times10^{-7}$ | $1.9\times10^{7}$ |
| 2 | $4.9\times10^{-4}$ | $4.0\times10^{4}$ | $-1.86\times10^{-4}$ | $1.1\times10^{-3}$ | $2.6\times10^{-8}$ | $1.2\times10^{6}$ |
| 3 | $2.4\times10^{-4}$ | $1.7\times10^{4}$ | $1.19\times10^{-4}$ | $4.8\times10^{-4}$ | $2.9\times10^{-8}$ | $1.0\times10^{6}$ |
| 4 | $1.2\times10^{-4}$ | $1.0\times10^{3}$ | $3.73\times10^{-4}$ | $2.1\times10^{-4}$ | $2.1\times10^{-7}$ | $1.2\times10^{5}$ |
| $\sum$ | | | $5.69\times10^{-1}$ | | $7.1\times10^{-7}$ | $2.3\times10^{7}$ |

Table 42: $\varepsilon = 0.5$, $\Delta t_1 = 4.88 \times 10^{-4}$

| $\ell$ | $\Delta t_\ell$ | $P_\ell$ | $\mathbb{E}[\hat{F}_\ell - \hat{F}_{\ell-1}]$ | $\mathbb{V}[\hat{F}_\ell - \hat{F}_{\ell-1}]$ | $\mathbb{V}[\hat{Y}_\ell]$ | $P_\ell C_\ell$ |
|---|---|---|---|---|---|---|
| 0 | $5.0\times10^{-1}$ | $7.1\times10^{7}$ | $7.78\times10^{-1}$ | $1.2\times10^{0}$ | $1.7\times10^{-8}$ | $1.4\times10^{6}$ |
| 1 | $4.9\times10^{-4}$ | $1.8\times10^{6}$ | $-2.10\times10^{-1}$ | $8.1\times10^{-1}$ | $4.4\times10^{-7}$ | $3.8\times10^{7}$ |
| 2 | $2.4\times10^{-4}$ | $3.4\times10^{4}$ | $3.95\times10^{-5}$ | $6.4\times10^{-4}$ | $1.9\times10^{-8}$ | $2.1\times10^{6}$ |
| 3 | $1.2\times10^{-4}$ | $1.1\times10^{4}$ | $5.53\times10^{-5}$ | $2.5\times10^{-4}$ | $2.2\times10^{-8}$ | $1.4\times10^{6}$ |
| 4 | $6.1\times10^{-5}$ | $1.0\times10^{3}$ | $9.04\times10^{-5}$ | $9.6\times10^{-5}$ | $9.6\times10^{-8}$ | $2.5\times10^{5}$ |
| $\sum$ | | | $5.68\times10^{-1}$ | | $6.0\times10^{-7}$ | $4.3\times10^{7}$ |

## 1.5 Combined correlation, $\varepsilon = 0.1$

Table 43: $\varepsilon = 0.1$, $\Delta t_1 = 1.00 \times 10^{-2}$

| $\ell$ | $\Delta t_\ell$ | $P_\ell$ | $\mathbb{E}[\hat{F}_\ell - \hat{F}_{\ell-1}]$ | $\mathbb{V}[\hat{F}_\ell - \hat{F}_{\ell-1}]$ | $\mathbb{V}[\hat{Y}_\ell]$ | $P_\ell C_\ell$ |
|---|---|---|---|---|---|---|
| 0 | $5.0\times10^{-1}$ | $4.5\times10^{8}$ | $9.90\times10^{-1}$ | $2.0\times10^{0}$ | $4.3\times10^{-9}$ | $9.1\times10^{6}$ |
| 1 | $1.0\times10^{-2}$ | $1.8\times10^{7}$ | $-1.25\times10^{-1}$ | $1.6\times10^{-1}$ | $8.8\times10^{-9}$ | $1.9\times10^{7}$ |
| 2 | $5.0\times10^{-3}$ | $1.8\times10^{7}$ | $1.04\times10^{-2}$ | $4.4\times10^{-1}$ | $2.5\times10^{-8}$ | $5.3\times10^{7}$ |
| 3 | $2.5\times10^{-3}$ | $1.2\times10^{7}$ | $2.85\times10^{-2}$ | $4.0\times10^{-1}$ | $3.4\times10^{-8}$ | $7.1\times10^{7}$ |
| 4 | $1.3\times10^{-3}$ | $7.3\times10^{6}$ | $2.86\times10^{-2}$ | $3.0\times10^{-1}$ | $4.2\times10^{-8}$ | $8.8\times10^{7}$ |
| 5 | $6.3\times10^{-4}$ | $4.1\times10^{6}$ | $2.06\times10^{-2}$ | $1.9\times10^{-1}$ | $4.7\times10^{-8}$ | $9.9\times10^{7}$ |
| 6 | $3.1\times10^{-4}$ | $2.2\times10^{6}$ | $1.24\times10^{-2}$ | $1.1\times10^{-1}$ | $5.0\times10^{-8}$ | $1.1\times10^{8}$ |
| 7 | $1.6\times10^{-4}$ | $1.2\times10^{6}$ | $6.84\times10^{-3}$ | $6.0\times10^{-2}$ | $5.2\times10^{-8}$ | $1.1\times10^{8}$ |
| 8 | $7.8\times10^{-5}$ | $5.8\times10^{5}$ | $3.55\times10^{-3}$ | $3.1\times10^{-2}$ | $5.3\times10^{-8}$ | $1.1\times10^{8}$ |
| 9 | $3.9\times10^{-5}$ | $2.9\times10^{5}$ | $1.38\times10^{-3}$ | $1.6\times10^{-2}$ | $5.4\times10^{-8}$ | $1.1\times10^{8}$ |
| 10 | $2.0\times10^{-5}$ | $1.6\times10^{5}$ | $9.31\times10^{-4}$ | $8.8\times10^{-3}$ | $5.6\times10^{-8}$ | $1.2\times10^{8}$ |
| 11 | $9.8\times10^{-6}$ | $7.0\times10^{4}$ | $6.67\times10^{-4}$ | $3.6\times10^{-3}$ | $5.2\times10^{-8}$ | $1.1\times10^{8}$ |
| 12 | $4.9\times10^{-6}$ | $1.5\times10^{4}$ | $-1.13\times10^{-4}$ | $2.5\times10^{-3}$ | $1.6\times10^{-7}$ | $4.7\times10^{7}$ |
| 13 | $2.4\times10^{-6}$ | $1.0\times10^{3}$ | $2.24\times10^{-4}$ | $3.5\times10^{-4}$ | $3.5\times10^{-7}$ | $6.1\times10^{6}$ |
| $\sum$ | | | $9.79\times10^{-1}$ | | $1.0\times10^{-6}$ | $1.1\times10^{9}$ |

Table 44: $\varepsilon = 0.1$, $\Delta t_1 = 5.00 \times 10^{-3}$

| $\ell$ | $\Delta t_\ell$ | $P_\ell$ | $\mathbb{E}[\hat{F}_\ell - \hat{F}_{\ell-1}]$ | $\mathbb{V}[\hat{F}_\ell - \hat{F}_{\ell-1}]$ | $\mathbb{V}[\hat{Y}_\ell]$ | $P_\ell C_\ell$ |
|---|---|---|---|---|---|---|
| 0 | $5.0\times10^{-1}$ | $4.2\times10^{8}$ | $9.90\times10^{-1}$ | $2.0\times10^{0}$ | $4.7\times10^{-9}$ | $8.3\times10^{6}$ |
| 1 | $5.0\times10^{-3}$ | $1.3\times10^{7}$ | $-1.14\times10^{-1}$ | $1.9\times10^{-1}$ | $1.5\times10^{-8}$ | $2.6\times10^{7}$ |
| 2 | $2.5\times10^{-3}$ | $1.1\times10^{7}$ | $2.84\times10^{-2}$ | $4.0\times10^{-1}$ | $3.7\times10^{-8}$ | $6.5\times10^{7}$ |
| 3 | $1.3\times10^{-3}$ | $6.7\times10^{6}$ | $2.86\times10^{-2}$ | $3.0\times10^{-1}$ | $4.5\times10^{-8}$ | $8.0\times10^{7}$ |
| 4 | $6.3\times10^{-4}$ | $3.8\times10^{6}$ | $2.08\times10^{-2}$ | $2.0\times10^{-1}$ | $5.2\times10^{-8}$ | $9.1\times10^{7}$ |
| 5 | $3.1\times10^{-4}$ | $2.0\times10^{6}$ | $1.24\times10^{-2}$ | $1.1\times10^{-1}$ | $5.5\times10^{-8}$ | $9.7\times10^{7}$ |
| 6 | $1.6\times10^{-4}$ | $1.0\times10^{6}$ | $7.03\times10^{-3}$ | $6.0\times10^{-2}$ | $5.7\times10^{-8}$ | $1.0\times10^{8}$ |
| 7 | $7.8\times10^{-5}$ | $5.3\times10^{5}$ | $3.81\times10^{-3}$ | $3.0\times10^{-2}$ | $5.8\times10^{-8}$ | $1.0\times10^{8}$ |
| 8 | $3.9\times10^{-5}$ | $2.9\times10^{5}$ | $2.16\times10^{-3}$ | $1.6\times10^{-2}$ | $5.6\times10^{-8}$ | $1.1\times10^{8}$ |
| 9 | $2.0\times10^{-5}$ | $1.5\times10^{5}$ | $6.70\times10^{-4}$ | $7.4\times10^{-3}$ | $5.1\times10^{-8}$ | $1.1\times10^{8}$ |
| 10 | $9.8\times10^{-6}$ | $7.0\times10^{4}$ | $2.25\times10^{-4}$ | $3.9\times10^{-3}$ | $5.5\times10^{-8}$ | $1.1\times10^{8}$ |
| 11 | $4.9\times10^{-6}$ | $1.0\times10^{3}$ | $-2.91\times10^{-4}$ | $5.5\times10^{-4}$ | $5.5\times10^{-7}$ | $3.1\times10^{6}$ |
| $\sum$ | | | $9.80\times10^{-1}$ | | $1.0\times10^{-6}$ | $9.0\times10^{8}$ |

Table 45: $\varepsilon = 0.1$, $\Delta t_1 = 2.50 \times 10^{-3}$

| $\ell$ | $\Delta t_\ell$ | $P_\ell$ | $\mathbb{E}[\hat{F}_\ell - \hat{F}_{\ell-1}]$ | $\mathbb{V}[\hat{F}_\ell - \hat{F}_{\ell-1}]$ | $\mathbb{V}[\hat{Y}_\ell]$ | $P_\ell C_\ell$ |
|---|---|---|---|---|---|---|
| 0 | $5.0\times10^{-1}$ | $4.4\times10^{8}$ | $9.90\times10^{-1}$ | $2.0\times10^{0}$ | $4.4\times10^{-9}$ | $8.9\times10^{6}$ |
| 1 | $2.5\times10^{-3}$ | $1.0\times10^{7}$ | $-8.62\times10^{-2}$ | $2.2\times10^{-1}$ | $2.1\times10^{-8}$ | $4.2\times10^{7}$ |
| 2 | $1.3\times10^{-3}$ | $7.1\times10^{6}$ | $2.90\times10^{-2}$ | $3.0\times10^{-1}$ | $4.3\times10^{-8}$ | $8.6\times10^{7}$ |
| 3 | $6.3\times10^{-4}$ | $4.0\times10^{6}$ | $2.06\times10^{-2}$ | $1.9\times10^{-1}$ | $4.8\times10^{-8}$ | $9.7\times10^{7}$ |
| 4 | $3.1\times10^{-4}$ | $2.2\times10^{6}$ | $1.22\times10^{-2}$ | $1.1\times10^{-1}$ | $5.2\times10^{-8}$ | $1.0\times10^{8}$ |
| 5 | $1.6\times10^{-4}$ | $1.1\times10^{6}$ | $6.93\times10^{-3}$ | $6.0\times10^{-2}$ | $5.4\times10^{-8}$ | $1.1\times10^{8}$ |
| 6 | $7.8\times10^{-5}$ | $5.6\times10^{5}$ | $3.57\times10^{-3}$ | $3.0\times10^{-2}$ | $5.4\times10^{-8}$ | $1.1\times10^{8}$ |
| 7 | $3.9\times10^{-5}$ | $2.9\times10^{5}$ | $1.88\times10^{-3}$ | $1.6\times10^{-2}$ | $5.5\times10^{-8}$ | $1.1\times10^{8}$ |
| 8 | $2.0\times10^{-5}$ | $1.5\times10^{5}$ | $6.98\times10^{-4}$ | $7.9\times10^{-3}$ | $5.4\times10^{-8}$ | $1.1\times10^{8}$ |
| 9 | $9.8\times10^{-6}$ | $7.8\times10^{4}$ | $5.86\times10^{-4}$ | $4.4\times10^{-3}$ | $5.7\times10^{-8}$ | $1.2\times10^{8}$ |
| 10 | $4.9\times10^{-6}$ | $3.5\times10^{4}$ | $-1.08\times10^{-4}$ | $1.8\times10^{-3}$ | $5.1\times10^{-8}$ | $1.1\times10^{8}$ |
| 11 | $2.4\times10^{-6}$ | $1.0\times10^{3}$ | $5.65\times10^{-4}$ | $3.2\times10^{-4}$ | $3.2\times10^{-7}$ | $6.1\times10^{6}$ |
| $\sum$ | | | $9.80\times10^{-1}$ | | $8.1\times10^{-7}$ | $1.0\times10^{9}$ |

Table 46: $\varepsilon = 0.1$, $\Delta t_1 = 1.25 \times 10^{-3}$

| $\ell$ | $\Delta t_\ell$ | $P_\ell$ | $\mathbb{E}[\hat{F}_\ell - \hat{F}_{\ell-1}]$ | $\mathbb{V}[\hat{F}_\ell - \hat{F}_{\ell-1}]$ | $\mathbb{V}[\hat{Y}_\ell]$ | $P_\ell C_\ell$ |
|---|---|---|---|---|---|---|
| 0 | $5.0\times10^{-1}$ | $4.6\times10^{8}$ | $9.90\times10^{-1}$ | $2.0\times10^{0}$ | $4.2\times10^{-9}$ | $9.3\times10^{6}$ |
| 1 | $1.3\times10^{-3}$ | $8.0\times10^{6}$ | $-5.76\times10^{-2}$ | $2.3\times10^{-1}$ | $2.9\times10^{-8}$ | $6.4\times10^{7}$ |
| 2 | $6.3\times10^{-4}$ | $4.2\times10^{6}$ | $2.04\times10^{-2}$ | $2.0\times10^{-1}$ | $4.6\times10^{-8}$ | $1.0\times10^{8}$ |
| 3 | $3.1\times10^{-4}$ | $2.2\times10^{6}$ | $1.23\times10^{-2}$ | $1.1\times10^{-1}$ | $4.9\times10^{-8}$ | $1.1\times10^{8}$ |
| 4 | $1.6\times10^{-4}$ | $1.2\times10^{6}$ | $6.63\times10^{-3}$ | $6.0\times10^{-2}$ | $5.1\times10^{-8}$ | $1.1\times10^{8}$ |
| 5 | $7.8\times10^{-5}$ | $5.9\times10^{5}$ | $3.92\times10^{-3}$ | $3.1\times10^{-2}$ | $5.2\times10^{-8}$ | $1.1\times10^{8}$ |
| 6 | $3.9\times10^{-5}$ | $3.0\times10^{5}$ | $2.15\times10^{-3}$ | $1.5\times10^{-2}$ | $5.2\times10^{-8}$ | $1.1\times10^{8}$ |
| 7 | $2.0\times10^{-5}$ | $1.5\times10^{5}$ | $9.71\times10^{-4}$ | $7.8\times10^{-3}$ | $5.2\times10^{-8}$ | $1.1\times10^{8}$ |
| 8 | $9.8\times10^{-6}$ | $8.2\times10^{4}$ | $2.04\times10^{-4}$ | $3.5\times10^{-3}$ | $4.3\times10^{-8}$ | $1.3\times10^{8}$ |
| 9 | $4.9\times10^{-6}$ | $3.2\times10^{4}$ | $2.64\times10^{-4}$ | $1.4\times10^{-3}$ | $4.4\times10^{-8}$ | $9.8\times10^{7}$ |
| 10 | $2.4\times10^{-6}$ | $1.7\times10^{4}$ | $3.28\times10^{-4}$ | $7.9\times10^{-4}$ | $4.6\times10^{-8}$ | $1.1\times10^{8}$ |
| 11 | $1.2\times10^{-6}$ | $3.8\times10^{3}$ | $6.95\times10^{-4}$ | $2.4\times10^{-4}$ | $6.3\times10^{-8}$ | $4.7\times10^{7}$ |
| 12 | $6.1\times10^{-7}$ | $1.0\times10^{3}$ | $3.68\times10^{-4}$ | $3.8\times10^{-5}$ | $3.8\times10^{-8}$ | $2.5\times10^{7}$ |
| $\sum$ | | | $9.81\times10^{-1}$ | | $5.7\times10^{-7}$ | $1.1\times10^{9}$ |

Table 47: $\varepsilon = 0.1$, $\Delta t_1 = 6.25 \times 10^{-4}$

| $\ell$ | $\Delta t_\ell$ | $P_\ell$ | $\mathbb{E}[\hat{F}_\ell - \hat{F}_{\ell-1}]$ | $\mathbb{V}[\hat{F}_\ell - \hat{F}_{\ell-1}]$ | $\mathbb{V}[\hat{Y}_\ell]$ | $P_\ell C_\ell$ |
|---|---|---|---|---|---|---|
| 0 | $5.0\times10^{-1}$ | $3.5\times10^{8}$ | $9.90\times10^{-1}$ | $2.0\times10^{0}$ | $5.6\times10^{-9}$ | $7.0\times10^{6}$ |
| 1 | $6.3\times10^{-4}$ | $4.4\times10^{6}$ | $-3.68\times10^{-2}$ | $2.4\times10^{-1}$ | $5.6\times10^{-8}$ | $7.0\times10^{7}$ |
| 2 | $3.1\times10^{-4}$ | $1.7\times10^{6}$ | $1.24\times10^{-2}$ | $1.1\times10^{-1}$ | $6.6\times10^{-8}$ | $8.2\times10^{7}$ |
| 3 | $1.6\times10^{-4}$ | $8.8\times10^{5}$ | $6.88\times10^{-3}$ | $6.0\times10^{-2}$ | $6.8\times10^{-8}$ | $8.5\times10^{7}$ |
| 4 | $7.8\times10^{-5}$ | $4.5\times10^{5}$ | $3.81\times10^{-3}$ | $3.1\times10^{-2}$ | $7.0\times10^{-8}$ | $8.6\times10^{7}$ |
| 5 | $3.9\times10^{-5}$ | $2.3\times10^{5}$ | $1.88\times10^{-3}$ | $1.7\times10^{-2}$ | $7.1\times10^{-8}$ | $9.0\times10^{7}$ |
| 6 | $2.0\times10^{-5}$ | $1.1\times10^{5}$ | $6.45\times10^{-4}$ | $7.7\times10^{-3}$ | $6.9\times10^{-8}$ | $8.5\times10^{7}$ |
| 7 | $9.8\times10^{-6}$ | $7.9\times10^{4}$ | $3.89\times10^{-4}$ | $4.5\times10^{-3}$ | $5.7\times10^{-8}$ | $1.2\times10^{8}$ |
| 8 | $4.9\times10^{-6}$ | $1.0\times10^{3}$ | $3.73\times10^{-4}$ | $6.7\times10^{-4}$ | $6.7\times10^{-7}$ | $3.1\times10^{6}$ |
| $\sum$ | | | $9.80\times10^{-1}$ | | $1.1\times10^{-6}$ | $6.3\times10^{8}$ |

Table 48: $\varepsilon = 0.1$, $\Delta t_1 = 3.13 \times 10^{-4}$

| $\ell$ | $\Delta t_\ell$ | $P_\ell$ | $\mathbb{E}[\hat{F}_\ell - \hat{F}_{\ell-1}]$ | $\mathbb{V}[\hat{F}_\ell - \hat{F}_{\ell-1}]$ | $\mathbb{V}[\hat{Y}_\ell]$ | $P_\ell C_\ell$ |
|---|---|---|---|---|---|---|
| 0 | $5.0\times10^{-1}$ | $3.1\times10^{8}$ | $9.90\times10^{-1}$ | $2.0\times10^{0}$ | $6.3\times10^{-9}$ | $6.2\times10^{6}$ |
| 1 | $3.1\times10^{-4}$ | $2.8\times10^{6}$ | $-2.36\times10^{-2}$ | $2.5\times10^{-1}$ | $9.1\times10^{-8}$ | $8.8\times10^{7}$ |
| 2 | $1.6\times10^{-4}$ | $7.8\times10^{5}$ | $6.78\times10^{-3}$ | $6.1\times10^{-2}$ | $7.8\times10^{-8}$ | $7.5\times10^{7}$ |
| 3 | $7.8\times10^{-5}$ | $4.0\times10^{5}$ | $3.68\times10^{-3}$ | $3.1\times10^{-2}$ | $7.9\times10^{-8}$ | $7.7\times10^{7}$ |
| 4 | $3.9\times10^{-5}$ | $1.9\times10^{5}$ | $1.88\times10^{-3}$ | $1.5\times10^{-2}$ | $7.7\times10^{-8}$ | $7.5\times10^{7}$ |
| 5 | $2.0\times10^{-5}$ | $1.0\times10^{5}$ | $6.47\times10^{-4}$ | $8.2\times10^{-3}$ | $8.0\times10^{-8}$ | $7.8\times10^{7}$ |
| 6 | $9.8\times10^{-6}$ | $5.7\times10^{4}$ | $5.35\times10^{-4}$ | $3.9\times10^{-3}$ | $6.9\times10^{-8}$ | $8.7\times10^{7}$ |
| 7 | $4.9\times10^{-6}$ | $1.0\times10^{3}$ | $1.96\times10^{-4}$ | $8.7\times10^{-4}$ | $8.7\times10^{-7}$ | $3.1\times10^{6}$ |
| $\sum$ | | | $9.80\times10^{-1}$ | | $1.3\times10^{-6}$ | $4.9\times10^{8}$ |

Table 49: $\varepsilon = 0.1$, $\Delta t_1 = 1.56 \times 10^{-4}$

| $\ell$ | $\Delta t_\ell$ | $P_\ell$ | $\mathbb{E}[\hat{F}_\ell - \hat{F}_{\ell-1}]$ | $\mathbb{V}[\hat{F}_\ell - \hat{F}_{\ell-1}]$ | $\mathbb{V}[\hat{Y}_\ell]$ | $P_\ell C_\ell$ |
|---|---|---|---|---|---|---|
| 0 | $5.0\times10^{-1}$ | $3.1\times10^{8}$ | $9.90\times10^{-1}$ | $2.0\times10^{0}$ | $6.3\times10^{-9}$ | $6.2\times10^{6}$ |
| 1 | $1.6\times10^{-4}$ | $2.0\times10^{6}$ | $-1.77\times10^{-2}$ | $2.5\times10^{-1}$ | $1.3\times10^{-7}$ | $1.3\times10^{8}$ |
| 2 | $7.8\times10^{-5}$ | $4.0\times10^{5}$ | $3.38\times10^{-3}$ | $3.1\times10^{-2}$ | $7.7\times10^{-8}$ | $7.7\times10^{7}$ |
| 3 | $3.9\times10^{-5}$ | $2.0\times10^{5}$ | $2.10\times10^{-3}$ | $1.6\times10^{-2}$ | $7.9\times10^{-8}$ | $7.8\times10^{7}$ |
| 4 | $2.0\times10^{-5}$ | $1.1\times10^{5}$ | $8.65\times10^{-4}$ | $8.8\times10^{-3}$ | $8.1\times10^{-8}$ | $8.3\times10^{7}$ |
| 5 | $9.8\times10^{-6}$ | $4.5\times10^{4}$ | $3.71\times10^{-4}$ | $4.3\times10^{-3}$ | $9.6\times10^{-8}$ | $6.9\times10^{7}$ |
| 6 | $4.9\times10^{-6}$ | $1.8\times10^{4}$ | $9.03\times10^{-6}$ | $1.9\times10^{-3}$ | $1.1\times10^{-7}$ | $5.4\times10^{7}$ |
| 7 | $2.4\times10^{-6}$ | $1.0\times10^{3}$ | $-5.05\times10^{-4}$ | $3.9\times10^{-4}$ | $3.9\times10^{-7}$ | $6.1\times10^{6}$ |
| $\sum$ | | | $9.79\times10^{-1}$ | | $9.7\times10^{-7}$ | $5.0\times10^{8}$ |

Table 50: $\varepsilon = 0.1$, $\Delta t_1 = 7.81 \times 10^{-5}$

| $\ell$ | $\Delta t_\ell$ | $P_\ell$ | $\mathbb{E}[\hat{F}_\ell - \hat{F}_{\ell-1}]$ | $\mathbb{V}[\hat{F}_\ell - \hat{F}_{\ell-1}]$ | $\mathbb{V}[\hat{Y}_\ell]$ | $P_\ell C_\ell$ |
|---|---|---|---|---|---|---|
| 0 | $5.0\times10^{-1}$ | $4.1\times10^{8}$ | $9.90\times10^{-1}$ | $2.0\times10^{0}$ | $4.7\times10^{-9}$ | $8.3\times10^{6}$ |
| 1 | $7.8\times10^{-5}$ | $1.9\times10^{6}$ | $-1.38\times10^{-2}$ | $2.6\times10^{-1}$ | $1.4\times10^{-7}$ | $2.4\times10^{8}$ |
| 2 | $3.9\times10^{-5}$ | $2.7\times10^{5}$ | $1.90\times10^{-3}$ | $1.6\times10^{-2}$ | $6.0\times10^{-8}$ | $1.0\times10^{8}$ |
| 3 | $2.0\times10^{-5}$ | $1.3\times10^{5}$ | $1.17\times10^{-3}$ | $7.5\times10^{-3}$ | $5.8\times10^{-8}$ | $9.9\times10^{7}$ |
| 4 | $9.8\times10^{-6}$ | $9.1\times10^{4}$ | $7.83\times10^{-4}$ | $3.8\times10^{-3}$ | $4.2\times10^{-8}$ | $1.4\times10^{8}$ |
| 5 | $4.9\times10^{-6}$ | $3.5\times10^{4}$ | $7.04\times10^{-5}$ | $2.1\times10^{-3}$ | $6.2\times10^{-8}$ | $1.1\times10^{8}$ |
| 6 | $2.4\times10^{-6}$ | $2.0\times10^{4}$ | $3.44\times10^{-4}$ | $1.3\times10^{-3}$ | $6.3\times10^{-8}$ | $1.2\times10^{8}$ |
| 7 | $1.2\times10^{-6}$ | $7.6\times10^{3}$ | $-6.41\times10^{-5}$ | $5.6\times10^{-4}$ | $7.4\times10^{-8}$ | $9.3\times10^{7}$ |
| 8 | $6.1\times10^{-7}$ | $1.0\times10^{3}$ | $5.58\times10^{-4}$ | $3.6\times10^{-5}$ | $3.6\times10^{-8}$ | $2.5\times10^{7}$ |
| $\sum$ | | | $9.81\times10^{-1}$ | | $5.3\times10^{-7}$ | $9.4\times10^{8}$ |

Table 51: $\varepsilon = 0.1$, $\Delta t_1 = 3.91 \times 10^{-5}$

| $\ell$ | $\Delta t_\ell$ | $P_\ell$ | $\mathbb{E}[\hat{F}_\ell - \hat{F}_{\ell-1}]$ | $\mathbb{V}[\hat{F}_\ell - \hat{F}_{\ell-1}]$ | $\mathbb{V}[\hat{Y}_\ell]$ | $P_\ell C_\ell$ |
|---|---|---|---|---|---|---|
| 0 | $5.0\times10^{-1}$ | $5.5\times10^{8}$ | $9.90\times10^{-1}$ | $2.0\times10^{0}$ | $3.5\times10^{-9}$ | $1.1\times10^{7}$ |
| 1 | $3.9\times10^{-5}$ | $1.8\times10^{6}$ | $-1.22\times10^{-2}$ | $2.5\times10^{-1}$ | $1.4\times10^{-7}$ | $4.5\times10^{8}$ |
| 2 | $2.0\times10^{-5}$ | $1.9\times10^{5}$ | $9.13\times10^{-4}$ | $8.1\times10^{-3}$ | $4.4\times10^{-8}$ | $1.4\times10^{8}$ |
| 3 | $9.8\times10^{-6}$ | $9.2\times10^{4}$ | $3.42\times10^{-4}$ | $4.9\times10^{-3}$ | $5.3\times10^{-8}$ | $1.4\times10^{8}$ |
| 4 | $4.9\times10^{-6}$ | $4.8\times10^{4}$ | $4.37\times10^{-4}$ | $2.1\times10^{-3}$ | $4.3\times10^{-8}$ | $1.5\times10^{8}$ |
| 5 | $2.4\times10^{-6}$ | $3.2\times10^{4}$ | $8.51\times10^{-5}$ | $2.2\times10^{-3}$ | $6.8\times10^{-8}$ | $1.9\times10^{8}$ |
| 6 | $1.2\times10^{-6}$ | $3.9\times10^{4}$ | $4.14\times10^{-5}$ | $7.4\times10^{-4}$ | $1.9\times10^{-8}$ | $4.8\times10^{8}$ |
| 7 | $6.1\times10^{-7}$ | $1.0\times10^{3}$ | $-1.54\times10^{-4}$ | $4.6\times10^{-5}$ | $4.6\times10^{-8}$ | $2.5\times10^{7}$ |
| $\sum$ | | | $9.79\times10^{-1}$ | | $4.2\times10^{-7}$ | $1.6\times10^{9}$ |

Table 52: $\varepsilon = 0.1$, $\Delta t_1 = 1.95 \times 10^{-5}$

| $\ell$ | $\Delta t_\ell$ | $P_\ell$ | $\mathbb{E}[\hat{F}_\ell - \hat{F}_{\ell-1}]$ | $\mathbb{V}[\hat{F}_\ell - \hat{F}_{\ell-1}]$ | $\mathbb{V}[\hat{Y}_\ell]$ | $P_\ell C_\ell$ |
|---|---|---|---|---|---|---|
| 0 | $5.0\times10^{-1}$ | $3.6\times10^{8}$ | $9.90\times10^{-1}$ | $2.0\times10^{0}$ | $5.4\times10^{-9}$ | $7.3\times10^{6}$ |
| 1 | $2.0\times10^{-5}$ | $8.2\times10^{5}$ | $-1.09\times10^{-2}$ | $2.6\times10^{-1}$ | $3.1\times10^{-7}$ | $4.2\times10^{8}$ |
| 2 | $9.8\times10^{-6}$ | $5.4\times10^{4}$ | $9.84\times10^{-4}$ | $3.4\times10^{-3}$ | $6.2\times10^{-8}$ | $8.3\times10^{7}$ |
| 3 | $4.9\times10^{-6}$ | $2.7\times10^{4}$ | $3.36\times10^{-4}$ | $1.4\times10^{-3}$ | $5.0\times10^{-8}$ | $8.4\times10^{7}$ |
| 4 | $2.4\times10^{-6}$ | $1.5\times10^{4}$ | $1.62\times10^{-5}$ | $6.2\times10^{-4}$ | $4.2\times10^{-8}$ | $9.1\times10^{7}$ |
| 5 | $1.2\times10^{-6}$ | $1.0\times10^{3}$ | $2.90\times10^{-4}$ | $8.2\times10^{-5}$ | $8.2\times10^{-8}$ | $1.2\times10^{7}$ |
| $\sum$ | | | $9.81\times10^{-1}$ | | $5.5\times10^{-7}$ | $7.0\times10^{8}$ |

## 1.6 Combined correlation, $\varepsilon = 0.05$

Table 53: $\varepsilon = 0.05$, $\Delta t_1 = 2.50 \times 10^{-3}$

| $\ell$ | $\Delta t_\ell$ | $P_\ell$ | $\mathbb{E}[\hat{F}_\ell - \hat{F}_{\ell-1}]$ | $\mathbb{V}[\hat{F}_\ell - \hat{F}_{\ell-1}]$ | $\mathbb{V}[\hat{Y}_\ell]$ | $P_\ell C_\ell$ |
|---|---|---|---|---|---|---|
| 0 | $5.0\times10^{-1}$ | $1.0\times10^{9}$ | $9.97\times10^{-1}$ | $2.0\times10^{0}$ | $1.9\times10^{-9}$ | $2.1\times10^{7}$ |
| 1 | $2.5\times10^{-3}$ | $1.3\times10^{7}$ | $-1.25\times10^{-1}$ | $6.5\times10^{-2}$ | $4.9\times10^{-9}$ | $5.4\times10^{7}$ |
| 2 | $1.3\times10^{-3}$ | $2.1\times10^{7}$ | $1.29\times10^{-2}$ | $4.7\times10^{-1}$ | $2.3\times10^{-8}$ | $2.5\times10^{8}$ |
| 3 | $6.3\times10^{-4}$ | $1.4\times10^{7}$ | $3.05\times10^{-2}$ | $4.4\times10^{-1}$ | $3.1\times10^{-8}$ | $3.4\times10^{8}$ |
| 4 | $3.1\times10^{-4}$ | $8.7\times10^{6}$ | $3.02\times10^{-2}$ | $3.3\times10^{-1}$ | $3.8\times10^{-8}$ | $4.2\times10^{8}$ |
| 5 | $1.6\times10^{-4}$ | $4.9\times10^{6}$ | $2.17\times10^{-2}$ | $2.1\times10^{-1}$ | $4.3\times10^{-8}$ | $4.7\times10^{8}$ |
| 6 | $7.8\times10^{-5}$ | $2.6\times10^{6}$ | $1.25\times10^{-2}$ | $1.2\times10^{-1}$ | $4.6\times10^{-8}$ | $5.1\times10^{8}$ |
| 7 | $3.9\times10^{-5}$ | $1.4\times10^{6}$ | $6.92\times10^{-3}$ | $6.6\times10^{-2}$ | $4.8\times10^{-8}$ | $5.3\times10^{8}$ |
| 8 | $2.0\times10^{-5}$ | $7.0\times10^{5}$ | $3.52\times10^{-3}$ | $3.4\times10^{-2}$ | $4.9\times10^{-8}$ | $5.3\times10^{8}$ |
| 9 | $9.8\times10^{-6}$ | $3.5\times10^{5}$ | $2.00\times10^{-3}$ | $1.7\times10^{-2}$ | $4.9\times10^{-8}$ | $5.4\times10^{8}$ |
| 10 | $4.9\times10^{-6}$ | $1.8\times10^{5}$ | $1.08\times10^{-3}$ | $9.0\times10^{-3}$ | $5.0\times10^{-8}$ | $5.5\times10^{8}$ |
| 11 | $2.4\times10^{-6}$ | $9.5\times10^{4}$ | $4.10\times10^{-4}$ | $4.6\times10^{-3}$ | $4.9\times10^{-8}$ | $5.8\times10^{8}$ |
| 12 | $1.2\times10^{-6}$ | $5.5\times10^{4}$ | $3.40\times10^{-4}$ | $2.3\times10^{-3}$ | $4.2\times10^{-8}$ | $6.8\times10^{8}$ |
| 13 | $6.1\times10^{-7}$ | $1.0\times10^{3}$ | $-2.72\times10^{-4}$ | $5.7\times10^{-4}$ | $5.7\times10^{-7}$ | $2.5\times10^{7}$ |
| $\sum$ | | | $9.94\times10^{-1}$ | | $1.0\times10^{-6}$ | $5.5\times10^{9}$ |

Table 54: $\varepsilon = 0.05$, $\Delta t_1 = 1.25 \times 10^{-3}$

| $\ell$ | $\Delta t_\ell$ | $P_\ell$ | $\mathbb{E}[\hat{F}_\ell - \hat{F}_{\ell-1}]$ | $\mathbb{V}[\hat{F}_\ell - \hat{F}_{\ell-1}]$ | $\mathbb{V}[\hat{Y}_\ell]$ | $P_\ell C_\ell$ |
|---|---|---|---|---|---|---|
| 0 | $5.0\times10^{-1}$ | $9.7\times10^{8}$ | $9.97\times10^{-1}$ | $2.0\times10^{0}$ | $2.1\times10^{-9}$ | $1.9\times10^{7}$ |
| 1 | $1.3\times10^{-3}$ | $9.0\times10^{6}$ | $-1.12\times10^{-1}$ | $6.9\times10^{-2}$ | $7.7\times10^{-9}$ | $7.2\times10^{7}$ |
| 2 | $6.3\times10^{-4}$ | $1.3\times10^{7}$ | $3.06\times10^{-2}$ | $4.3\times10^{-1}$ | $3.3\times10^{-8}$ | $3.1\times10^{8}$ |
| 3 | $3.1\times10^{-4}$ | $8.0\times10^{6}$ | $3.01\times10^{-2}$ | $3.3\times10^{-1}$ | $4.1\times10^{-8}$ | $3.9\times10^{8}$ |
| 4 | $1.6\times10^{-4}$ | $4.6\times10^{6}$ | $2.13\times10^{-2}$ | $2.1\times10^{-1}$ | $4.7\times10^{-8}$ | $4.4\times10^{8}$ |
| 5 | $7.8\times10^{-5}$ | $2.5\times10^{6}$ | $1.29\times10^{-2}$ | $1.2\times10^{-1}$ | $5.0\times10^{-8}$ | $4.7\times10^{8}$ |
| 6 | $3.9\times10^{-5}$ | $1.3\times10^{6}$ | $7.14\times10^{-3}$ | $6.6\times10^{-2}$ | $5.2\times10^{-8}$ | $4.9\times10^{8}$ |
| 7 | $2.0\times10^{-5}$ | $6.5\times10^{5}$ | $3.79\times10^{-3}$ | $3.4\times10^{-2}$ | $5.3\times10^{-8}$ | $5.0\times10^{8}$ |
| 8 | $9.8\times10^{-6}$ | $3.3\times10^{5}$ | $1.65\times10^{-3}$ | $1.8\times10^{-2}$ | $5.3\times10^{-8}$ | $5.0\times10^{8}$ |
| 9 | $4.9\times10^{-6}$ | $1.6\times10^{5}$ | $8.04\times10^{-4}$ | $8.7\times10^{-3}$ | $5.4\times10^{-8}$ | $5.0\times10^{8}$ |
| 10 | $2.4\times10^{-6}$ | $8.9\times10^{4}$ | $4.78\times10^{-4}$ | $5.0\times10^{-3}$ | $5.6\times10^{-8}$ | $5.5\times10^{8}$ |
| 11 | $1.2\times10^{-6}$ | $3.9\times10^{4}$ | $3.16\times10^{-4}$ | $2.4\times10^{-3}$ | $6.1\times10^{-8}$ | $4.8\times10^{8}$ |
| 12 | $6.1\times10^{-7}$ | $1.0\times10^{3}$ | $-2.05\times10^{-4}$ | $3.6\times10^{-4}$ | $3.6\times10^{-7}$ | $2.5\times10^{7}$ |
| $\sum$ | | | $9.94\times10^{-1}$ | | $8.7\times10^{-7}$ | $4.7\times10^{9}$ |

Table 55: $\varepsilon = 0.05$, $\Delta t_1 = 6.25 \times 10^{-4}$

| $\ell$ | $\Delta t_\ell$ | $P_\ell$ | $\mathbb{E}[\hat{F}_\ell - \hat{F}_{\ell-1}]$ | $\mathbb{V}[\hat{F}_\ell - \hat{F}_{\ell-1}]$ | $\mathbb{V}[\hat{Y}_\ell]$ | $P_\ell C_\ell$ |
|---|---|---|---|---|---|---|
| 0 | $5.0\times10^{-1}$ | $9.9\times10^{8}$ | $9.97\times10^{-1}$ | $2.0\times10^{0}$ | $2.0\times10^{-9}$ | $2.0\times10^{7}$ |
| 1 | $6.3\times10^{-4}$ | $6.4\times10^{6}$ | $-8.17\times10^{-2}$ | $6.7\times10^{-2}$ | $1.0\times10^{-8}$ | $1.0\times10^{8}$ |
| 2 | $3.1\times10^{-4}$ | $8.3\times10^{6}$ | $3.00\times10^{-2}$ | $3.3\times10^{-1}$ | $4.0\times10^{-8}$ | $4.0\times10^{8}$ |
| 3 | $1.6\times10^{-4}$ | $4.7\times10^{6}$ | $2.16\times10^{-2}$ | $2.1\times10^{-1}$ | $4.5\times10^{-8}$ | $4.5\times10^{8}$ |
| 4 | $7.8\times10^{-5}$ | $2.5\times10^{6}$ | $1.27\times10^{-2}$ | $1.2\times10^{-1}$ | $4.9\times10^{-8}$ | $4.8\times10^{8}$ |
| 5 | $3.9\times10^{-5}$ | $1.3\times10^{6}$ | $6.61\times10^{-3}$ | $6.6\times10^{-2}$ | $5.0\times10^{-8}$ | $5.0\times10^{8}$ |
| 6 | $2.0\times10^{-5}$ | $6.6\times10^{5}$ | $3.52\times10^{-3}$ | $3.4\times10^{-2}$ | $5.1\times10^{-8}$ | $5.1\times10^{8}$ |
| 7 | $9.8\times10^{-6}$ | $3.3\times10^{5}$ | $1.96\times10^{-3}$ | $1.7\times10^{-2}$ | $5.2\times10^{-8}$ | $5.1\times10^{8}$ |
| 8 | $4.9\times10^{-6}$ | $1.7\times10^{5}$ | $9.12\times10^{-4}$ | $9.3\times10^{-3}$ | $5.4\times10^{-8}$ | $5.3\times10^{8}$ |
| 9 | $2.4\times10^{-6}$ | $8.7\times10^{4}$ | $9.02\times10^{-4}$ | $4.7\times10^{-3}$ | $5.4\times10^{-8}$ | $5.3\times10^{8}$ |
| 10 | $1.2\times10^{-6}$ | $4.4\times10^{4}$ | $-2.29\times10^{-4}$ | $2.2\times10^{-3}$ | $5.0\times10^{-8}$ | $5.3\times10^{8}$ |
| 11 | $6.1\times10^{-7}$ | $1.6\times10^{4}$ | $2.13\times10^{-4}$ | $9.7\times10^{-4}$ | $6.0\times10^{-8}$ | $4.0\times10^{8}$ |
| 12 | $3.1\times10^{-7}$ | $1.0\times10^{3}$ | $-4.54\times10^{-5}$ | $5.9\times10^{-4}$ | $5.9\times10^{-7}$ | $4.9\times10^{7}$ |
| $\sum$ | | | $9.94\times10^{-1}$ | | $1.1\times10^{-6}$ | $5.0\times10^{9}$ |

Table 56: $\varepsilon = 0.05$, $\Delta t_1 = 3.13 \times 10^{-4}$

| $\ell$ | $\Delta t_\ell$ | $P_\ell$ | $\mathbb{E}[\hat{F}_\ell - \hat{F}_{\ell-1}]$ | $\mathbb{V}[\hat{F}_\ell - \hat{F}_{\ell-1}]$ | $\mathbb{V}[\hat{Y}_\ell]$ | $P_\ell C_\ell$ |
|---|---|---|---|---|---|---|
| 0 | $5.0\times10^{-1}$ | $9.9\times10^{8}$ | $9.98\times10^{-1}$ | $2.0\times10^{0}$ | $2.0\times10^{-9}$ | $2.0\times10^{7}$ |
| 1 | $3.1\times10^{-4}$ | $4.5\times10^{6}$ | $-5.12\times10^{-2}$ | $6.5\times10^{-2}$ | $1.5\times10^{-8}$ | $1.4\times10^{8}$ |
| 2 | $1.6\times10^{-4}$ | $4.7\times10^{6}$ | $2.13\times10^{-2}$ | $2.1\times10^{-1}$ | $4.5\times10^{-8}$ | $4.5\times10^{8}$ |
| 3 | $7.8\times10^{-5}$ | $2.5\times10^{6}$ | $1.32\times10^{-2}$ | $1.2\times10^{-1}$ | $4.9\times10^{-8}$ | $4.8\times10^{8}$ |
| 4 | $3.9\times10^{-5}$ | $1.3\times10^{6}$ | $7.57\times10^{-3}$ | $6.5\times10^{-2}$ | $5.0\times10^{-8}$ | $5.0\times10^{8}$ |
| 5 | $2.0\times10^{-5}$ | $6.6\times10^{5}$ | $3.58\times10^{-3}$ | $3.4\times10^{-2}$ | $5.2\times10^{-8}$ | $5.1\times10^{8}$ |
| 6 | $9.8\times10^{-6}$ | $3.3\times10^{5}$ | $2.24\times10^{-3}$ | $1.7\times10^{-2}$ | $5.2\times10^{-8}$ | $5.1\times10^{8}$ |
| 7 | $4.9\times10^{-6}$ | $1.7\times10^{5}$ | $1.11\times10^{-3}$ | $8.7\times10^{-3}$ | $5.2\times10^{-8}$ | $5.2\times10^{8}$ |
| 8 | $2.4\times10^{-6}$ | $8.8\times10^{4}$ | $1.86\times10^{-4}$ | $4.8\times10^{-3}$ | $5.4\times10^{-8}$ | $5.4\times10^{8}$ |
| 9 | $1.2\times10^{-6}$ | $4.7\times10^{4}$ | $1.24\times10^{-4}$ | $2.7\times10^{-3}$ | $5.7\times10^{-8}$ | $5.8\times10^{8}$ |
| 10 | $6.1\times10^{-7}$ | $2.8\times10^{4}$ | $1.93\times10^{-5}$ | $1.1\times10^{-3}$ | $4.1\times10^{-8}$ | $6.9\times10^{8}$ |
| 11 | $3.1\times10^{-7}$ | $1.0\times10^{3}$ | $-5.63\times10^{-4}$ | $2.0\times10^{-4}$ | $2.0\times10^{-7}$ | $4.9\times10^{7}$ |
| $\sum$ | | | $9.95\times10^{-1}$ | | $6.7\times10^{-7}$ | $5.0\times10^{9}$ |

Table 57: $\varepsilon = 0.05$, $\Delta t_1 = 1.56 \times 10^{-4}$

| $\ell$ | $\Delta t_\ell$ | $P_\ell$ | $\mathbb{E}[\hat{F}_\ell - \hat{F}_{\ell-1}]$ | $\mathbb{V}[\hat{F}_\ell - \hat{F}_{\ell-1}]$ | $\mathbb{V}[\hat{Y}_\ell]$ | $P_\ell C_\ell$ |
|---|---|---|---|---|---|---|
| 0 | $5.0\times10^{-1}$ | $8.5\times10^{8}$ | $9.98\times10^{-1}$ | $2.0\times10^{0}$ | $2.3\times10^{-9}$ | $1.7\times10^{7}$ |
| 1 | $1.6\times10^{-4}$ | $2.7\times10^{6}$ | $-2.98\times10^{-2}$ | $6.6\times10^{-2}$ | $2.4\times10^{-8}$ | $1.7\times10^{8}$ |
| 2 | $7.8\times10^{-5}$ | $2.1\times10^{6}$ | $1.27\times10^{-2}$ | $1.2\times10^{-1}$ | $5.7\times10^{-8}$ | $4.1\times10^{8}$ |
| 3 | $3.9\times10^{-5}$ | $1.1\times10^{6}$ | $7.22\times10^{-3}$ | $6.6\times10^{-2}$ | $5.9\times10^{-8}$ | $4.3\times10^{8}$ |
| 4 | $2.0\times10^{-5}$ | $5.6\times10^{5}$ | $3.99\times10^{-3}$ | $3.4\times10^{-2}$ | $6.0\times10^{-8}$ | $4.3\times10^{8}$ |
| 5 | $9.8\times10^{-6}$ | $2.9\times10^{5}$ | $1.72\times10^{-3}$ | $1.8\times10^{-2}$ | $6.1\times10^{-8}$ | $4.5\times10^{8}$ |
| 6 | $4.9\times10^{-6}$ | $1.5\times10^{5}$ | $8.55\times10^{-4}$ | $9.2\times10^{-3}$ | $6.3\times10^{-8}$ | $4.5\times10^{8}$ |
| 7 | $2.4\times10^{-6}$ | $8.8\times10^{4}$ | $6.66\times10^{-4}$ | $4.2\times10^{-3}$ | $4.8\times10^{-8}$ | $5.4\times10^{8}$ |
| 8 | $1.2\times10^{-6}$ | $3.4\times10^{4}$ | $1.00\times10^{-4}$ | $2.0\times10^{-3}$ | $6.0\times10^{-8}$ | $4.2\times10^{8}$ |
| 9 | $6.1\times10^{-7}$ | $1.6\times10^{4}$ | $-9.53\times10^{-6}$ | $1.2\times10^{-3}$ | $7.6\times10^{-8}$ | $4.0\times10^{8}$ |
| 10 | $3.1\times10^{-7}$ | $1.0\times10^{3}$ | $-4.07\times10^{-4}$ | $8.7\times10^{-5}$ | $8.7\times10^{-8}$ | $4.9\times10^{7}$ |
| $\sum$ | | | $9.95\times10^{-1}$ | | $6.0\times10^{-7}$ | $3.8\times10^{9}$ |

Table 58: $\varepsilon = 0.05$, $\Delta t_1 = 7.81 \times 10^{-5}$

| $\ell$ | $\Delta t_\ell$ | $P_\ell$ | $\mathbb{E}[\hat{F}_\ell - \hat{F}_{\ell-1}]$ | $\mathbb{V}[\hat{F}_\ell - \hat{F}_{\ell-1}]$ | $\mathbb{V}[\hat{Y}_\ell]$ | $P_\ell C_\ell$ |
|---|---|---|---|---|---|---|
| 0 | $5.0\times10^{-1}$ | $8.2\times10^{8}$ | $9.97\times10^{-1}$ | $2.0\times10^{0}$ | $2.4\times10^{-9}$ | $1.6\times10^{7}$ |
| 1 | $7.8\times10^{-5}$ | $1.9\times10^{6}$ | $-1.69\times10^{-2}$ | $6.7\times10^{-2}$ | $3.6\times10^{-8}$ | $2.4\times10^{8}$ |
| 2 | $3.9\times10^{-5}$ | $1.1\times10^{6}$ | $6.78\times10^{-3}$ | $6.6\times10^{-2}$ | $6.2\times10^{-8}$ | $4.1\times10^{8}$ |
| 3 | $2.0\times10^{-5}$ | $5.5\times10^{5}$ | $3.87\times10^{-3}$ | $3.4\times10^{-2}$ | $6.3\times10^{-8}$ | $4.2\times10^{8}$ |
| 4 | $9.8\times10^{-6}$ | $2.7\times10^{5}$ | $2.01\times10^{-3}$ | $1.7\times10^{-2}$ | $6.3\times10^{-8}$ | $4.2\times10^{8}$ |
| 5 | $4.9\times10^{-6}$ | $1.4\times10^{5}$ | $9.06\times10^{-4}$ | $8.6\times10^{-3}$ | $6.3\times10^{-8}$ | $4.2\times10^{8}$ |
| 6 | $2.4\times10^{-6}$ | $6.9\times10^{4}$ | $3.04\times10^{-4}$ | $4.4\times10^{-3}$ | $6.3\times10^{-8}$ | $4.2\times10^{8}$ |
| 7 | $1.2\times10^{-6}$ | $4.0\times10^{4}$ | $2.05\times10^{-4}$ | $2.6\times10^{-3}$ | $6.5\times10^{-8}$ | $5.0\times10^{8}$ |
| 8 | $6.1\times10^{-7}$ | $2.1\times10^{4}$ | $-3.71\times10^{-5}$ | $9.4\times10^{-4}$ | $4.4\times10^{-8}$ | $5.2\times10^{8}$ |
| 9 | $3.1\times10^{-7}$ | $1.0\times10^{3}$ | $5.98\times10^{-5}$ | $3.4\times10^{-4}$ | $3.4\times10^{-7}$ | $4.9\times10^{7}$ |
| $\sum$ | | | $9.95\times10^{-1}$ | | $8.0\times10^{-7}$ | $3.4\times10^{9}$ |

Table 59: $\varepsilon = 0.05$, $\Delta t_1 = 3.91 \times 10^{-5}$

| $\ell$ | $\Delta t_\ell$ | $P_\ell$ | $\mathbb{E}[\hat{F}_\ell - \hat{F}_{\ell-1}]$ | $\mathbb{V}[\hat{F}_\ell - \hat{F}_{\ell-1}]$ | $\mathbb{V}[\hat{Y}_\ell]$ | $P_\ell C_\ell$ |
|---|---|---|---|---|---|---|
| 0 | $5.0\times10^{-1}$ | $6.7\times10^{8}$ | $9.98\times10^{-1}$ | $2.0\times10^{0}$ | $3.0\times10^{-9}$ | $1.3\times10^{7}$ |
| 1 | $3.9\times10^{-5}$ | $1.1\times10^{6}$ | $-9.75\times10^{-3}$ | $6.7\times10^{-2}$ | $6.2\times10^{-8}$ | $2.8\times10^{8}$ |
| 2 | $2.0\times10^{-5}$ | $4.5\times10^{5}$ | $3.53\times10^{-3}$ | $3.4\times10^{-2}$ | $7.6\times10^{-8}$ | $3.5\times10^{8}$ |
| 3 | $9.8\times10^{-6}$ | $2.3\times10^{5}$ | $2.13\times10^{-3}$ | $1.7\times10^{-2}$ | $7.6\times10^{-8}$ | $3.5\times10^{8}$ |
| 4 | $4.9\times10^{-6}$ | $1.1\times10^{5}$ | $9.84\times10^{-4}$ | $8.7\times10^{-3}$ | $7.7\times10^{-8}$ | $3.5\times10^{8}$ |
| 5 | $2.4\times10^{-6}$ | $5.5\times10^{4}$ | $5.14\times10^{-4}$ | $4.1\times10^{-3}$ | $7.5\times10^{-8}$ | $3.4\times10^{8}$ |
| 6 | $1.2\times10^{-6}$ | $3.2\times10^{4}$ | $4.07\times10^{-4}$ | $2.4\times10^{-3}$ | $7.6\times10^{-8}$ | $3.9\times10^{8}$ |
| 7 | $6.1\times10^{-7}$ | $9.1\times10^{3}$ | $4.32\times10^{-5}$ | $6.2\times10^{-4}$ | $6.8\times10^{-8}$ | $2.2\times10^{8}$ |
| 8 | $3.1\times10^{-7}$ | $1.0\times10^{3}$ | $1.45\times10^{-5}$ | $1.0\times10^{-4}$ | $1.0\times10^{-7}$ | $4.9\times10^{7}$ |
| $\sum$ | | | $9.95\times10^{-1}$ | | $6.2\times10^{-7}$ | $2.3\times10^{9}$ |

Table 60: $\varepsilon = 0.05$, $\Delta t_1 = 1.95 \times 10^{-5}$

| $\ell$ | $\Delta t_\ell$ | $P_\ell$ | $\mathbb{E}[\hat{F}_\ell - \hat{F}_{\ell-1}]$ | $\mathbb{V}[\hat{F}_\ell - \hat{F}_{\ell-1}]$ | $\mathbb{V}[\hat{Y}_\ell]$ | $P_\ell C_\ell$ |
|---|---|---|---|---|---|---|
| 0 | $5.0\times10^{-1}$ | $6.2\times10^{8}$ | $9.98\times10^{-1}$ | $2.0\times10^{0}$ | $3.2\times10^{-9}$ | $1.2\times10^{7}$ |
| 1 | $2.0\times10^{-5}$ | $7.2\times10^{5}$ | $-6.39\times10^{-3}$ | $6.8\times10^{-2}$ | $9.4\times10^{-8}$ | $3.7\times10^{8}$ |
| 2 | $9.8\times10^{-6}$ | $2.1\times10^{5}$ | $1.84\times10^{-3}$ | $1.8\times10^{-2}$ | $8.3\times10^{-8}$ | $3.3\times10^{8}$ |
| 3 | $4.9\times10^{-6}$ | $1.1\times10^{5}$ | $8.18\times10^{-4}$ | $8.9\times10^{-3}$ | $8.4\times10^{-8}$ | $3.3\times10^{8}$ |
| 4 | $2.4\times10^{-6}$ | $5.2\times10^{4}$ | $7.12\times10^{-4}$ | $4.6\times10^{-3}$ | $8.9\times10^{-8}$ | $3.2\times10^{8}$ |
| 5 | $1.2\times10^{-6}$ | $2.4\times10^{4}$ | $6.51\times10^{-4}$ | $1.8\times10^{-3}$ | $7.7\times10^{-8}$ | $2.9\times10^{8}$ |
| 6 | $6.1\times10^{-7}$ | $1.3\times10^{4}$ | $-1.80\times10^{-4}$ | $9.3\times10^{-4}$ | $7.4\times10^{-8}$ | $3.1\times10^{8}$ |
| 7 | $3.1\times10^{-7}$ | $1.0\times10^{3}$ | $5.89\times10^{-4}$ | $2.3\times10^{-4}$ | $2.3\times10^{-7}$ | $4.9\times10^{7}$ |
| $\sum$ | | | $9.96\times10^{-1}$ | | $7.3\times10^{-7}$ | $2.0\times10^{9}$ |

Table 61: $\varepsilon = 0.05$, $\Delta t_1 = 9.77 \times 10^{-6}$

| $\ell$ | $\Delta t_\ell$ | $P_\ell$ | $\mathbb{E}[\hat{F}_\ell - \hat{F}_{\ell-1}]$ | $\mathbb{V}[\hat{F}_\ell - \hat{F}_{\ell-1}]$ | $\mathbb{V}[\hat{Y}_\ell]$ | $P_\ell C_\ell$ |
|---|---|---|---|---|---|---|
| 0 | $5.0\times10^{-1}$ | $4.7\times10^{8}$ | $9.98\times10^{-1}$ | $2.0\times10^{0}$ | $4.2\times10^{-9}$ | $9.5\times10^{6}$ |
| 1 | $9.8\times10^{-6}$ | $3.9\times10^{5}$ | $-4.31\times10^{-3}$ | $6.9\times10^{-2}$ | $1.8\times10^{-7}$ | $4.0\times10^{8}$ |
| 2 | $4.9\times10^{-6}$ | $7.7\times10^{4}$ | $7.33\times10^{-4}$ | $8.0\times10^{-3}$ | $1.0\times10^{-7}$ | $2.4\times10^{8}$ |
| 3 | $2.4\times10^{-6}$ | $3.9\times10^{4}$ | $3.57\times10^{-4}$ | $4.5\times10^{-3}$ | $1.1\times10^{-7}$ | $2.4\times10^{8}$ |
| 4 | $1.2\times10^{-6}$ | $2.0\times10^{4}$ | $3.85\times10^{-4}$ | $2.2\times10^{-3}$ | $1.1\times10^{-7}$ | $2.4\times10^{8}$ |
| 5 | $6.1\times10^{-7}$ | $1.0\times10^{3}$ | $-4.33\times10^{-4}$ | $2.8\times10^{-4}$ | $2.8\times10^{-7}$ | $2.5\times10^{7}$ |
| $\sum$ | | | $9.94\times10^{-1}$ | | $7.9\times10^{-7}$ | $1.2\times10^{9}$ |

Table 62: $\varepsilon = 0.05$, $\Delta t_1 = 4.88 \times 10^{-6}$

| $\ell$ | $\Delta t_\ell$ | $P_\ell$ | $\mathbb{E}[\hat{F}_\ell - \hat{F}_{\ell-1}]$ | $\mathbb{V}[\hat{F}_\ell - \hat{F}_{\ell-1}]$ | $\mathbb{V}[\hat{Y}_\ell]$ | $P_\ell C_\ell$ |
|---|---|---|---|---|---|---|
| 0 | $5.0\times10^{-1}$ | $4.0\times10^{8}$ | $9.97\times10^{-1}$ | $2.0\times10^{0}$ | $4.9\times10^{-9}$ | $8.1\times10^{6}$ |
| 1 | $4.9\times10^{-6}$ | $2.4\times10^{5}$ | $-4.49\times10^{-3}$ | $6.9\times10^{-2}$ | $2.9\times10^{-7}$ | $4.8\times10^{8}$ |
| 2 | $2.4\times10^{-6}$ | $3.5\times10^{4}$ | $6.10\times10^{-4}$ | $4.6\times10^{-3}$ | $1.3\times10^{-7}$ | $2.1\times10^{8}$ |
| 3 | $1.2\times10^{-6}$ | $9.8\times10^{3}$ | $-2.22\times10^{-4}$ | $1.7\times10^{-3}$ | $1.7\times10^{-7}$ | $1.2\times10^{8}$ |
| 4 | $6.1\times10^{-7}$ | $1.0\times10^{3}$ | $2.63\times10^{-4}$ | $3.2\times10^{-4}$ | $3.2\times10^{-7}$ | $2.5\times10^{7}$ |
| $\sum$ | | | $9.94\times10^{-1}$ | | $9.2\times10^{-7}$ | $8.5\times10^{8}$ |

Table 63: $\varepsilon = 0.05$, $\Delta t_1 = 2.44 \times 10^{-6}$

| $\ell$ | $\Delta t_\ell$ | $P_\ell$ | $\mathbb{E}[\hat{F}_\ell - \hat{F}_{\ell-1}]$ | $\mathbb{V}[\hat{F}_\ell - \hat{F}_{\ell-1}]$ | $\mathbb{V}[\hat{Y}_\ell]$ | $P_\ell C_\ell$ |
|---|---|---|---|---|---|---|
| 0 | $5.0\times10^{-1}$ | $7.8\times10^{8}$ | $9.97\times10^{-1}$ | $2.0\times10^{0}$ | $2.5\times10^{-9}$ | $1.6\times10^{7}$ |
| 1 | $2.4\times10^{-6}$ | $3.2\times10^{5}$ | $-2.92\times10^{-3}$ | $6.8\times10^{-2}$ | $2.1\times10^{-7}$ | $1.3\times10^{9}$ |
| 2 | $1.2\times10^{-6}$ | $3.1\times10^{4}$ | $7.88\times10^{-4}$ | $2.1\times10^{-3}$ | $6.6\times10^{-8}$ | $3.8\times10^{8}$ |
| 3 | $6.1\times10^{-7}$ | $1.9\times10^{4}$ | $-6.26\times10^{-5}$ | $9.8\times10^{-4}$ | $5.3\times10^{-8}$ | $4.6\times10^{8}$ |
| 4 | $3.1\times10^{-7}$ | $2.0\times10^{4}$ | $1.00\times10^{-4}$ | $7.2\times10^{-4}$ | $3.6\times10^{-8}$ | $9.7\times10^{8}$ |
| 5 | $1.5\times10^{-7}$ | $1.0\times10^{3}$ | $2.29\times10^{-4}$ | $4.4\times10^{-5}$ | $4.4\times10^{-8}$ | $9.8\times10^{7}$ |
| $\sum$ | | | $9.96\times10^{-1}$ | | $4.1\times10^{-7}$ | $3.2\times10^{9}$ |

Table 64: $\varepsilon = 0.05$, $\Delta t_1 = 1.22 \times 10^{-6}$

| $\ell$ | $\Delta t_\ell$ | $P_\ell$ | $\mathbb{E}[\hat{F}_\ell - \hat{F}_{\ell-1}]$ | $\mathbb{V}[\hat{F}_\ell - \hat{F}_{\ell-1}]$ | $\mathbb{V}[\hat{Y}_\ell]$ | $P_\ell C_\ell$ |
|---|---|---|---|---|---|---|
| 0 | $5.0\times10^{-1}$ | $6.1\times10^{8}$ | $9.98\times10^{-1}$ | $2.0\times10^{0}$ | $3.3\times10^{-9}$ | $1.2\times10^{7}$ |
| 1 | $1.2\times10^{-6}$ | $1.8\times10^{5}$ | $-3.33\times10^{-3}$ | $6.8\times10^{-2}$ | $3.9\times10^{-7}$ | $1.4\times10^{9}$ |
| 2 | $6.1\times10^{-7}$ | $9.1\times10^{3}$ | $-2.14\times10^{-5}$ | $7.8\times10^{-4}$ | $8.6\times10^{-8}$ | $2.2\times10^{8}$ |
| 3 | $3.1\times10^{-7}$ | $3.8\times10^{3}$ | $-4.39\times10^{-5}$ | $3.1\times10^{-4}$ | $8.3\times10^{-8}$ | $1.9\times10^{8}$ |
| 4 | $1.5\times10^{-7}$ | $1.0\times10^{3}$ | $3.05\times10^{-4}$ | $1.7\times10^{-4}$ | $1.7\times10^{-7}$ | $9.8\times10^{7}$ |
| $\sum$ | | | $9.94\times10^{-1}$ | | $7.2\times10^{-7}$ | $2.0\times10^{9}$ |

# 2 Tables corresponding with Figure 5

## 2.1 Term-by-term correlation, $\varepsilon = 0.5$

Table 65: $\varepsilon = 0.5$, $\Delta t_1 = 2.50 \times 10^{-1}$

| $\ell$ | $\Delta t_\ell$ | $P_\ell$ | $\mathbb{E}[\hat{F}_\ell - \hat{F}_{\ell-1}]$ | $\mathbb{V}[\hat{F}_\ell - \hat{F}_{\ell-1}]$ | $\mathbb{V}[\hat{Y}_\ell]$ | $P_\ell C_\ell$ |
|---|---|---|---|---|---|---|
| 0 | $5.0\times10^{-1}$ | $3.8\times10^{7}$ | $7.78\times10^{-1}$ | $1.2\times10^{0}$ | $3.2\times10^{-8}$ | $7.5\times10^{5}$ |
| 1 | $2.5\times10^{-1}$ | $8.5\times10^{6}$ | $-9.03\times10^{-2}$ | $1.9\times10^{-1}$ | $2.2\times10^{-8}$ | $5.1\times10^{5}$ |
| 2 | $1.2\times10^{-1}$ | $5.8\times10^{6}$ | $-6.60\times10^{-2}$ | $1.7\times10^{-1}$ | $3.0\times10^{-8}$ | $7.0\times10^{5}$ |
| 3 | $6.2\times10^{-2}$ | $3.6\times10^{6}$ | $-3.43\times10^{-2}$ | $1.3\times10^{-1}$ | $3.7\times10^{-8}$ | $8.6\times10^{5}$ |
| 4 | $3.1\times10^{-2}$ | $2.0\times10^{6}$ | $-1.35\times10^{-2}$ | $8.6\times10^{-2}$ | $4.2\times10^{-8}$ | $9.8\times10^{5}$ |
| 5 | $1.6\times10^{-2}$ | $1.1\times10^{6}$ | $-4.15\times10^{-3}$ | $5.0\times10^{-2}$ | $4.5\times10^{-8}$ | $1.1\times10^{6}$ |
| 6 | $7.8\times10^{-3}$ | $5.8\times10^{5}$ | $-1.54\times10^{-3}$ | $2.8\times10^{-2}$ | $4.8\times10^{-8}$ | $1.1\times10^{6}$ |
| 7 | $3.9\times10^{-3}$ | $2.9\times10^{5}$ | $-2.67\times10^{-5}$ | $1.3\times10^{-2}$ | $4.7\times10^{-8}$ | $1.1\times10^{6}$ |
| 8 | $2.0\times10^{-3}$ | $2.1\times10^{5}$ | $-1.14\times10^{-5}$ | $7.8\times10^{-3}$ | $3.7\times10^{-8}$ | $1.6\times10^{6}$ |
| 9 | $9.8\times10^{-4}$ | $7.5\times10^{4}$ | $-2.54\times10^{-4}$ | $3.8\times10^{-3}$ | $5.0\times10^{-8}$ | $1.2\times10^{6}$ |
| 10 | $4.9\times10^{-4}$ | $5.1\times10^{4}$ | $3.95\times10^{-4}$ | $2.4\times10^{-3}$ | $4.6\times10^{-8}$ | $1.6\times10^{6}$ |
| 11 | $2.4\times10^{-4}$ | $1.2\times10^{4}$ | $1.44\times10^{-4}$ | $6.5\times10^{-4}$ | $5.4\times10^{-8}$ | $7.3\times10^{5}$ |
| 12 | $1.2\times10^{-4}$ | $1.0\times10^{3}$ | $-3.44\times10^{-4}$ | $1.9\times10^{-3}$ | $1.9\times10^{-6}$ | $1.2\times10^{5}$ |
| $\sum$ | | | $5.68\times10^{-1}$ | | $2.4\times10^{-6}$ | $1.2\times10^{7}$ |

Table 66: $\varepsilon = 0.5$, $\Delta t_1 = 1.25 \times 10^{-1}$

| $\ell$ | $\Delta t_\ell$ | $P_\ell$ | $\mathbb{E}[\hat{F}_\ell - \hat{F}_{\ell-1}]$ | $\mathbb{V}[\hat{F}_\ell - \hat{F}_{\ell-1}]$ | $\mathbb{V}[\hat{Y}_\ell]$ | $P_\ell C_\ell$ |
|---|---|---|---|---|---|---|
| 0 | $5.0\times10^{-1}$ | $3.5\times10^{7}$ | $7.78\times10^{-1}$ | $1.2\times10^{0}$ | $3.4\times10^{-8}$ | $7.0\times10^{5}$ |
| 1 | $1.2\times10^{-1}$ | $1.0\times10^{7}$ | $-1.56\times10^{-1}$ | $5.4\times10^{-1}$ | $5.1\times10^{-8}$ | $1.0\times10^{6}$ |
| 2 | $6.2\times10^{-2}$ | $3.4\times10^{6}$ | $-3.40\times10^{-2}$ | $1.3\times10^{-1}$ | $3.9\times10^{-8}$ | $8.1\times10^{5}$ |
| 3 | $3.1\times10^{-2}$ | $1.9\times10^{6}$ | $-1.32\times10^{-2}$ | $8.6\times10^{-2}$ | $4.5\times10^{-8}$ | $9.2\times10^{5}$ |
| 4 | $1.6\times10^{-2}$ | $1.0\times10^{6}$ | $-4.07\times10^{-3}$ | $5.0\times10^{-2}$ | $4.8\times10^{-8}$ | $9.9\times10^{5}$ |
| 5 | $7.8\times10^{-3}$ | $5.5\times10^{5}$ | $-1.57\times10^{-3}$ | $2.8\times10^{-2}$ | $5.2\times10^{-8}$ | $1.1\times10^{6}$ |
| 6 | $3.9\times10^{-3}$ | $2.7\times10^{5}$ | $-4.59\times10^{-4}$ | $1.4\times10^{-2}$ | $5.2\times10^{-8}$ | $1.0\times10^{6}$ |
| 7 | $2.0\times10^{-3}$ | $1.3\times10^{5}$ | $2.09\times10^{-5}$ | $6.7\times10^{-3}$ | $5.1\times10^{-8}$ | $1.0\times10^{6}$ |
| 8 | $9.8\times10^{-4}$ | $9.9\times10^{4}$ | $5.14\times10^{-5}$ | $3.8\times10^{-3}$ | $3.8\times10^{-8}$ | $1.5\times10^{6}$ |
| 9 | $4.9\times10^{-4}$ | $2.9\times10^{4}$ | $-1.13\times10^{-4}$ | $1.2\times10^{-3}$ | $4.0\times10^{-8}$ | $9.0\times10^{5}$ |
| 10 | $2.4\times10^{-4}$ | $1.1\times10^{4}$ | $-2.33\times10^{-5}$ | $1.1\times10^{-3}$ | $1.0\times10^{-7}$ | $6.8\times10^{5}$ |
| 11 | $1.2\times10^{-4}$ | $1.0\times10^{3}$ | $-1.05\times10^{-4}$ | $1.6\times10^{-4}$ | $1.6\times10^{-7}$ | $1.2\times10^{5}$ |
| $\sum$ | | | $5.68\times10^{-1}$ | | $7.1\times10^{-7}$ | $1.1\times10^{7}$ |

Table 67: $\varepsilon = 0.5$, $\Delta t_1 = 6.25 \times 10^{-2}$

| $\ell$ | $\Delta t_\ell$ | $P_\ell$ | $\mathbb{E}[\hat{F}_\ell - \hat{F}_{\ell-1}]$ | $\mathbb{V}[\hat{F}_\ell - \hat{F}_{\ell-1}]$ | $\mathbb{V}[\hat{Y}_\ell]$ | $P_\ell C_\ell$ |
|---|---|---|---|---|---|---|
| 0 | $5.0\times10^{-1}$ | $2.5\times10^{7}$ | $7.78\times10^{-1}$ | $1.2\times10^{0}$ | $4.8\times10^{-8}$ | $5.1\times10^{5}$ |
| 1 | $6.2\times10^{-2}$ | $7.4\times10^{6}$ | $-1.90\times10^{-1}$ | $9.3\times10^{-1}$ | $1.3\times10^{-7}$ | $1.3\times10^{6}$ |
| 2 | $3.1\times10^{-2}$ | $1.4\times10^{6}$ | $-1.35\times10^{-2}$ | $8.7\times10^{-2}$ | $6.3\times10^{-8}$ | $6.7\times10^{5}$ |
| 3 | $1.6\times10^{-2}$ | $7.4\times10^{5}$ | $-4.26\times10^{-3}$ | $5.0\times10^{-2}$ | $6.8\times10^{-8}$ | $7.1\times10^{5}$ |
| 4 | $7.8\times10^{-3}$ | $4.3\times10^{5}$ | $-1.07\times10^{-3}$ | $2.8\times10^{-2}$ | $6.4\times10^{-8}$ | $8.2\times10^{5}$ |
| 5 | $3.9\times10^{-3}$ | $2.0\times10^{5}$ | $1.50\times10^{-5}$ | $1.4\times10^{-2}$ | $7.1\times10^{-8}$ | $7.5\times10^{5}$ |
| 6 | $2.0\times10^{-3}$ | $7.5\times10^{4}$ | $-1.46\times10^{-4}$ | $7.4\times10^{-3}$ | $9.9\times10^{-8}$ | $5.8\times10^{5}$ |
| 7 | $9.8\times10^{-4}$ | $1.0\times10^{3}$ | $-3.77\times10^{-4}$ | $1.7\times10^{-3}$ | $1.7\times10^{-6}$ | $1.5\times10^{4}$ |
| $\sum$ | | | $5.68\times10^{-1}$ | | $2.3\times10^{-6}$ | $5.4\times10^{6}$ |

Table 68: $\varepsilon = 0.5$, $\Delta t_1 = 3.12 \times 10^{-2}$

| $\ell$ | $\Delta t_\ell$ | $P_\ell$ | $\mathbb{E}[\hat{F}_\ell - \hat{F}_{\ell-1}]$ | $\mathbb{V}[\hat{F}_\ell - \hat{F}_{\ell-1}]$ | $\mathbb{V}[\hat{Y}_\ell]$ | $P_\ell C_\ell$ |
|---|---|---|---|---|---|---|
| 0 | $5.0\times10^{-1}$ | $2.6\times10^{7}$ | $7.77\times10^{-1}$ | $1.2\times10^{0}$ | $4.6\times10^{-8}$ | $5.3\times10^{5}$ |
| 1 | $3.1\times10^{-2}$ | $6.5\times10^{6}$ | $-2.04\times10^{-1}$ | $1.3\times10^{0}$ | $1.9\times10^{-7}$ | $2.2\times10^{6}$ |
| 2 | $1.6\times10^{-2}$ | $7.8\times10^{5}$ | $-4.65\times10^{-3}$ | $5.1\times10^{-2}$ | $6.5\times10^{-8}$ | $7.5\times10^{5}$ |
| 3 | $7.8\times10^{-3}$ | $4.0\times10^{5}$ | $-1.59\times10^{-3}$ | $2.6\times10^{-2}$ | $6.6\times10^{-8}$ | $7.6\times10^{5}$ |
| 4 | $3.9\times10^{-3}$ | $2.1\times10^{5}$ | $-3.72\times10^{-4}$ | $1.3\times10^{-2}$ | $6.6\times10^{-8}$ | $7.9\times10^{5}$ |
| 5 | $2.0\times10^{-3}$ | $9.5\times10^{4}$ | $4.86\times10^{-6}$ | $6.8\times10^{-3}$ | $7.2\times10^{-8}$ | $7.3\times10^{5}$ |
| 6 | $9.8\times10^{-4}$ | $1.0\times10^{3}$ | $1.71\times10^{-4}$ | $5.3\times10^{-3}$ | $5.3\times10^{-6}$ | $1.5\times10^{4}$ |
| $\sum$ | | | $5.67\times10^{-1}$ | | $5.8\times10^{-6}$ | $5.8\times10^{6}$ |

Table 69: $\varepsilon = 0.5$, $\Delta t_1 = 1.56 \times 10^{-2}$

| $\ell$ | $\Delta t_\ell$ | $P_\ell$ | $\mathbb{E}[\hat{F}_\ell - \hat{F}_{\ell-1}]$ | $\mathbb{V}[\hat{F}_\ell - \hat{F}_{\ell-1}]$ | $\mathbb{V}[\hat{Y}_\ell]$ | $P_\ell C_\ell$ |
|---|---|---|---|---|---|---|
| 0 | $5.0\times10^{-1}$ | $3.5\times10^{7}$ | $7.78\times10^{-1}$ | $1.2\times10^{0}$ | $3.5\times10^{-8}$ | $6.9\times10^{5}$ |
| 1 | $1.6\times10^{-2}$ | $6.7\times10^{6}$ | $-2.08\times10^{-1}$ | $1.5\times10^{0}$ | $2.2\times10^{-7}$ | $4.4\times10^{6}$ |
| 2 | $7.8\times10^{-3}$ | $5.3\times10^{5}$ | $-1.02\times10^{-3}$ | $2.7\times10^{-2}$ | $5.1\times10^{-8}$ | $1.0\times10^{6}$ |
| 3 | $3.9\times10^{-3}$ | $2.7\times10^{5}$ | $-4.81\times10^{-4}$ | $1.4\times10^{-2}$ | $5.2\times10^{-8}$ | $1.0\times10^{6}$ |
| 4 | $2.0\times10^{-3}$ | $1.4\times10^{5}$ | $-1.83\times10^{-4}$ | $7.7\times10^{-3}$ | $5.4\times10^{-8}$ | $1.1\times10^{6}$ |
| 5 | $9.8\times10^{-4}$ | $6.8\times10^{4}$ | $-1.58\times10^{-4}$ | $3.4\times10^{-3}$ | $5.0\times10^{-8}$ | $1.0\times10^{6}$ |
| 6 | $4.9\times10^{-4}$ | $2.2\times10^{4}$ | $5.74\times10^{-4}$ | $3.2\times10^{-3}$ | $1.5\times10^{-7}$ | $6.6\times10^{5}$ |
| 7 | $2.4\times10^{-4}$ | $1.0\times10^{3}$ | $-3.31\times10^{-5}$ | $3.3\times10^{-4}$ | $3.3\times10^{-7}$ | $6.1\times10^{4}$ |
| $\sum$ | | | $5.69\times10^{-1}$ | | $9.4\times10^{-7}$ | $1.0\times10^{7}$ |

Table 70: $\varepsilon = 0.5$, $\Delta t_1 = 7.81 \times 10^{-3}$

| $\ell$ | $\Delta t_\ell$ | $P_\ell$ | $\mathbb{E}[\hat{F}_\ell - \hat{F}_{\ell-1}]$ | $\mathbb{V}[\hat{F}_\ell - \hat{F}_{\ell-1}]$ | $\mathbb{V}[\hat{Y}_\ell]$ | $P_\ell C_\ell$ |
|---|---|---|---|---|---|---|
| 0 | $5.0\times10^{-1}$ | $4.4\times10^{7}$ | $7.78\times10^{-1}$ | $1.2\times10^{0}$ | $2.8\times10^{-8}$ | $8.8\times10^{5}$ |
| 1 | $7.8\times10^{-3}$ | $6.3\times10^{6}$ | $-2.10\times10^{-1}$ | $1.6\times10^{0}$ | $2.6\times10^{-7}$ | $8.2\times10^{6}$ |
| 2 | $3.9\times10^{-3}$ | $3.4\times10^{5}$ | $-4.71\times10^{-4}$ | $1.4\times10^{-2}$ | $4.2\times10^{-8}$ | $1.3\times10^{6}$ |
| 3 | $2.0\times10^{-3}$ | $1.8\times10^{5}$ | $2.69\times10^{-4}$ | $7.3\times10^{-3}$ | $4.2\times10^{-8}$ | $1.4\times10^{6}$ |
| 4 | $9.8\times10^{-4}$ | $8.9\times10^{4}$ | $2.03\times10^{-4}$ | $3.4\times10^{-3}$ | $3.9\times10^{-8}$ | $1.4\times10^{6}$ |
| 5 | $4.9\times10^{-4}$ | $9.1\times10^{4}$ | $5.14\times10^{-5}$ | $1.3\times10^{-3}$ | $1.4\times10^{-8}$ | $2.8\times10^{6}$ |
| 6 | $2.4\times10^{-4}$ | $1.0\times10^{3}$ | $4.54\times10^{-4}$ | $3.3\times10^{-4}$ | $3.3\times10^{-7}$ | $6.1\times10^{4}$ |
| $\sum$ | | | $5.69\times10^{-1}$ | | $7.6\times10^{-7}$ | $1.6\times10^{7}$ |

Table 71: $\varepsilon = 0.5$, $\Delta t_1 = 3.91 \times 10^{-3}$

| $\ell$ | $\Delta t_\ell$ | $P_\ell$ | $\mathbb{E}[\hat{F}_\ell - \hat{F}_{\ell-1}]$ | $\mathbb{V}[\hat{F}_\ell - \hat{F}_{\ell-1}]$ | $\mathbb{V}[\hat{Y}_\ell]$ | $P_\ell C_\ell$ |
|---|---|---|---|---|---|---|
| 0 | $5.0\times10^{-1}$ | $4.3\times10^{7}$ | $7.78\times10^{-1}$ | $1.2\times10^{0}$ | $2.8\times10^{-8}$ | $8.7\times10^{5}$ |
| 1 | $3.9\times10^{-3}$ | $4.6\times10^{6}$ | $-2.11\times10^{-1}$ | $1.7\times10^{0}$ | $3.8\times10^{-7}$ | $1.2\times10^{7}$ |
| 2 | $2.0\times10^{-3}$ | $3.7\times10^{5}$ | $-1.63\times10^{-4}$ | $6.6\times10^{-3}$ | $1.8\times10^{-8}$ | $2.9\times10^{6}$ |
| 3 | $9.8\times10^{-4}$ | $4.9\times10^{4}$ | $3.92\times10^{-5}$ | $3.8\times10^{-3}$ | $7.7\times10^{-8}$ | $7.6\times10^{5}$ |
| 4 | $4.9\times10^{-4}$ | $1.0\times10^{3}$ | $-1.56\times10^{-4}$ | $8.2\times10^{-4}$ | $8.2\times10^{-7}$ | $3.1\times10^{4}$ |
| $\sum$ | | | $5.67\times10^{-1}$ | | $1.3\times10^{-6}$ | $1.6\times10^{7}$ |

Table 72: $\varepsilon = 0.5$, $\Delta t_1 = 1.95 \times 10^{-3}$

| $\ell$ | $\Delta t_\ell$ | $P_\ell$ | $\mathbb{E}[\hat{F}_\ell - \hat{F}_{\ell-1}]$ | $\mathbb{V}[\hat{F}_\ell - \hat{F}_{\ell-1}]$ | $\mathbb{V}[\hat{Y}_\ell]$ | $P_\ell C_\ell$ |
|---|---|---|---|---|---|---|
| 0 | $5.0\times10^{-1}$ | $6.5\times10^{7}$ | $7.78\times10^{-1}$ | $1.2\times10^{0}$ | $1.9\times10^{-8}$ | $1.3\times10^{6}$ |
| 1 | $2.0\times10^{-3}$ | $4.9\times10^{6}$ | $-2.10\times10^{-1}$ | $1.8\times10^{0}$ | $3.6\times10^{-7}$ | $2.5\times10^{7}$ |
| 2 | $9.8\times10^{-4}$ | $1.3\times10^{5}$ | $-6.95\times10^{-5}$ | $3.7\times10^{-3}$ | $2.8\times10^{-8}$ | $2.0\times10^{6}$ |
| 3 | $4.9\times10^{-4}$ | $7.4\times10^{4}$ | $3.12\times10^{-5}$ | $2.7\times10^{-3}$ | $3.6\times10^{-8}$ | $2.3\times10^{6}$ |
| 4 | $2.4\times10^{-4}$ | $2.5\times10^{4}$ | $-4.04\times10^{-5}$ | $4.9\times10^{-4}$ | $2.0\times10^{-8}$ | $1.5\times10^{6}$ |
| 5 | $1.2\times10^{-4}$ | $2.0\times10^{4}$ | $1.59\times10^{-4}$ | $3.1\times10^{-4}$ | $1.5\times10^{-8}$ | $2.5\times10^{6}$ |
| 6 | $6.1\times10^{-5}$ | $1.0\times10^{3}$ | $2.65\times10^{-4}$ | $1.1\times10^{-4}$ | $1.1\times10^{-7}$ | $2.5\times10^{5}$ |
| $\sum$ | | | $5.68\times10^{-1}$ | | $5.9\times10^{-7}$ | $3.5\times10^{7}$ |

Table 73: $\varepsilon = 0.5$, $\Delta t_1 = 9.77 \times 10^{-4}$

| $\ell$ | $\Delta t_\ell$ | $P_\ell$ | $\mathbb{E}[\hat{F}_\ell - \hat{F}_{\ell-1}]$ | $\mathbb{V}[\hat{F}_\ell - \hat{F}_{\ell-1}]$ | $\mathbb{V}[\hat{Y}_\ell]$ | $P_\ell C_\ell$ |
|---|---|---|---|---|---|---|
| 0 | $5.0\times10^{-1}$ | $7.5\times10^{7}$ | $7.78\times10^{-1}$ | $1.2\times10^{0}$ | $1.6\times10^{-8}$ | $1.5\times10^{6}$ |
| 1 | $9.8\times10^{-4}$ | $4.1\times10^{6}$ | $-2.10\times10^{-1}$ | $1.8\times10^{0}$ | $4.5\times10^{-7}$ | $4.2\times10^{7}$ |
| 2 | $4.9\times10^{-4}$ | $6.7\times10^{4}$ | $2.05\times10^{-5}$ | $1.4\times10^{-3}$ | $2.0\times10^{-8}$ | $2.0\times10^{6}$ |
| 3 | $2.4\times10^{-4}$ | $2.5\times10^{4}$ | $-2.54\times10^{-5}$ | $4.2\times10^{-4}$ | $1.7\times10^{-8}$ | $1.5\times10^{6}$ |
| 4 | $1.2\times10^{-4}$ | $1.0\times10^{3}$ | $-1.43\times10^{-4}$ | $1.9\times10^{-4}$ | $1.9\times10^{-7}$ | $1.2\times10^{5}$ |
| $\sum$ | | | $5.68\times10^{-1}$ | | $6.9\times10^{-7}$ | $4.7\times10^{7}$ |

Table 74: $\varepsilon = 0.5$, $\Delta t_1 = 4.88 \times 10^{-4}$

| $\ell$ | $\Delta t_\ell$ | $P_\ell$ | $\mathbb{E}[\hat{F}_\ell - \hat{F}_{\ell-1}]$ | $\mathbb{V}[\hat{F}_\ell - \hat{F}_{\ell-1}]$ | $\mathbb{V}[\hat{Y}_\ell]$ | $P_\ell C_\ell$ |
|---|---|---|---|---|---|---|
| 0 | $5.0\times10^{-1}$ | $1.1\times10^{8}$ | $7.78\times10^{-1}$ | $1.2\times10^{0}$ | $1.1\times10^{-8}$ | $2.2\times10^{6}$ |
| 1 | $4.9\times10^{-4}$ | $4.4\times10^{6}$ | $-2.09\times10^{-1}$ | $1.8\times10^{0}$ | $4.2\times10^{-7}$ | $9.1\times10^{7}$ |
| 2 | $2.4\times10^{-4}$ | $1.1\times10^{5}$ | $-2.27\times10^{-4}$ | $1.7\times10^{-3}$ | $1.6\times10^{-8}$ | $6.8\times10^{6}$ |
| 3 | $1.2\times10^{-4}$ | $1.6\times10^{4}$ | $-1.25\times10^{-5}$ | $1.9\times10^{-4}$ | $1.2\times10^{-8}$ | $2.0\times10^{6}$ |
| 4 | $6.1\times10^{-5}$ | $1.0\times10^{3}$ | $1.52\times10^{-4}$ | $8.4\times10^{-5}$ | $8.4\times10^{-8}$ | $2.5\times10^{5}$ |
| $\sum$ | | | $5.68\times10^{-1}$ | | $5.4\times10^{-7}$ | $1.0\times10^{8}$ |

## 2.2 Term-by-term correlation, $\varepsilon = 0.1$

Table 75: $\varepsilon = 0.1$, $\Delta t_1 = 1.00 \times 10^{-2}$

| $\ell$ | $\Delta t_\ell$ | $P_\ell$ | $\mathbb{E}[\hat{F}_\ell - \hat{F}_{\ell-1}]$ | $\mathbb{V}[\hat{F}_\ell - \hat{F}_{\ell-1}]$ | $\mathbb{V}[\hat{Y}_\ell]$ | $P_\ell C_\ell$ |
|---|---|---|---|---|---|---|
| 0 | $5.0\times10^{-1}$ | $5.4\times10^{8}$ | $9.90\times10^{-1}$ | $2.0\times10^{0}$ | $3.7\times10^{-9}$ | $1.1\times10^{7}$ |
| 1 | $1.0\times10^{-2}$ | $6.5\times10^{7}$ | $-1.25\times10^{-1}$ | $1.5\times10^{0}$ | $2.3\times10^{-8}$ | $6.6\times10^{7}$ |
| 2 | $5.0\times10^{-3}$ | $2.1\times10^{7}$ | $1.07\times10^{-2}$ | $4.7\times10^{-1}$ | $2.2\times10^{-8}$ | $6.4\times10^{7}$ |
| 3 | $2.5\times10^{-3}$ | $1.5\times10^{7}$ | $2.84\times10^{-2}$ | $4.4\times10^{-1}$ | $3.0\times10^{-8}$ | $8.8\times10^{7}$ |
| 4 | $1.3\times10^{-3}$ | $9.0\times10^{6}$ | $2.90\times10^{-2}$ | $3.3\times10^{-1}$ | $3.7\times10^{-8}$ | $1.1\times10^{8}$ |
| 5 | $6.3\times10^{-4}$ | $5.1\times10^{6}$ | $2.08\times10^{-2}$ | $2.1\times10^{-1}$ | $4.2\times10^{-8}$ | $1.2\times10^{8}$ |
| 6 | $3.1\times10^{-4}$ | $2.7\times10^{6}$ | $1.23\times10^{-2}$ | $1.2\times10^{-1}$ | $4.5\times10^{-8}$ | $1.3\times10^{8}$ |
| 7 | $1.6\times10^{-4}$ | $1.4\times10^{6}$ | $6.56\times10^{-3}$ | $6.5\times10^{-2}$ | $4.6\times10^{-8}$ | $1.4\times10^{8}$ |
| 8 | $7.8\times10^{-5}$ | $7.3\times10^{5}$ | $3.55\times10^{-3}$ | $3.4\times10^{-2}$ | $4.7\times10^{-8}$ | $1.4\times10^{8}$ |
| 9 | $3.9\times10^{-5}$ | $3.6\times10^{5}$ | $1.79\times10^{-3}$ | $1.7\times10^{-2}$ | $4.7\times10^{-8}$ | $1.4\times10^{8}$ |
| 10 | $2.0\times10^{-5}$ | $2.0\times10^{5}$ | $1.27\times10^{-3}$ | $9.9\times10^{-3}$ | $5.1\times10^{-8}$ | $1.5\times10^{8}$ |
| 11 | $9.8\times10^{-6}$ | $9.3\times10^{4}$ | $6.62\times10^{-4}$ | $4.5\times10^{-3}$ | $4.8\times10^{-8}$ | $1.4\times10^{8}$ |
| 12 | $4.9\times10^{-6}$ | $3.7\times10^{4}$ | $1.76\times10^{-4}$ | $1.6\times10^{-3}$ | $4.2\times10^{-8}$ | $1.1\times10^{8}$ |
| 13 | $2.4\times10^{-6}$ | $9.6\times10^{3}$ | $-2.58\times10^{-4}$ | $1.7\times10^{-3}$ | $1.7\times10^{-7}$ | $5.9\times10^{7}$ |
| 14 | $1.2\times10^{-6}$ | $1.0\times10^{3}$ | $2.01\times10^{-4}$ | $1.6\times10^{-4}$ | $1.6\times10^{-7}$ | $1.2\times10^{7}$ |
| $\sum$ | | | $9.80\times10^{-1}$ | | $8.1\times10^{-7}$ | $1.5\times10^{9}$ |

Table 76: $\varepsilon = 0.1$, $\Delta t_1 = 5.00 \times 10^{-3}$

| $\ell$ | $\Delta t_\ell$ | $P_\ell$ | $\mathbb{E}[\hat{F}_\ell - \hat{F}_{\ell-1}]$ | $\mathbb{V}[\hat{F}_\ell - \hat{F}_{\ell-1}]$ | $\mathbb{V}[\hat{Y}_\ell]$ | $P_\ell C_\ell$ |
|---|---|---|---|---|---|---|
| 0 | $5.0\times10^{-1}$ | $8.3\times10^{8}$ | $9.90\times10^{-1}$ | $2.0\times10^{0}$ | $2.3\times10^{-9}$ | $1.7\times10^{7}$ |
| 1 | $5.0\times10^{-3}$ | $8.8\times10^{7}$ | $-1.15\times10^{-1}$ | $2.2\times10^{0}$ | $2.5\times10^{-8}$ | $1.8\times10^{8}$ |
| 2 | $2.5\times10^{-3}$ | $2.3\times10^{7}$ | $2.84\times10^{-2}$ | $4.4\times10^{-1}$ | $1.9\times10^{-8}$ | $1.4\times10^{8}$ |
| 3 | $1.3\times10^{-3}$ | $1.4\times10^{7}$ | $2.87\times10^{-2}$ | $3.3\times10^{-1}$ | $2.4\times10^{-8}$ | $1.7\times10^{8}$ |
| 4 | $6.3\times10^{-4}$ | $7.9\times10^{6}$ | $2.05\times10^{-2}$ | $2.1\times10^{-1}$ | $2.7\times10^{-8}$ | $1.9\times10^{8}$ |
| 5 | $3.1\times10^{-4}$ | $4.2\times10^{6}$ | $1.28\times10^{-2}$ | $1.2\times10^{-1}$ | $2.9\times10^{-8}$ | $2.0\times10^{8}$ |
| 6 | $1.6\times10^{-4}$ | $2.2\times10^{6}$ | $6.75\times10^{-3}$ | $6.6\times10^{-2}$ | $3.0\times10^{-8}$ | $2.1\times10^{8}$ |
| 7 | $7.8\times10^{-5}$ | $1.1\times10^{6}$ | $3.88\times10^{-3}$ | $3.3\times10^{-2}$ | $3.0\times10^{-8}$ | $2.1\times10^{8}$ |
| 8 | $3.9\times10^{-5}$ | $5.7\times10^{5}$ | $1.80\times10^{-3}$ | $1.8\times10^{-2}$ | $3.1\times10^{-8}$ | $2.2\times10^{8}$ |
| 9 | $2.0\times10^{-5}$ | $3.1\times10^{5}$ | $9.39\times10^{-4}$ | $1.0\times10^{-2}$ | $3.2\times10^{-8}$ | $2.4\times10^{8}$ |
| 10 | $9.8\times10^{-6}$ | $1.3\times10^{5}$ | $7.01\times10^{-4}$ | $3.9\times10^{-3}$ | $2.9\times10^{-8}$ | $2.1\times10^{8}$ |
| 11 | $4.9\times10^{-6}$ | $7.5\times10^{4}$ | $7.74\times10^{-5}$ | $2.3\times10^{-3}$ | $3.0\times10^{-8}$ | $2.3\times10^{8}$ |
| 12 | $2.4\times10^{-6}$ | $3.1\times10^{4}$ | $1.22\times10^{-4}$ | $7.4\times10^{-4}$ | $2.4\times10^{-8}$ | $1.9\times10^{8}$ |
| 13 | $1.2\times10^{-6}$ | $7.5\times10^{3}$ | $-1.23\times10^{-4}$ | $1.1\times10^{-4}$ | $1.5\times10^{-8}$ | $9.3\times10^{7}$ |
| 14 | $6.1\times10^{-7}$ | $4.3\times10^{4}$ | $-3.18\times10^{-5}$ | $3.5\times10^{-4}$ | $8.2\times10^{-9}$ | $1.1\times10^{9}$ |
| 15 | $3.1\times10^{-7}$ | $1.0\times10^{3}$ | $-3.46\times10^{-4}$ | $2.3\times10^{-4}$ | $2.3\times10^{-7}$ | $4.9\times10^{7}$ |
| $\sum$ | | | $9.80\times10^{-1}$ | | $5.9\times10^{-7}$ | $3.6\times10^{9}$ |

Table 77: $\varepsilon = 0.1$, $\Delta t_1 = 2.50 \times 10^{-3}$

| $\ell$ | $\Delta t_\ell$ | $P_\ell$ | $\mathbb{E}[\hat{F}_\ell - \hat{F}_{\ell-1}]$ | $\mathbb{V}[\hat{F}_\ell - \hat{F}_{\ell-1}]$ | $\mathbb{V}[\hat{Y}_\ell]$ | $P_\ell C_\ell$ |
|---|---|---|---|---|---|---|
| 0 | $5.0\times10^{-1}$ | $5.2\times10^{8}$ | $9.90\times10^{-1}$ | $2.0\times10^{0}$ | $3.8\times10^{-9}$ | $1.0\times10^{7}$ |
| 1 | $2.5\times10^{-3}$ | $4.4\times10^{7}$ | $-8.63\times10^{-2}$ | $2.8\times10^{0}$ | $6.4\times10^{-8}$ | $1.8\times10^{8}$ |
| 2 | $1.3\times10^{-3}$ | $8.7\times10^{6}$ | $2.89\times10^{-2}$ | $3.3\times10^{-1}$ | $3.8\times10^{-8}$ | $1.0\times10^{8}$ |
| 3 | $6.3\times10^{-4}$ | $5.0\times10^{6}$ | $2.13\times10^{-2}$ | $2.1\times10^{-1}$ | $4.3\times10^{-8}$ | $1.2\times10^{8}$ |
| 4 | $3.1\times10^{-4}$ | $2.6\times10^{6}$ | $1.22\times10^{-2}$ | $1.2\times10^{-1}$ | $4.6\times10^{-8}$ | $1.3\times10^{8}$ |
| 5 | $1.6\times10^{-4}$ | $1.4\times10^{6}$ | $6.84\times10^{-3}$ | $6.5\times10^{-2}$ | $4.8\times10^{-8}$ | $1.3\times10^{8}$ |
| 6 | $7.8\times10^{-5}$ | $6.9\times10^{5}$ | $3.66\times10^{-3}$ | $3.3\times10^{-2}$ | $4.8\times10^{-8}$ | $1.3\times10^{8}$ |
| 7 | $3.9\times10^{-5}$ | $3.5\times10^{5}$ | $1.82\times10^{-3}$ | $1.8\times10^{-2}$ | $5.0\times10^{-8}$ | $1.4\times10^{8}$ |
| 8 | $2.0\times10^{-5}$ | $1.8\times10^{5}$ | $1.09\times10^{-3}$ | $8.8\times10^{-3}$ | $5.0\times10^{-8}$ | $1.4\times10^{8}$ |
| 9 | $9.8\times10^{-6}$ | $8.3\times10^{4}$ | $2.40\times10^{-4}$ | $3.7\times10^{-3}$ | $4.5\times10^{-8}$ | $1.3\times10^{8}$ |
| 10 | $4.9\times10^{-6}$ | $3.8\times10^{4}$ | $5.69\times10^{-4}$ | $1.7\times10^{-3}$ | $4.4\times10^{-8}$ | $1.2\times10^{8}$ |
| 11 | $2.4\times10^{-6}$ | $9.7\times10^{3}$ | $1.13\times10^{-4}$ | $3.7\times10^{-4}$ | $3.8\times10^{-8}$ | $6.0\times10^{7}$ |
| 12 | $1.2\times10^{-6}$ | $1.0\times10^{3}$ | $-6.77\times10^{-6}$ | $5.1\times10^{-4}$ | $5.1\times10^{-7}$ | $1.2\times10^{7}$ |
| $\sum$ | | | $9.80\times10^{-1}$ | | $1.0\times10^{-6}$ | $1.4\times10^{9}$ |

Table 78: $\varepsilon = 0.1$, $\Delta t_1 = 1.25 \times 10^{-3}$

| $\ell$ | $\Delta t_\ell$ | $P_\ell$ | $\mathbb{E}[\hat{F}_\ell - \hat{F}_{\ell-1}]$ | $\mathbb{V}[\hat{F}_\ell - \hat{F}_{\ell-1}]$ | $\mathbb{V}[\hat{Y}_\ell]$ | $P_\ell C_\ell$ |
|---|---|---|---|---|---|---|
| 0 | $5.0\times10^{-1}$ | $5.9\times10^{8}$ | $9.90\times10^{-1}$ | $2.0\times10^{0}$ | $3.3\times10^{-9}$ | $1.2\times10^{7}$ |
| 1 | $1.3\times10^{-3}$ | $3.8\times10^{7}$ | $-5.74\times10^{-2}$ | $3.3\times10^{0}$ | $8.6\times10^{-8}$ | $3.1\times10^{8}$ |
| 2 | $6.3\times10^{-4}$ | $5.6\times10^{6}$ | $2.09\times10^{-2}$ | $2.1\times10^{-1}$ | $3.8\times10^{-8}$ | $1.4\times10^{8}$ |
| 3 | $3.1\times10^{-4}$ | $3.0\times10^{6}$ | $1.24\times10^{-2}$ | $1.2\times10^{-1}$ | $4.1\times10^{-8}$ | $1.5\times10^{8}$ |
| 4 | $1.6\times10^{-4}$ | $1.6\times10^{6}$ | $6.91\times10^{-3}$ | $6.5\times10^{-2}$ | $4.2\times10^{-8}$ | $1.5\times10^{8}$ |
| 5 | $7.8\times10^{-5}$ | $8.0\times10^{5}$ | $3.57\times10^{-3}$ | $3.5\times10^{-2}$ | $4.3\times10^{-8}$ | $1.5\times10^{8}$ |
| 6 | $3.9\times10^{-5}$ | $4.0\times10^{5}$ | $1.83\times10^{-3}$ | $1.8\times10^{-2}$ | $4.4\times10^{-8}$ | $1.5\times10^{8}$ |
| 7 | $2.0\times10^{-5}$ | $2.0\times10^{5}$ | $8.59\times10^{-4}$ | $8.8\times10^{-3}$ | $4.4\times10^{-8}$ | $1.5\times10^{8}$ |
| 8 | $9.8\times10^{-6}$ | $9.6\times10^{4}$ | $2.04\times10^{-4}$ | $3.9\times10^{-3}$ | $4.0\times10^{-8}$ | $1.5\times10^{8}$ |
| 9 | $4.9\times10^{-6}$ | $4.4\times10^{4}$ | $6.06\times10^{-4}$ | $1.7\times10^{-3}$ | $3.9\times10^{-8}$ | $1.4\times10^{8}$ |
| 10 | $2.4\times10^{-6}$ | $2.1\times10^{4}$ | $1.80\times10^{-4}$ | $5.7\times10^{-4}$ | $2.7\times10^{-8}$ | $1.3\times10^{8}$ |
| 11 | $1.2\times10^{-6}$ | $1.3\times10^{4}$ | $-1.71\times10^{-4}$ | $5.8\times10^{-4}$ | $4.5\times10^{-8}$ | $1.6\times10^{8}$ |
| 12 | $6.1\times10^{-7}$ | $1.0\times10^{3}$ | $2.86\times10^{-4}$ | $5.3\times10^{-5}$ | $5.3\times10^{-8}$ | $2.5\times10^{7}$ |
| $\sum$ | | | $9.80\times10^{-1}$ | | $5.4\times10^{-7}$ | $1.8\times10^{9}$ |

Table 79: $\varepsilon = 0.1$, $\Delta t_1 = 6.25 \times 10^{-4}$

| $\ell$ | $\Delta t_\ell$ | $P_\ell$ | $\mathbb{E}[\hat{F}_\ell - \hat{F}_{\ell-1}]$ | $\mathbb{V}[\hat{F}_\ell - \hat{F}_{\ell-1}]$ | $\mathbb{V}[\hat{Y}_\ell]$ | $P_\ell C_\ell$ |
|---|---|---|---|---|---|---|
| 0 | $5.0\times10^{-1}$ | $4.9\times10^{8}$ | $9.90\times10^{-1}$ | $2.0\times10^{0}$ | $4.0\times10^{-9}$ | $9.8\times10^{6}$ |
| 1 | $6.3\times10^{-4}$ | $2.3\times10^{7}$ | $-3.64\times10^{-2}$ | $3.6\times10^{0}$ | $1.5\times10^{-7}$ | $3.8\times10^{8}$ |
| 2 | $3.1\times10^{-4}$ | $2.5\times10^{6}$ | $1.24\times10^{-2}$ | $1.2\times10^{-1}$ | $4.9\times10^{-8}$ | $1.2\times10^{8}$ |
| 3 | $1.6\times10^{-4}$ | $1.3\times10^{6}$ | $7.06\times10^{-3}$ | $6.6\times10^{-2}$ | $5.1\times10^{-8}$ | $1.2\times10^{8}$ |
| 4 | $7.8\times10^{-5}$ | $6.6\times10^{5}$ | $3.64\times10^{-3}$ | $3.4\times10^{-2}$ | $5.1\times10^{-8}$ | $1.3\times10^{8}$ |
| 5 | $3.9\times10^{-5}$ | $3.3\times10^{5}$ | $1.95\times10^{-3}$ | $1.8\times10^{-2}$ | $5.3\times10^{-8}$ | $1.3\times10^{8}$ |
| 6 | $2.0\times10^{-5}$ | $1.7\times10^{5}$ | $7.65\times10^{-4}$ | $9.2\times10^{-3}$ | $5.4\times10^{-8}$ | $1.3\times10^{8}$ |
| 7 | $9.8\times10^{-6}$ | $8.4\times10^{4}$ | $5.51\times10^{-4}$ | $4.5\times10^{-3}$ | $5.3\times10^{-8}$ | $1.3\times10^{8}$ |
| 8 | $4.9\times10^{-6}$ | $2.5\times10^{4}$ | $-1.13\times10^{-5}$ | $2.0\times10^{-3}$ | $8.0\times10^{-8}$ | $7.6\times10^{7}$ |
| 9 | $2.4\times10^{-6}$ | $1.0\times10^{3}$ | $5.37\times10^{-4}$ | $3.8\times10^{-4}$ | $3.8\times10^{-7}$ | $6.1\times10^{6}$ |
| $\sum$ | | | $9.80\times10^{-1}$ | | $9.3\times10^{-7}$ | $1.2\times10^{9}$ |

Table 80: $\varepsilon = 0.1$, $\Delta t_1 = 3.13 \times 10^{-4}$

| $\ell$ | $\Delta t_\ell$ | $P_\ell$ | $\mathbb{E}[\hat{F}_\ell - \hat{F}_{\ell-1}]$ | $\mathbb{V}[\hat{F}_\ell - \hat{F}_{\ell-1}]$ | $\mathbb{V}[\hat{Y}_\ell]$ | $P_\ell C_\ell$ |
|---|---|---|---|---|---|---|
| 0 | $5.0\times10^{-1}$ | $5.2\times10^{8}$ | $9.90\times10^{-1}$ | $2.0\times10^{0}$ | $3.8\times10^{-9}$ | $1.0\times10^{7}$ |
| 1 | $3.1\times10^{-4}$ | $1.8\times10^{7}$ | $-2.41\times10^{-2}$ | $3.8\times10^{0}$ | $2.1\times10^{-7}$ | $5.8\times10^{8}$ |
| 2 | $1.6\times10^{-4}$ | $1.4\times10^{6}$ | $6.90\times10^{-3}$ | $6.7\times10^{-2}$ | $4.8\times10^{-8}$ | $1.3\times10^{8}$ |
| 3 | $7.8\times10^{-5}$ | $7.0\times10^{5}$ | $3.49\times10^{-3}$ | $3.4\times10^{-2}$ | $4.9\times10^{-8}$ | $1.3\times10^{8}$ |
| 4 | $3.9\times10^{-5}$ | $3.5\times10^{5}$ | $1.71\times10^{-3}$ | $1.7\times10^{-2}$ | $4.8\times10^{-8}$ | $1.3\times10^{8}$ |
| 5 | $2.0\times10^{-5}$ | $1.7\times10^{5}$ | $8.32\times10^{-4}$ | $8.3\times10^{-3}$ | $4.9\times10^{-8}$ | $1.3\times10^{8}$ |
| 6 | $9.8\times10^{-6}$ | $1.0\times10^{5}$ | $2.90\times10^{-4}$ | $5.4\times10^{-3}$ | $5.4\times10^{-8}$ | $1.6\times10^{8}$ |
| 7 | $4.9\times10^{-6}$ | $3.0\times10^{4}$ | $-2.66\times10^{-4}$ | $3.3\times10^{-3}$ | $1.1\times10^{-7}$ | $9.3\times10^{7}$ |
| 8 | $2.4\times10^{-6}$ | $1.0\times10^{3}$ | $3.52\times10^{-4}$ | $1.8\times10^{-4}$ | $1.8\times10^{-7}$ | $6.1\times10^{6}$ |
| $\sum$ | | | $9.79\times10^{-1}$ | | $7.5\times10^{-7}$ | $1.4\times10^{9}$ |

Table 81: $\varepsilon = 0.1$, $\Delta t_1 = 1.56 \times 10^{-4}$

| $\ell$ | $\Delta t_\ell$ | $P_\ell$ | $\mathbb{E}[\hat{F}_\ell - \hat{F}_{\ell-1}]$ | $\mathbb{V}[\hat{F}_\ell - \hat{F}_{\ell-1}]$ | $\mathbb{V}[\hat{Y}_\ell]$ | $P_\ell C_\ell$ |
|---|---|---|---|---|---|---|
| 0 | $5.0\times10^{-1}$ | $6.0\times10^{8}$ | $9.90\times10^{-1}$ | $2.0\times10^{0}$ | $3.2\times10^{-9}$ | $1.2\times10^{7}$ |
| 1 | $1.6\times10^{-4}$ | $1.5\times10^{7}$ | $-1.69\times10^{-2}$ | $3.9\times10^{0}$ | $2.6\times10^{-7}$ | $9.6\times10^{8}$ |
| 2 | $7.8\times10^{-5}$ | $8.2\times10^{5}$ | $3.22\times10^{-3}$ | $3.5\times10^{-2}$ | $4.2\times10^{-8}$ | $1.6\times10^{8}$ |
| 3 | $3.9\times10^{-5}$ | $4.2\times10^{5}$ | $1.54\times10^{-3}$ | $1.8\times10^{-2}$ | $4.2\times10^{-8}$ | $1.6\times10^{8}$ |
| 4 | $2.0\times10^{-5}$ | $2.1\times10^{5}$ | $1.11\times10^{-3}$ | $8.3\times10^{-3}$ | $4.0\times10^{-8}$ | $1.6\times10^{8}$ |
| 5 | $9.8\times10^{-6}$ | $1.1\times10^{5}$ | $5.58\times10^{-4}$ | $4.4\times10^{-3}$ | $4.1\times10^{-8}$ | $1.6\times10^{8}$ |
| 6 | $4.9\times10^{-6}$ | $8.1\times10^{4}$ | $2.63\times10^{-5}$ | $2.2\times10^{-3}$ | $2.7\times10^{-8}$ | $2.5\times10^{8}$ |
| 7 | $2.4\times10^{-6}$ | $1.0\times10^{3}$ | $-3.50\times10^{-4}$ | $4.5\times10^{-4}$ | $4.5\times10^{-7}$ | $6.1\times10^{6}$ |
| $\sum$ | | | $9.79\times10^{-1}$ | | $9.1\times10^{-7}$ | $1.9\times10^{9}$ |

Table 82: $\varepsilon = 0.1$, $\Delta t_1 = 7.81 \times 10^{-5}$

| $\ell$ | $\Delta t_\ell$ | $P_\ell$ | $\mathbb{E}[\hat{F}_\ell - \hat{F}_{\ell-1}]$ | $\mathbb{V}[\hat{F}_\ell - \hat{F}_{\ell-1}]$ | $\mathbb{V}[\hat{Y}_\ell]$ | $P_\ell C_\ell$ |
|---|---|---|---|---|---|---|
| 0 | $5.0\times10^{-1}$ | $7.6\times10^{8}$ | $9.90\times10^{-1}$ | $2.0\times10^{0}$ | $2.6\times10^{-9}$ | $1.5\times10^{7}$ |
| 1 | $7.8\times10^{-5}$ | $1.4\times10^{7}$ | $-1.37\times10^{-2}$ | $3.9\times10^{0}$ | $2.9\times10^{-7}$ | $1.7\times10^{9}$ |
| 2 | $3.9\times10^{-5}$ | $5.3\times10^{5}$ | $1.78\times10^{-3}$ | $1.8\times10^{-2}$ | $3.4\times10^{-8}$ | $2.0\times10^{8}$ |
| 3 | $2.0\times10^{-5}$ | $2.6\times10^{5}$ | $1.18\times10^{-3}$ | $8.6\times10^{-3}$ | $3.4\times10^{-8}$ | $2.0\times10^{8}$ |
| 4 | $9.8\times10^{-6}$ | $1.2\times10^{5}$ | $4.15\times10^{-4}$ | $3.9\times10^{-3}$ | $3.2\times10^{-8}$ | $1.9\times10^{8}$ |
| 5 | $4.9\times10^{-6}$ | $7.8\times10^{4}$ | $9.50\times10^{-5}$ | $3.0\times10^{-3}$ | $3.8\times10^{-8}$ | $2.4\times10^{8}$ |
| 6 | $2.4\times10^{-6}$ | $3.5\times10^{4}$ | $-6.71\times10^{-5}$ | $8.7\times10^{-4}$ | $2.5\times10^{-8}$ | $2.1\times10^{8}$ |
| 7 | $1.2\times10^{-6}$ | $1.5\times10^{4}$ | $1.33\times10^{-4}$ | $5.7\times10^{-4}$ | $3.8\times10^{-8}$ | $1.8\times10^{8}$ |
| 8 | $6.1\times10^{-7}$ | $1.0\times10^{3}$ | $-9.98\times10^{-5}$ | $2.0\times10^{-4}$ | $2.0\times10^{-7}$ | $2.5\times10^{7}$ |
| $\sum$ | | | $9.80\times10^{-1}$ | | $7.0\times10^{-7}$ | $3.0\times10^{9}$ |

Table 83: $\varepsilon = 0.1$, $\Delta t_1 = 3.91 \times 10^{-5}$

| $\ell$ | $\Delta t_\ell$ | $P_\ell$ | $\mathbb{E}[\hat{F}_\ell - \hat{F}_{\ell-1}]$ | $\mathbb{V}[\hat{F}_\ell - \hat{F}_{\ell-1}]$ | $\mathbb{V}[\hat{Y}_\ell]$ | $P_\ell C_\ell$ |
|---|---|---|---|---|---|---|
| 0 | $5.0\times10^{-1}$ | $1.1\times10^{9}$ | $9.90\times10^{-1}$ | $2.0\times10^{0}$ | $1.8\times10^{-9}$ | $2.2\times10^{7}$ |
| 1 | $3.9\times10^{-5}$ | $1.4\times10^{7}$ | $-1.14\times10^{-2}$ | $4.0\times10^{0}$ | $2.8\times10^{-7}$ | $3.6\times10^{9}$ |
| 2 | $2.0\times10^{-5}$ | $3.8\times10^{5}$ | $7.00\times10^{-4}$ | $8.6\times10^{-3}$ | $2.3\times10^{-8}$ | $2.9\times10^{8}$ |
| 3 | $9.8\times10^{-6}$ | $1.8\times10^{5}$ | $5.11\times10^{-4}$ | $4.4\times10^{-3}$ | $2.4\times10^{-8}$ | $2.8\times10^{8}$ |
| 4 | $4.9\times10^{-6}$ | $1.1\times10^{5}$ | $2.01\times10^{-4}$ | $2.8\times10^{-3}$ | $2.6\times10^{-8}$ | $3.3\times10^{8}$ |
| 5 | $2.4\times10^{-6}$ | $3.0\times10^{5}$ | $5.02\times10^{-5}$ | $1.3\times10^{-3}$ | $4.3\times10^{-9}$ | $1.8\times10^{9}$ |
| 6 | $1.2\times10^{-6}$ | $3.6\times10^{4}$ | $1.72\times10^{-4}$ | $2.6\times10^{-4}$ | $7.3\times10^{-9}$ | $4.4\times10^{8}$ |
| 7 | $6.1\times10^{-7}$ | $1.0\times10^{3}$ | $7.53\times10^{-5}$ | $6.9\times10^{-5}$ | $6.9\times10^{-8}$ | $2.5\times10^{7}$ |
| $\sum$ | | | $9.80\times10^{-1}$ | | $4.4\times10^{-7}$ | $6.8\times10^{9}$ |

Table 84: $\varepsilon = 0.1$, $\Delta t_1 = 1.95 \times 10^{-5}$

| $\ell$ | $\Delta t_\ell$ | $P_\ell$ | $\mathbb{E}[\hat{F}_\ell - \hat{F}_{\ell-1}]$ | $\mathbb{V}[\hat{F}_\ell - \hat{F}_{\ell-1}]$ | $\mathbb{V}[\hat{Y}_\ell]$ | $P_\ell C_\ell$ |
|---|---|---|---|---|---|---|
| 0 | $5.0\times10^{-1}$ | $1.0\times10^{9}$ | $9.90\times10^{-1}$ | $2.0\times10^{0}$ | $1.9\times10^{-9}$ | $2.1\times10^{7}$ |
| 1 | $2.0\times10^{-5}$ | $9.2\times10^{6}$ | $-1.07\times10^{-2}$ | $4.0\times10^{0}$ | $4.3\times10^{-7}$ | $4.7\times10^{9}$ |
| 2 | $9.8\times10^{-6}$ | $4.6\times10^{5}$ | $5.12\times10^{-4}$ | $4.6\times10^{-3}$ | $9.9\times10^{-9}$ | $7.1\times10^{8}$ |
| 3 | $4.9\times10^{-6}$ | $7.7\times10^{4}$ | $1.12\times10^{-4}$ | $2.1\times10^{-3}$ | $2.8\times10^{-8}$ | $2.4\times10^{8}$ |
| 4 | $2.4\times10^{-6}$ | $1.9\times10^{4}$ | $-5.22\times10^{-5}$ | $3.0\times10^{-3}$ | $1.6\times10^{-7}$ | $1.2\times10^{8}$ |
| 5 | $1.2\times10^{-6}$ | $1.0\times10^{3}$ | $-3.85\times10^{-4}$ | $9.6\times10^{-4}$ | $9.6\times10^{-7}$ | $1.2\times10^{7}$ |
| $\sum$ | | | $9.79\times10^{-1}$ | | $1.6\times10^{-6}$ | $5.8\times10^{9}$ |

## 2.3 Term-by-term correlation, $\varepsilon = 0.05$

Table 85: $\varepsilon = 0.05$, $\Delta t_1 = 2.50 \times 10^{-3}$

| $\ell$ | $\Delta t_\ell$ | $P_\ell$ | $\mathbb{E}[\hat{F}_\ell - \hat{F}_{\ell-1}]$ | $\mathbb{V}[\hat{F}_\ell - \hat{F}_{\ell-1}]$ | $\mathbb{V}[\hat{Y}_\ell]$ | $P_\ell C_\ell$ |
|---|---|---|---|---|---|---|
| 0 | $5.0\times10^{-1}$ | $1.2\times10^{9}$ | $9.97\times10^{-1}$ | $2.0\times10^{0}$ | $1.6\times10^{-9}$ | $2.5\times10^{7}$ |
| 1 | $2.5\times10^{-3}$ | $7.6\times10^{7}$ | $-1.25\times10^{-1}$ | $1.5\times10^{0}$ | $2.0\times10^{-8}$ | $3.0\times10^{8}$ |
| 2 | $1.3\times10^{-3}$ | $2.5\times10^{7}$ | $1.32\times10^{-2}$ | $4.8\times10^{-1}$ | $1.9\times10^{-8}$ | $2.9\times10^{8}$ |
| 3 | $6.3\times10^{-4}$ | $1.7\times10^{7}$ | $3.04\times10^{-2}$ | $4.5\times10^{-1}$ | $2.7\times10^{-8}$ | $4.0\times10^{8}$ |
| 4 | $3.1\times10^{-4}$ | $1.0\times10^{7}$ | $2.99\times10^{-2}$ | $3.4\times10^{-1}$ | $3.3\times10^{-8}$ | $5.0\times10^{8}$ |
| 5 | $1.6\times10^{-4}$ | $5.9\times10^{6}$ | $2.11\times10^{-2}$ | $2.2\times10^{-1}$ | $3.7\times10^{-8}$ | $5.6\times10^{8}$ |
| 6 | $7.8\times10^{-5}$ | $3.1\times10^{6}$ | $1.28\times10^{-2}$ | $1.2\times10^{-1}$ | $4.0\times10^{-8}$ | $6.0\times10^{8}$ |
| 7 | $3.9\times10^{-5}$ | $1.6\times10^{6}$ | $6.83\times10^{-3}$ | $6.8\times10^{-2}$ | $4.1\times10^{-8}$ | $6.3\times10^{8}$ |
| 8 | $2.0\times10^{-5}$ | $8.3\times10^{5}$ | $3.84\times10^{-3}$ | $3.5\times10^{-2}$ | $4.2\times10^{-8}$ | $6.4\times10^{8}$ |
| 9 | $9.8\times10^{-6}$ | $4.2\times10^{5}$ | $2.34\times10^{-3}$ | $1.7\times10^{-2}$ | $4.2\times10^{-8}$ | $6.4\times10^{8}$ |
| 10 | $4.9\times10^{-6}$ | $2.1\times10^{5}$ | $8.10\times10^{-4}$ | $8.7\times10^{-3}$ | $4.2\times10^{-8}$ | $6.4\times10^{8}$ |
| 11 | $2.4\times10^{-6}$ | $1.1\times10^{5}$ | $3.77\times10^{-4}$ | $4.9\times10^{-3}$ | $4.4\times10^{-8}$ | $6.8\times10^{8}$ |
| 12 | $1.2\times10^{-6}$ | $5.2\times10^{4}$ | $6.03\times10^{-4}$ | $2.1\times10^{-3}$ | $4.0\times10^{-8}$ | $6.4\times10^{8}$ |
| 13 | $6.1\times10^{-7}$ | $4.2\times10^{4}$ | $2.84\times10^{-4}$ | $1.3\times10^{-3}$ | $3.0\times10^{-8}$ | $1.0\times10^{9}$ |
| 14 | $3.1\times10^{-7}$ | $1.0\times10^{3}$ | $2.33\times10^{-5}$ | $5.1\times10^{-4}$ | $5.1\times10^{-7}$ | $4.9\times10^{7}$ |
| $\sum$ | | | $9.95\times10^{-1}$ | | $9.6\times10^{-7}$ | $7.6\times10^{9}$ |

Table 86: $\varepsilon = 0.05$, $\Delta t_1 = 1.25 \times 10^{-3}$

| $\ell$ | $\Delta t_\ell$ | $P_\ell$ | $\mathbb{E}[\hat{F}_\ell - \hat{F}_{\ell-1}]$ | $\mathbb{V}[\hat{F}_\ell - \hat{F}_{\ell-1}]$ | $\mathbb{V}[\hat{Y}_\ell]$ | $P_\ell C_\ell$ |
|---|---|---|---|---|---|---|
| 0 | $5.0\times10^{-1}$ | $1.1\times10^{9}$ | $9.97\times10^{-1}$ | $2.0\times10^{0}$ | $1.8\times10^{-9}$ | $2.2\times10^{7}$ |
| 1 | $1.3\times10^{-3}$ | $5.9\times10^{7}$ | $-1.12\times10^{-1}$ | $2.2\times10^{0}$ | $3.8\times10^{-8}$ | $4.7\times10^{8}$ |
| 2 | $6.3\times10^{-4}$ | $1.5\times10^{7}$ | $3.06\times10^{-2}$ | $4.5\times10^{-1}$ | $2.9\times10^{-8}$ | $3.7\times10^{8}$ |
| 3 | $3.1\times10^{-4}$ | $9.4\times10^{6}$ | $2.99\times10^{-2}$ | $3.4\times10^{-1}$ | $3.6\times10^{-8}$ | $4.5\times10^{8}$ |
| 4 | $1.6\times10^{-4}$ | $5.3\times10^{6}$ | $2.18\times10^{-2}$ | $2.2\times10^{-1}$ | $4.1\times10^{-8}$ | $5.1\times10^{8}$ |
| 5 | $7.8\times10^{-5}$ | $2.9\times10^{6}$ | $1.30\times10^{-2}$ | $1.3\times10^{-1}$ | $4.4\times10^{-8}$ | $5.5\times10^{8}$ |
| 6 | $3.9\times10^{-5}$ | $1.5\times10^{6}$ | $6.74\times10^{-3}$ | $6.7\times10^{-2}$ | $4.6\times10^{-8}$ | $5.7\times10^{8}$ |
| 7 | $2.0\times10^{-5}$ | $7.5\times10^{5}$ | $3.81\times10^{-3}$ | $3.5\times10^{-2}$ | $4.6\times10^{-8}$ | $5.8\times10^{8}$ |
| 8 | $9.8\times10^{-6}$ | $3.8\times10^{5}$ | $2.00\times10^{-3}$ | $1.8\times10^{-2}$ | $4.6\times10^{-8}$ | $5.8\times10^{8}$ |
| 9 | $4.9\times10^{-6}$ | $1.9\times10^{5}$ | $1.18\times10^{-3}$ | $8.6\times10^{-3}$ | $4.6\times10^{-8}$ | $5.7\times10^{8}$ |
| 10 | $2.4\times10^{-6}$ | $9.3\times10^{4}$ | $5.49\times10^{-4}$ | $4.3\times10^{-3}$ | $4.6\times10^{-8}$ | $5.7\times10^{8}$ |
| 11 | $1.2\times10^{-6}$ | $4.5\times10^{4}$ | $6.65\times10^{-4}$ | $1.9\times10^{-3}$ | $4.3\times10^{-8}$ | $5.5\times10^{8}$ |
| 12 | $6.1\times10^{-7}$ | $1.8\times10^{4}$ | $-3.09\times10^{-5}$ | $1.6\times10^{-3}$ | $8.4\times10^{-8}$ | $4.5\times10^{8}$ |
| 13 | $3.1\times10^{-7}$ | $1.0\times10^{3}$ | $-6.66\times10^{-4}$ | $2.1\times10^{-4}$ | $2.1\times10^{-7}$ | $4.9\times10^{7}$ |
| $\sum$ | | | $9.95\times10^{-1}$ | | $7.5\times10^{-7}$ | $6.3\times10^{9}$ |

Table 87: $\varepsilon = 0.05$, $\Delta t_1 = 6.25 \times 10^{-4}$

| $\ell$ | $\Delta t_\ell$ | $P_\ell$ | $\mathbb{E}[\hat{F}_\ell - \hat{F}_{\ell-1}]$ | $\mathbb{V}[\hat{F}_\ell - \hat{F}_{\ell-1}]$ | $\mathbb{V}[\hat{Y}_\ell]$ | $P_\ell C_\ell$ |
|---|---|---|---|---|---|---|
| 0 | $5.0\times10^{-1}$ | $1.0\times10^{9}$ | $9.97\times10^{-1}$ | $2.0\times10^{0}$ | $2.0\times10^{-9}$ | $2.0\times10^{7}$ |
| 1 | $6.3\times10^{-4}$ | $4.2\times10^{7}$ | $-8.16\times10^{-2}$ | $2.9\times10^{0}$ | $6.8\times10^{-8}$ | $6.8\times10^{8}$ |
| 2 | $3.1\times10^{-4}$ | $8.4\times10^{6}$ | $3.02\times10^{-2}$ | $3.4\times10^{-1}$ | $4.0\times10^{-8}$ | $4.0\times10^{8}$ |
| 3 | $1.6\times10^{-4}$ | $4.8\times10^{6}$ | $2.17\times10^{-2}$ | $2.2\times10^{-1}$ | $4.6\times10^{-8}$ | $4.6\times10^{8}$ |
| 4 | $7.8\times10^{-5}$ | $2.6\times10^{6}$ | $1.28\times10^{-2}$ | $1.3\times10^{-1}$ | $4.9\times10^{-8}$ | $4.9\times10^{8}$ |
| 5 | $3.9\times10^{-5}$ | $1.3\times10^{6}$ | $7.02\times10^{-3}$ | $6.8\times10^{-2}$ | $5.1\times10^{-8}$ | $5.1\times10^{8}$ |
| 6 | $2.0\times10^{-5}$ | $6.7\times10^{5}$ | $3.74\times10^{-3}$ | $3.5\times10^{-2}$ | $5.2\times10^{-8}$ | $5.2\times10^{8}$ |
| 7 | $9.8\times10^{-6}$ | $3.4\times10^{5}$ | $2.02\times10^{-3}$ | $1.8\times10^{-2}$ | $5.2\times10^{-8}$ | $5.2\times10^{8}$ |
| 8 | $4.9\times10^{-6}$ | $1.7\times10^{5}$ | $1.20\times10^{-3}$ | $8.5\times10^{-3}$ | $5.0\times10^{-8}$ | $5.2\times10^{8}$ |
| 9 | $2.4\times10^{-6}$ | $8.4\times10^{4}$ | $9.22\times10^{-5}$ | $4.6\times10^{-3}$ | $5.5\times10^{-8}$ | $5.1\times10^{8}$ |
| 10 | $1.2\times10^{-6}$ | $3.0\times10^{4}$ | $7.76\times10^{-5}$ | $2.0\times10^{-3}$ | $6.7\times10^{-8}$ | $3.7\times10^{8}$ |
| 11 | $6.1\times10^{-7}$ | $1.0\times10^{3}$ | $-3.17\times10^{-4}$ | $4.1\times10^{-4}$ | $4.1\times10^{-7}$ | $2.5\times10^{7}$ |
| $\sum$ | | | $9.94\times10^{-1}$ | | $9.5\times10^{-7}$ | $5.0\times10^{9}$ |

Table 88: $\varepsilon = 0.05$, $\Delta t_1 = 3.13 \times 10^{-4}$

| $\ell$ | $\Delta t_\ell$ | $P_\ell$ | $\mathbb{E}[\hat{F}_\ell - \hat{F}_{\ell-1}]$ | $\mathbb{V}[\hat{F}_\ell - \hat{F}_{\ell-1}]$ | $\mathbb{V}[\hat{Y}_\ell]$ | $P_\ell C_\ell$ |
|---|---|---|---|---|---|---|
| 0 | $5.0\times10^{-1}$ | $1.2\times10^{9}$ | $9.98\times10^{-1}$ | $2.0\times10^{0}$ | $1.7\times10^{-9}$ | $2.3\times10^{7}$ |
| 1 | $3.1\times10^{-4}$ | $3.8\times10^{7}$ | $-5.14\times10^{-2}$ | $3.4\times10^{0}$ | $8.8\times10^{-8}$ | $1.2\times10^{9}$ |
| 2 | $1.6\times10^{-4}$ | $5.6\times10^{6}$ | $2.13\times10^{-2}$ | $2.2\times10^{-1}$ | $3.9\times10^{-8}$ | $5.4\times10^{8}$ |
| 3 | $7.8\times10^{-5}$ | $3.0\times10^{6}$ | $1.27\times10^{-2}$ | $1.2\times10^{-1}$ | $4.2\times10^{-8}$ | $5.7\times10^{8}$ |
| 4 | $3.9\times10^{-5}$ | $1.6\times10^{6}$ | $7.11\times10^{-3}$ | $6.8\times10^{-2}$ | $4.3\times10^{-8}$ | $6.0\times10^{8}$ |
| 5 | $2.0\times10^{-5}$ | $7.9\times10^{5}$ | $3.58\times10^{-3}$ | $3.5\times10^{-2}$ | $4.4\times10^{-8}$ | $6.1\times10^{8}$ |
| 6 | $9.8\times10^{-6}$ | $4.0\times10^{5}$ | $1.69\times10^{-3}$ | $1.8\times10^{-2}$ | $4.5\times10^{-8}$ | $6.1\times10^{8}$ |
| 7 | $4.9\times10^{-6}$ | $2.0\times10^{5}$ | $1.18\times10^{-3}$ | $9.2\times10^{-3}$ | $4.5\times10^{-8}$ | $6.2\times10^{8}$ |
| 8 | $2.4\times10^{-6}$ | $1.0\times10^{5}$ | $3.94\times10^{-4}$ | $4.8\times10^{-3}$ | $4.5\times10^{-8}$ | $6.4\times10^{8}$ |
| 9 | $1.2\times10^{-6}$ | $5.5\times10^{4}$ | $1.44\times10^{-4}$ | $2.7\times10^{-3}$ | $4.9\times10^{-8}$ | $6.7\times10^{8}$ |
| 10 | $6.1\times10^{-7}$ | $3.2\times10^{4}$ | $2.29\times10^{-4}$ | $8.1\times10^{-4}$ | $2.5\times10^{-8}$ | $7.8\times10^{8}$ |
| 11 | $3.1\times10^{-7}$ | $1.0\times10^{3}$ | $5.93\times10^{-4}$ | $1.3\times10^{-4}$ | $1.3\times10^{-7}$ | $4.9\times10^{7}$ |
| $\sum$ | | | $9.95\times10^{-1}$ | | $6.0\times10^{-7}$ | $6.9\times10^{9}$ |

Table 89: $\varepsilon = 0.05$, $\Delta t_1 = 1.56 \times 10^{-4}$

| $\ell$ | $\Delta t_\ell$ | $P_\ell$ | $\mathbb{E}[\hat{F}_\ell - \hat{F}_{\ell-1}]$ | $\mathbb{V}[\hat{F}_\ell - \hat{F}_{\ell-1}]$ | $\mathbb{V}[\hat{Y}_\ell]$ | $P_\ell C_\ell$ |
|---|---|---|---|---|---|---|
| 0 | $5.0\times10^{-1}$ | $1.3\times10^{9}$ | $9.97\times10^{-1}$ | $2.0\times10^{0}$ | $1.5\times10^{-9}$ | $2.7\times10^{7}$ |
| 1 | $1.6\times10^{-4}$ | $3.2\times10^{7}$ | $-3.01\times10^{-2}$ | $3.6\times10^{0}$ | $1.1\times10^{-7}$ | $2.1\times10^{9}$ |
| 2 | $7.8\times10^{-5}$ | $3.4\times10^{6}$ | $1.29\times10^{-2}$ | $1.2\times10^{-1}$ | $3.6\times10^{-8}$ | $6.6\times10^{8}$ |
| 3 | $3.9\times10^{-5}$ | $1.8\times10^{6}$ | $7.04\times10^{-3}$ | $6.7\times10^{-2}$ | $3.8\times10^{-8}$ | $6.8\times10^{8}$ |
| 4 | $2.0\times10^{-5}$ | $9.0\times10^{5}$ | $3.75\times10^{-3}$ | $3.5\times10^{-2}$ | $3.8\times10^{-8}$ | $6.9\times10^{8}$ |
| 5 | $9.8\times10^{-6}$ | $4.6\times10^{5}$ | $1.95\times10^{-3}$ | $1.8\times10^{-2}$ | $3.9\times10^{-8}$ | $7.0\times10^{8}$ |
| 6 | $4.9\times10^{-6}$ | $2.3\times10^{5}$ | $8.14\times10^{-4}$ | $8.8\times10^{-3}$ | $3.8\times10^{-8}$ | $7.0\times10^{8}$ |
| 7 | $2.4\times10^{-6}$ | $1.2\times10^{5}$ | $3.52\times10^{-4}$ | $4.6\times10^{-3}$ | $4.0\times10^{-8}$ | $7.1\times10^{8}$ |
| 8 | $1.2\times10^{-6}$ | $6.1\times10^{4}$ | $1.04\times10^{-4}$ | $2.5\times10^{-3}$ | $4.0\times10^{-8}$ | $7.5\times10^{8}$ |
| 9 | $6.1\times10^{-7}$ | $2.7\times10^{4}$ | $5.43\times10^{-5}$ | $9.8\times10^{-4}$ | $3.6\times10^{-8}$ | $6.7\times10^{8}$ |
| 10 | $3.1\times10^{-7}$ | $2.8\times10^{4}$ | $1.08\times10^{-4}$ | $4.9\times10^{-4}$ | $1.7\times10^{-8}$ | $1.4\times10^{9}$ |
| 11 | $1.5\times10^{-7}$ | $1.0\times10^{3}$ | $1.97\times10^{-4}$ | $5.5\times10^{-5}$ | $5.5\times10^{-8}$ | $9.8\times10^{7}$ |
| $\sum$ | | | $9.95\times10^{-1}$ | | $4.9\times10^{-7}$ | $9.1\times10^{9}$ |

Table 90: $\varepsilon = 0.05$, $\Delta t_1 = 7.81 \times 10^{-5}$

| $\ell$ | $\Delta t_\ell$ | $P_\ell$ | $\mathbb{E}[\hat{F}_\ell - \hat{F}_{\ell-1}]$ | $\mathbb{V}[\hat{F}_\ell - \hat{F}_{\ell-1}]$ | $\mathbb{V}[\hat{Y}_\ell]$ | $P_\ell C_\ell$ |
|---|---|---|---|---|---|---|
| 0 | $5.0\times10^{-1}$ | $1.2\times10^{9}$ | $9.98\times10^{-1}$ | $2.0\times10^{0}$ | $1.7\times10^{-9}$ | $2.3\times10^{7}$ |
| 1 | $7.8\times10^{-5}$ | $2.0\times10^{7}$ | $-1.73\times10^{-2}$ | $3.8\times10^{0}$ | $1.9\times10^{-7}$ | $2.6\times10^{9}$ |
| 2 | $3.9\times10^{-5}$ | $1.5\times10^{6}$ | $7.15\times10^{-3}$ | $6.7\times10^{-2}$ | $4.4\times10^{-8}$ | $5.9\times10^{8}$ |
| 3 | $2.0\times10^{-5}$ | $7.8\times10^{5}$ | $4.07\times10^{-3}$ | $3.5\times10^{-2}$ | $4.5\times10^{-8}$ | $6.0\times10^{8}$ |
| 4 | $9.8\times10^{-6}$ | $4.0\times10^{5}$ | $1.92\times10^{-3}$ | $1.8\times10^{-2}$ | $4.6\times10^{-8}$ | $6.2\times10^{8}$ |
| 5 | $4.9\times10^{-6}$ | $2.0\times10^{5}$ | $8.87\times10^{-4}$ | $8.7\times10^{-3}$ | $4.4\times10^{-8}$ | $6.0\times10^{8}$ |
| 6 | $2.4\times10^{-6}$ | $1.0\times10^{5}$ | $3.99\times10^{-4}$ | $4.7\times10^{-3}$ | $4.6\times10^{-8}$ | $6.3\times10^{8}$ |
| 7 | $1.2\times10^{-6}$ | $5.2\times10^{4}$ | $-7.27\times10^{-5}$ | $2.9\times10^{-3}$ | $5.7\times10^{-8}$ | $6.4\times10^{8}$ |
| 8 | $6.1\times10^{-7}$ | $1.8\times10^{4}$ | $3.03\times10^{-4}$ | $8.9\times10^{-4}$ | $4.8\times10^{-8}$ | $4.5\times10^{8}$ |
| 9 | $3.1\times10^{-7}$ | $1.0\times10^{3}$ | $-1.78\times10^{-4}$ | $5.8\times10^{-4}$ | $5.8\times10^{-7}$ | $4.9\times10^{7}$ |
| $\sum$ | | | $9.95\times10^{-1}$ | | $1.1\times10^{-6}$ | $6.8\times10^{9}$ |

Table 91: $\varepsilon = 0.05$, $\Delta t_1 = 3.91 \times 10^{-5}$

| $\ell$ | $\Delta t_\ell$ | $P_\ell$ | $\mathbb{E}[\hat{F}_\ell - \hat{F}_{\ell-1}]$ | $\mathbb{V}[\hat{F}_\ell - \hat{F}_{\ell-1}]$ | $\mathbb{V}[\hat{Y}_\ell]$ | $P_\ell C_\ell$ |
|---|---|---|---|---|---|---|
| 0 | $5.0\times10^{-1}$ | $1.2\times10^{9}$ | $9.97\times10^{-1}$ | $2.0\times10^{0}$ | $1.7\times10^{-9}$ | $2.4\times10^{7}$ |
| 1 | $3.9\times10^{-5}$ | $1.5\times10^{7}$ | $-1.06\times10^{-2}$ | $3.9\times10^{0}$ | $2.6\times10^{-7}$ | $3.8\times10^{9}$ |
| 2 | $2.0\times10^{-5}$ | $8.1\times10^{5}$ | $3.55\times10^{-3}$ | $3.5\times10^{-2}$ | $4.3\times10^{-8}$ | $6.2\times10^{8}$ |
| 3 | $9.8\times10^{-6}$ | $4.1\times10^{5}$ | $1.89\times10^{-3}$ | $1.8\times10^{-2}$ | $4.3\times10^{-8}$ | $6.3\times10^{8}$ |
| 4 | $4.9\times10^{-6}$ | $2.1\times10^{5}$ | $9.57\times10^{-4}$ | $9.3\times10^{-3}$ | $4.5\times10^{-8}$ | $6.3\times10^{8}$ |
| 5 | $2.4\times10^{-6}$ | $1.0\times10^{5}$ | $2.47\times10^{-4}$ | $4.6\times10^{-3}$ | $4.4\times10^{-8}$ | $6.4\times10^{8}$ |
| 6 | $1.2\times10^{-6}$ | $7.4\times10^{4}$ | $3.67\times10^{-4}$ | $2.5\times10^{-3}$ | $3.3\times10^{-8}$ | $9.1\times10^{8}$ |
| 7 | $6.1\times10^{-7}$ | $1.0\times10^{3}$ | $2.07\times10^{-4}$ | $2.5\times10^{-4}$ | $2.5\times10^{-7}$ | $2.5\times10^{7}$ |
| $\sum$ | | | $9.94\times10^{-1}$ | | $7.3\times10^{-7}$ | $7.3\times10^{9}$ |

Table 92: $\varepsilon = 0.05$, $\Delta t_1 = 1.95 \times 10^{-5}$

| $\ell$ | $\Delta t_\ell$ | $P_\ell$ | $\mathbb{E}[\hat{F}_\ell - \hat{F}_{\ell-1}]$ | $\mathbb{V}[\hat{F}_\ell - \hat{F}_{\ell-1}]$ | $\mathbb{V}[\hat{Y}_\ell]$ | $P_\ell C_\ell$ |
|---|---|---|---|---|---|---|
| 0 | $5.0\times10^{-1}$ | $1.3\times10^{9}$ | $9.98\times10^{-1}$ | $2.0\times10^{0}$ | $1.6\times10^{-9}$ | $2.6\times10^{7}$ |
| 1 | $2.0\times10^{-5}$ | $1.1\times10^{7}$ | $-6.57\times10^{-3}$ | $4.0\times10^{0}$ | $3.5\times10^{-7}$ | $5.8\times10^{9}$ |
| 2 | $9.8\times10^{-6}$ | $4.3\times10^{5}$ | $2.32\times10^{-3}$ | $1.7\times10^{-2}$ | $4.0\times10^{-8}$ | $6.6\times10^{8}$ |
| 3 | $4.9\times10^{-6}$ | $2.2\times10^{5}$ | $9.38\times10^{-4}$ | $9.3\times10^{-3}$ | $4.2\times10^{-8}$ | $6.9\times10^{8}$ |
| 4 | $2.4\times10^{-6}$ | $1.3\times10^{5}$ | $4.77\times10^{-4}$ | $5.8\times10^{-3}$ | $4.5\times10^{-8}$ | $7.9\times10^{8}$ |
| 5 | $1.2\times10^{-6}$ | $2.6\times10^{4}$ | $6.47\times10^{-4}$ | $2.4\times10^{-3}$ | $9.0\times10^{-8}$ | $3.2\times10^{8}$ |
| 6 | $6.1\times10^{-7}$ | $1.0\times10^{3}$ | $-2.15\times10^{-5}$ | $2.2\times10^{-4}$ | $2.2\times10^{-7}$ | $2.5\times10^{7}$ |
| $\sum$ | | | $9.95\times10^{-1}$ | | $7.9\times10^{-7}$ | $8.3\times10^{9}$ |

Table 93: $\varepsilon = 0.05$, $\Delta t_1 = 9.77 \times 10^{-6}$

| $\ell$ | $\Delta t_\ell$ | $P_\ell$ | $\mathbb{E}[\hat{F}_\ell - \hat{F}_{\ell-1}]$ | $\mathbb{V}[\hat{F}_\ell - \hat{F}_{\ell-1}]$ | $\mathbb{V}[\hat{Y}_\ell]$ | $P_\ell C_\ell$ |
|---|---|---|---|---|---|---|
| 0 | $5.0\times10^{-1}$ | $1.6\times10^{9}$ | $9.97\times10^{-1}$ | $2.0\times10^{0}$ | $1.2\times10^{-9}$ | $3.2\times10^{7}$ |
| 1 | $9.8\times10^{-6}$ | $1.0\times10^{7}$ | $-4.54\times10^{-3}$ | $4.0\times10^{0}$ | $3.9\times10^{-7}$ | $1.0\times10^{10}$ |
| 2 | $4.9\times10^{-6}$ | $2.8\times10^{5}$ | $7.79\times10^{-4}$ | $9.0\times10^{-3}$ | $3.2\times10^{-8}$ | $8.5\times10^{8}$ |
| 3 | $2.4\times10^{-6}$ | $1.4\times10^{5}$ | $5.12\times10^{-4}$ | $4.4\times10^{-3}$ | $3.0\times10^{-8}$ | $8.9\times10^{8}$ |
| 4 | $1.2\times10^{-6}$ | $8.2\times10^{4}$ | $5.12\times10^{-4}$ | $2.3\times10^{-3}$ | $2.8\times10^{-8}$ | $1.0\times10^{9}$ |
| 5 | $6.1\times10^{-7}$ | $1.0\times10^{3}$ | $-2.80\times10^{-5}$ | $3.5\times10^{-4}$ | $3.5\times10^{-7}$ | $2.5\times10^{7}$ |
| $\sum$ | | | $9.95\times10^{-1}$ | | $8.4\times10^{-7}$ | $1.3\times10^{10}$ |

Table 94: $\varepsilon = 0.05$, $\Delta t_1 = 4.88 \times 10^{-6}$

| $\ell$ | $\Delta t_\ell$ | $P_\ell$ | $\mathbb{E}[\hat{F}_\ell - \hat{F}_{\ell-1}]$ | $\mathbb{V}[\hat{F}_\ell - \hat{F}_{\ell-1}]$ | $\mathbb{V}[\hat{Y}_\ell]$ | $P_\ell C_\ell$ |
|---|---|---|---|---|---|---|
| 0 | $5.0\times10^{-1}$ | $2.1\times10^{9}$ | $9.98\times10^{-1}$ | $2.0\times10^{0}$ | $9.6\times10^{-10}$ | $4.2\times10^{7}$ |
| 1 | $4.9\times10^{-6}$ | $9.2\times10^{6}$ | $-3.06\times10^{-3}$ | $4.0\times10^{0}$ | $4.3\times10^{-7}$ | $1.9\times10^{10}$ |
| 2 | $2.4\times10^{-6}$ | $1.9\times10^{5}$ | $7.18\times10^{-4}$ | $4.9\times10^{-3}$ | $2.6\times10^{-8}$ | $1.1\times10^{9}$ |
| 3 | $1.2\times10^{-6}$ | $1.2\times10^{5}$ | $-2.78\times10^{-5}$ | $2.0\times10^{-3}$ | $1.6\times10^{-8}$ | $1.5\times10^{9}$ |
| 4 | $6.1\times10^{-7}$ | $2.8\times10^{4}$ | $-2.61\times10^{-4}$ | $1.5\times10^{-3}$ | $5.4\times10^{-8}$ | $7.0\times10^{8}$ |
| 5 | $3.1\times10^{-7}$ | $1.0\times10^{3}$ | $-1.91\times10^{-4}$ | $4.6\times10^{-4}$ | $4.6\times10^{-7}$ | $4.9\times10^{7}$ |
| $\sum$ | | | $9.95\times10^{-1}$ | | $9.9\times10^{-7}$ | $2.2\times10^{10}$ |

Table 95: $\varepsilon = 0.05$, $\Delta t_1 = 2.44 \times 10^{-6}$

| $\ell$ | $\Delta t_\ell$ | $P_\ell$ | $\mathbb{E}[\hat{F}_\ell - \hat{F}_{\ell-1}]$ | $\mathbb{V}[\hat{F}_\ell - \hat{F}_{\ell-1}]$ | $\mathbb{V}[\hat{Y}_\ell]$ | $P_\ell C_\ell$ |
|---|---|---|---|---|---|---|
| 0 | $5.0\times10^{-1}$ | $2.8\times10^{9}$ | $9.97\times10^{-1}$ | $2.0\times10^{0}$ | $7.2\times10^{-10}$ | $5.5\times10^{7}$ |
| 1 | $2.4\times10^{-6}$ | $8.6\times10^{6}$ | $-2.17\times10^{-3}$ | $4.0\times10^{0}$ | $4.6\times10^{-7}$ | $3.5\times10^{10}$ |
| 2 | $1.2\times10^{-6}$ | $1.3\times10^{5}$ | $1.32\times10^{-4}$ | $2.3\times10^{-3}$ | $1.7\times10^{-8}$ | $1.6\times10^{9}$ |
| 3 | $6.1\times10^{-7}$ | $5.3\times10^{4}$ | $8.69\times10^{-5}$ | $9.8\times10^{-4}$ | $1.9\times10^{-8}$ | $1.3\times10^{9}$ |
| 4 | $3.1\times10^{-7}$ | $1.0\times10^{3}$ | $3.91\times10^{-4}$ | $4.1\times10^{-4}$ | $4.1\times10^{-7}$ | $4.9\times10^{7}$ |
| $\sum$ | | | $9.96\times10^{-1}$ | | $9.1\times10^{-7}$ | $3.8\times10^{10}$ |

Table 96: $\varepsilon = 0.05$, $\Delta t_1 = 1.22 \times 10^{-6}$

| $\ell$ | $\Delta t_\ell$ | $P_\ell$ | $\mathbb{E}[\hat{F}_\ell - \hat{F}_{\ell-1}]$ | $\mathbb{V}[\hat{F}_\ell - \hat{F}_{\ell-1}]$ | $\mathbb{V}[\hat{Y}_\ell]$ | $P_\ell C_\ell$ |
|---|---|---|---|---|---|---|
| 0 | $5.0\times10^{-1}$ | $3.8\times10^{9}$ | $9.97\times10^{-1}$ | $2.0\times10^{0}$ | $5.2\times10^{-10}$ | $7.6\times10^{7}$ |
| 1 | $1.2\times10^{-6}$ | $8.7\times10^{6}$ | $-2.88\times10^{-3}$ | $4.0\times10^{0}$ | $4.6\times10^{-7}$ | $7.1\times10^{10}$ |
| 2 | $6.1\times10^{-7}$ | $8.1\times10^{4}$ | $2.47\times10^{-4}$ | $1.2\times10^{-3}$ | $1.5\times10^{-8}$ | $2.0\times10^{9}$ |
| 3 | $3.1\times10^{-7}$ | $3.0\times10^{4}$ | $-9.63\times10^{-5}$ | $6.4\times10^{-4}$ | $2.1\times10^{-8}$ | $1.5\times10^{9}$ |
| 4 | $1.5\times10^{-7}$ | $1.0\times10^{3}$ | $-2.21\times10^{-4}$ | $1.4\times10^{-4}$ | $1.4\times10^{-7}$ | $9.8\times10^{7}$ |
| $\sum$ | | | $9.95\times10^{-1}$ | | $6.3\times10^{-7}$ | $7.5\times10^{10}$ |

## 2.4 Combined correlation, $\varepsilon = 0.5$

Table 97: $\varepsilon = 0.5$, $\Delta t_1 = 2.50 \times 10^{-1}$

| $\ell$ | $\Delta t_\ell$ | $P_\ell$ | $\mathbb{E}[\hat{F}_\ell - \hat{F}_{\ell-1}]$ | $\mathbb{V}[\hat{F}_\ell - \hat{F}_{\ell-1}]$ | $\mathbb{V}[\hat{Y}_\ell]$ | $P_\ell C_\ell$ |
|---|---|---|---|---|---|---|
| 0 | $5.0\times10^{-1}$ | $5.7\times10^{7}$ | $7.78\times10^{-1}$ | $1.2\times10^{0}$ | $2.1\times10^{-8}$ | $1.1\times10^{6}$ |
| 1 | $2.5\times10^{-1}$ | $1.3\times10^{7}$ | $-9.03\times10^{-2}$ | $1.8\times10^{-1}$ | $1.4\times10^{-8}$ | $7.6\times10^{5}$ |
| 2 | $1.2\times10^{-1}$ | $8.7\times10^{6}$ | $-6.59\times10^{-2}$ | $1.7\times10^{-1}$ | $2.0\times10^{-8}$ | $1.0\times10^{6}$ |
| 3 | $6.2\times10^{-2}$ | $5.4\times10^{6}$ | $-3.42\times10^{-2}$ | $1.3\times10^{-1}$ | $2.5\times10^{-8}$ | $1.3\times10^{6}$ |
| 4 | $3.1\times10^{-2}$ | $3.1\times10^{6}$ | $-1.33\times10^{-2}$ | $8.6\times10^{-2}$ | $2.8\times10^{-8}$ | $1.5\times10^{6}$ |
| 5 | $1.6\times10^{-2}$ | $1.7\times10^{6}$ | $-4.30\times10^{-3}$ | $5.0\times10^{-2}$ | $3.0\times10^{-8}$ | $1.6\times10^{6}$ |
| 6 | $7.8\times10^{-3}$ | $8.7\times10^{5}$ | $-1.30\times10^{-3}$ | $2.8\times10^{-2}$ | $3.2\times10^{-8}$ | $1.7\times10^{6}$ |
| 7 | $3.9\times10^{-3}$ | $4.4\times10^{5}$ | $-4.46\times10^{-4}$ | $1.4\times10^{-2}$ | $3.1\times10^{-8}$ | $1.7\times10^{6}$ |
| 8 | $2.0\times10^{-3}$ | $2.1\times10^{5}$ | $3.22\times10^{-4}$ | $6.5\times10^{-3}$ | $3.1\times10^{-8}$ | $1.6\times10^{6}$ |
| 9 | $9.8\times10^{-4}$ | $1.1\times10^{5}$ | $-1.25\times10^{-4}$ | $4.4\times10^{-3}$ | $3.9\times10^{-8}$ | $1.7\times10^{6}$ |
| 10 | $4.9\times10^{-4}$ | $4.0\times10^{5}$ | $-1.21\times10^{-4}$ | $2.0\times10^{-3}$ | $4.8\times10^{-9}$ | $1.2\times10^{7}$ |
| 11 | $2.4\times10^{-4}$ | $1.3\times10^{4}$ | $1.25\times10^{-4}$ | $4.0\times10^{-4}$ | $3.2\times10^{-8}$ | $7.8\times10^{5}$ |
| 12 | $1.2\times10^{-4}$ | $1.0\times10^{3}$ | $-3.40\times10^{-4}$ | $1.9\times10^{-4}$ | $1.9\times10^{-7}$ | $1.2\times10^{5}$ |
| $\sum$ | | | $5.68\times10^{-1}$ | | $4.9\times10^{-7}$ | $2.7\times10^{7}$ |

Table 98: $\varepsilon = 0.5$, $\Delta t_1 = 1.25 \times 10^{-1}$

| $\ell$ | $\Delta t_\ell$ | $P_\ell$ | $\mathbb{E}[\hat{F}_\ell - \hat{F}_{\ell-1}]$ | $\mathbb{V}[\hat{F}_\ell - \hat{F}_{\ell-1}]$ | $\mathbb{V}[\hat{Y}_\ell]$ | $P_\ell C_\ell$ |
|---|---|---|---|---|---|---|
| 0 | $5.0\times10^{-1}$ | $3.3\times10^{7}$ | $7.77\times10^{-1}$ | $1.2\times10^{0}$ | $3.7\times10^{-8}$ | $6.5\times10^{5}$ |
| 1 | $1.2\times10^{-1}$ | $9.6\times10^{6}$ | $-1.57\times10^{-1}$ | $5.2\times10^{-1}$ | $5.5\times10^{-8}$ | $9.6\times10^{5}$ |
| 2 | $6.2\times10^{-2}$ | $3.1\times10^{6}$ | $-3.45\times10^{-2}$ | $1.3\times10^{-1}$ | $4.2\times10^{-8}$ | $7.4\times10^{5}$ |
| 3 | $3.1\times10^{-2}$ | $1.8\times10^{6}$ | $-1.33\times10^{-2}$ | $8.6\times10^{-2}$ | $4.9\times10^{-8}$ | $8.5\times10^{5}$ |
| 4 | $1.6\times10^{-2}$ | $9.6\times10^{5}$ | $-4.66\times10^{-3}$ | $5.0\times10^{-2}$ | $5.2\times10^{-8}$ | $9.2\times10^{5}$ |
| 5 | $7.8\times10^{-3}$ | $5.0\times10^{5}$ | $-1.07\times10^{-3}$ | $2.8\times10^{-2}$ | $5.5\times10^{-8}$ | $9.7\times10^{5}$ |
| 6 | $3.9\times10^{-3}$ | $2.7\times10^{5}$ | $-7.81\times10^{-4}$ | $1.6\times10^{-2}$ | $5.9\times10^{-8}$ | $1.1\times10^{6}$ |
| 7 | $2.0\times10^{-3}$ | $1.3\times10^{5}$ | $3.56\times10^{-5}$ | $6.3\times10^{-3}$ | $4.8\times10^{-8}$ | $1.0\times10^{6}$ |
| 8 | $9.8\times10^{-4}$ | $6.8\times10^{4}$ | $2.42\times10^{-4}$ | $4.1\times10^{-3}$ | $6.1\times10^{-8}$ | $1.0\times10^{6}$ |
| 9 | $4.9\times10^{-4}$ | $2.2\times10^{4}$ | $5.17\times10^{-4}$ | $1.4\times10^{-3}$ | $6.7\times10^{-8}$ | $6.6\times10^{5}$ |
| 10 | $2.4\times10^{-4}$ | $1.0\times10^{3}$ | $-2.18\times10^{-4}$ | $3.9\times10^{-4}$ | $3.9\times10^{-7}$ | $6.1\times10^{4}$ |
| $\sum$ | | | $5.67\times10^{-1}$ | | $9.2\times10^{-7}$ | $8.9\times10^{6}$ |

Table 99: $\varepsilon = 0.5$, $\Delta t_1 = 6.25 \times 10^{-2}$

| $\ell$ | $\Delta t_\ell$ | $P_\ell$ | $\mathbb{E}[\hat{F}_\ell - \hat{F}_{\ell-1}]$ | $\mathbb{V}[\hat{F}_\ell - \hat{F}_{\ell-1}]$ | $\mathbb{V}[\hat{Y}_\ell]$ | $P_\ell C_\ell$ |
|---|---|---|---|---|---|---|
| 0 | $5.0\times10^{-1}$ | $3.0\times10^{7}$ | $7.78\times10^{-1}$ | $1.2\times10^{0}$ | $4.0\times10^{-8}$ | $6.0\times10^{5}$ |
| 1 | $6.2\times10^{-2}$ | $8.6\times10^{6}$ | $-1.91\times10^{-1}$ | $9.0\times10^{-1}$ | $1.0\times10^{-7}$ | $1.5\times10^{6}$ |
| 2 | $3.1\times10^{-2}$ | $1.6\times10^{6}$ | $-1.38\times10^{-2}$ | $8.7\times10^{-2}$ | $5.3\times10^{-8}$ | $7.8\times10^{5}$ |
| 3 | $1.6\times10^{-2}$ | $8.8\times10^{5}$ | $-3.93\times10^{-3}$ | $5.0\times10^{-2}$ | $5.7\times10^{-8}$ | $8.4\times10^{5}$ |
| 4 | $7.8\times10^{-3}$ | $4.6\times10^{5}$ | $-9.97\times10^{-4}$ | $2.8\times10^{-2}$ | $6.0\times10^{-8}$ | $8.8\times10^{5}$ |
| 5 | $3.9\times10^{-3}$ | $2.3\times10^{5}$ | $-4.43\times10^{-4}$ | $1.5\times10^{-2}$ | $6.3\times10^{-8}$ | $8.9\times10^{5}$ |
| 6 | $2.0\times10^{-3}$ | $1.1\times10^{5}$ | $2.08\times10^{-4}$ | $6.2\times10^{-3}$ | $5.7\times10^{-8}$ | $8.4\times10^{5}$ |
| 7 | $9.8\times10^{-4}$ | $6.5\times10^{4}$ | $-1.90\times10^{-4}$ | $4.6\times10^{-3}$ | $7.1\times10^{-8}$ | $1.0\times10^{6}$ |
| 8 | $4.9\times10^{-4}$ | $1.0\times10^{3}$ | $8.61\times10^{-5}$ | $1.2\times10^{-3}$ | $1.2\times10^{-6}$ | $3.1\times10^{4}$ |
| $\sum$ | | | $5.68\times10^{-1}$ | | $1.7\times10^{-6}$ | $7.4\times10^{6}$ |

Table 100: $\varepsilon = 0.5$, $\Delta t_1 = 3.12 \times 10^{-2}$

| $\ell$ | $\Delta t_\ell$ | $P_\ell$ | $\mathbb{E}[\hat{F}_\ell - \hat{F}_{\ell-1}]$ | $\mathbb{V}[\hat{F}_\ell - \hat{F}_{\ell-1}]$ | $\mathbb{V}[\hat{Y}_\ell]$ | $P_\ell C_\ell$ |
|---|---|---|---|---|---|---|
| 0 | $5.0\times10^{-1}$ | $3.3\times10^{7}$ | $7.78\times10^{-1}$ | $1.2\times10^{0}$ | $3.7\times10^{-8}$ | $6.6\times10^{5}$ |
| 1 | $3.1\times10^{-2}$ | $8.0\times10^{6}$ | $-2.04\times10^{-1}$ | $1.2\times10^{0}$ | $1.5\times10^{-7}$ | $2.7\times10^{6}$ |
| 2 | $1.6\times10^{-2}$ | $9.8\times10^{5}$ | $-4.23\times10^{-3}$ | $5.1\times10^{-2}$ | $5.2\times10^{-8}$ | $9.4\times10^{5}$ |
| 3 | $7.8\times10^{-3}$ | $5.0\times10^{5}$ | $-1.34\times10^{-3}$ | $2.6\times10^{-2}$ | $5.3\times10^{-8}$ | $9.5\times10^{5}$ |
| 4 | $3.9\times10^{-3}$ | $2.6\times10^{5}$ | $-3.41\times10^{-4}$ | $1.5\times10^{-2}$ | $5.5\times10^{-8}$ | $1.0\times10^{6}$ |
| 5 | $2.0\times10^{-3}$ | $1.3\times10^{5}$ | $-2.41\times10^{-4}$ | $6.9\times10^{-3}$ | $5.3\times10^{-8}$ | $1.0\times10^{6}$ |
| 6 | $9.8\times10^{-4}$ | $7.0\times10^{4}$ | $7.43\times10^{-5}$ | $3.7\times10^{-3}$ | $5.3\times10^{-8}$ | $1.1\times10^{6}$ |
| 7 | $4.9\times10^{-4}$ | $2.1\times10^{4}$ | $1.33\times10^{-4}$ | $1.5\times10^{-3}$ | $7.4\times10^{-8}$ | $6.5\times10^{5}$ |
| 8 | $2.4\times10^{-4}$ | $1.0\times10^{3}$ | $5.91\times10^{-4}$ | $3.8\times10^{-4}$ | $3.8\times10^{-7}$ | $6.1\times10^{4}$ |
| $\sum$ | | | $5.68\times10^{-1}$ | | $9.1\times10^{-7}$ | $9.1\times10^{6}$ |

Table 101: $\varepsilon = 0.5$, $\Delta t_1 = 1.56 \times 10^{-2}$

| $\ell$ | $\Delta t_\ell$ | $P_\ell$ | $\mathbb{E}[\hat{F}_\ell - \hat{F}_{\ell-1}]$ | $\mathbb{V}[\hat{F}_\ell - \hat{F}_{\ell-1}]$ | $\mathbb{V}[\hat{Y}_\ell]$ | $P_\ell C_\ell$ |
|---|---|---|---|---|---|---|
| 0 | $5.0\times10^{-1}$ | $3.3\times10^{7}$ | $7.78\times10^{-1}$ | $1.2\times10^{0}$ | $3.7\times10^{-8}$ | $6.6\times10^{5}$ |
| 1 | $1.6\times10^{-2}$ | $6.2\times10^{6}$ | $-2.09\times10^{-1}$ | $1.4\times10^{0}$ | $2.3\times10^{-7}$ | $4.1\times10^{6}$ |
| 2 | $7.8\times10^{-3}$ | $5.0\times10^{5}$ | $-9.34\times10^{-4}$ | $2.7\times10^{-2}$ | $5.3\times10^{-8}$ | $9.6\times10^{5}$ |
| 3 | $3.9\times10^{-3}$ | $2.6\times10^{5}$ | $-2.37\times10^{-4}$ | $1.4\times10^{-2}$ | $5.5\times10^{-8}$ | $9.8\times10^{5}$ |
| 4 | $2.0\times10^{-3}$ | $1.5\times10^{5}$ | $-2.63\times10^{-4}$ | $8.0\times10^{-3}$ | $5.3\times10^{-8}$ | $1.1\times10^{6}$ |
| 5 | $9.8\times10^{-4}$ | $7.1\times10^{4}$ | $6.24\times10^{-5}$ | $3.1\times10^{-3}$ | $4.4\times10^{-8}$ | $1.1\times10^{6}$ |
| 6 | $4.9\times10^{-4}$ | $1.0\times10^{3}$ | $-5.67\times10^{-4}$ | $6.9\times10^{-4}$ | $6.9\times10^{-7}$ | $3.1\times10^{4}$ |
| $\sum$ | | | $5.68\times10^{-1}$ | | $1.2\times10^{-6}$ | $8.9\times10^{6}$ |

Table 102: $\varepsilon = 0.5$, $\Delta t_1 = 7.81 \times 10^{-3}$

| $\ell$ | $\Delta t_\ell$ | $P_\ell$ | $\mathbb{E}[\hat{F}_\ell - \hat{F}_{\ell-1}]$ | $\mathbb{V}[\hat{F}_\ell - \hat{F}_{\ell-1}]$ | $\mathbb{V}[\hat{Y}_\ell]$ | $P_\ell C_\ell$ |
|---|---|---|---|---|---|---|
| 0 | $5.0\times10^{-1}$ | $4.5\times10^{7}$ | $7.78\times10^{-1}$ | $1.2\times10^{0}$ | $2.7\times10^{-8}$ | $9.0\times10^{5}$ |
| 1 | $7.8\times10^{-3}$ | $6.2\times10^{6}$ | $-2.09\times10^{-1}$ | $1.5\times10^{0}$ | $2.5\times10^{-7}$ | $8.1\times10^{6}$ |
| 2 | $3.9\times10^{-3}$ | $3.5\times10^{5}$ | $-5.91\times10^{-4}$ | $1.4\times10^{-2}$ | $4.0\times10^{-8}$ | $1.3\times10^{6}$ |
| 3 | $2.0\times10^{-3}$ | $1.9\times10^{5}$ | $-1.64\times10^{-5}$ | $7.7\times10^{-3}$ | $4.1\times10^{-8}$ | $1.4\times10^{6}$ |
| 4 | $9.8\times10^{-4}$ | $3.1\times10^{5}$ | $-1.22\times10^{-4}$ | $3.9\times10^{-3}$ | $1.3\times10^{-8}$ | $4.8\times10^{6}$ |
| 5 | $4.9\times10^{-4}$ | $4.6\times10^{4}$ | $1.97\times10^{-4}$ | $1.7\times10^{-3}$ | $3.8\times10^{-8}$ | $1.4\times10^{6}$ |
| 6 | $2.4\times10^{-4}$ | $2.3\times10^{4}$ | $3.76\times10^{-4}$ | $1.1\times10^{-3}$ | $4.7\times10^{-8}$ | $1.4\times10^{6}$ |
| 7 | $1.2\times10^{-4}$ | $1.0\times10^{3}$ | $5.95\times10^{-5}$ | $3.9\times10^{-4}$ | $3.9\times10^{-7}$ | $1.2\times10^{5}$ |
| $\sum$ | | | $5.69\times10^{-1}$ | | $8.4\times10^{-7}$ | $2.0\times10^{7}$ |

Table 103: $\varepsilon = 0.5$, $\Delta t_1 = 3.91 \times 10^{-3}$

| $\ell$ | $\Delta t_\ell$ | $P_\ell$ | $\mathbb{E}[\hat{F}_\ell - \hat{F}_{\ell-1}]$ | $\mathbb{V}[\hat{F}_\ell - \hat{F}_{\ell-1}]$ | $\mathbb{V}[\hat{Y}_\ell]$ | $P_\ell C_\ell$ |
|---|---|---|---|---|---|---|
| 0 | $5.0\times10^{-1}$ | $4.0\times10^{7}$ | $7.78\times10^{-1}$ | $1.2\times10^{0}$ | $3.0\times10^{-8}$ | $8.1\times10^{5}$ |
| 1 | $3.9\times10^{-3}$ | $4.1\times10^{6}$ | $-2.10\times10^{-1}$ | $1.6\times10^{0}$ | $3.9\times10^{-7}$ | $1.1\times10^{7}$ |
| 2 | $2.0\times10^{-3}$ | $1.6\times10^{5}$ | $-1.05\times10^{-4}$ | $8.4\times10^{-3}$ | $5.2\times10^{-8}$ | $1.2\times10^{6}$ |
| 3 | $9.8\times10^{-4}$ | $5.4\times10^{4}$ | $-1.26\times10^{-4}$ | $4.0\times10^{-3}$ | $7.5\times10^{-8}$ | $8.2\times10^{5}$ |
| 4 | $4.9\times10^{-4}$ | $1.0\times10^{3}$ | $-1.44\times10^{-5}$ | $7.2\times10^{-4}$ | $7.2\times10^{-7}$ | $3.1\times10^{4}$ |
| $\sum$ | | | $5.67\times10^{-1}$ | | $1.3\times10^{-6}$ | $1.3\times10^{7}$ |

Table 104: $\varepsilon = 0.5$, $\Delta t_1 = 1.95 \times 10^{-3}$

| $\ell$ | $\Delta t_\ell$ | $P_\ell$ | $\mathbb{E}[\hat{F}_\ell - \hat{F}_{\ell-1}]$ | $\mathbb{V}[\hat{F}_\ell - \hat{F}_{\ell-1}]$ | $\mathbb{V}[\hat{Y}_\ell]$ | $P_\ell C_\ell$ |
|---|---|---|---|---|---|---|
| 0 | $5.0\times10^{-1}$ | $5.5\times10^{7}$ | $7.78\times10^{-1}$ | $1.2\times10^{0}$ | $2.2\times10^{-8}$ | $1.1\times10^{6}$ |
| 1 | $2.0\times10^{-3}$ | $4.0\times10^{6}$ | $-2.10\times10^{-1}$ | $1.7\times10^{0}$ | $4.1\times10^{-7}$ | $2.1\times10^{7}$ |
| 2 | $9.8\times10^{-4}$ | $1.1\times10^{5}$ | $1.65\times10^{-4}$ | $3.3\times10^{-3}$ | $3.1\times10^{-8}$ | $1.6\times10^{6}$ |
| 3 | $4.9\times10^{-4}$ | $4.8\times10^{4}$ | $1.90\times10^{-4}$ | $1.9\times10^{-3}$ | $4.0\times10^{-8}$ | $1.5\times10^{6}$ |
| 4 | $2.4\times10^{-4}$ | $1.0\times10^{3}$ | $-5.73\times10^{-4}$ | $4.1\times10^{-4}$ | $4.1\times10^{-7}$ | $6.1\times10^{4}$ |
| $\sum$ | | | $5.67\times10^{-1}$ | | $9.1\times10^{-7}$ | $2.5\times10^{7}$ |

Table 105: $\varepsilon = 0.5$, $\Delta t_1 = 9.77 \times 10^{-4}$

| $\ell$ | $\Delta t_\ell$ | $P_\ell$ | $\mathbb{E}[\hat{F}_\ell - \hat{F}_{\ell-1}]$ | $\mathbb{V}[\hat{F}_\ell - \hat{F}_{\ell-1}]$ | $\mathbb{V}[\hat{Y}_\ell]$ | $P_\ell C_\ell$ |
|---|---|---|---|---|---|---|
| 0 | $5.0\times10^{-1}$ | $7.3\times10^{7}$ | $7.78\times10^{-1}$ | $1.2\times10^{0}$ | $1.7\times10^{-8}$ | $1.5\times10^{6}$ |
| 1 | $9.8\times10^{-4}$ | $3.8\times10^{6}$ | $-2.09\times10^{-1}$ | $1.7\times10^{0}$ | $4.4\times10^{-7}$ | $3.9\times10^{7}$ |
| 2 | $4.9\times10^{-4}$ | $6.6\times10^{4}$ | $3.74\times10^{-4}$ | $2.0\times10^{-3}$ | $3.0\times10^{-8}$ | $2.0\times10^{6}$ |
| 3 | $2.4\times10^{-4}$ | $2.3\times10^{4}$ | $-2.72\times10^{-4}$ | $6.7\times10^{-4}$ | $2.9\times10^{-8}$ | $1.4\times10^{6}$ |
| 4 | $1.2\times10^{-4}$ | $1.0\times10^{3}$ | $-3.56\times10^{-4}$ | $1.8\times10^{-4}$ | $1.8\times10^{-7}$ | $1.2\times10^{5}$ |
| $\sum$ | | | $5.68\times10^{-1}$ | | $7.0\times10^{-7}$ | $4.4\times10^{7}$ |

Table 106: $\varepsilon = 0.5$, $\Delta t_1 = 4.88 \times 10^{-4}$

| $\ell$ | $\Delta t_\ell$ | $P_\ell$ | $\mathbb{E}[\hat{F}_\ell - \hat{F}_{\ell-1}]$ | $\mathbb{V}[\hat{F}_\ell - \hat{F}_{\ell-1}]$ | $\mathbb{V}[\hat{Y}_\ell]$ | $P_\ell C_\ell$ |
|---|---|---|---|---|---|---|
| 0 | $5.0\times10^{-1}$ | $1.0\times10^{8}$ | $7.78\times10^{-1}$ | $1.2\times10^{0}$ | $1.2\times10^{-8}$ | $2.0\times10^{6}$ |
| 1 | $4.9\times10^{-4}$ | $3.8\times10^{6}$ | $-2.10\times10^{-1}$ | $1.7\times10^{0}$ | $4.5\times10^{-7}$ | $7.8\times10^{7}$ |
| 2 | $2.4\times10^{-4}$ | $6.4\times10^{4}$ | $-2.57\times10^{-5}$ | $9.7\times10^{-4}$ | $1.5\times10^{-8}$ | $3.9\times10^{6}$ |
| 3 | $1.2\times10^{-4}$ | $1.6\times10^{4}$ | $-1.37\times10^{-5}$ | $1.9\times10^{-4}$ | $1.2\times10^{-8}$ | $2.0\times10^{6}$ |
| 4 | $6.1\times10^{-5}$ | $1.0\times10^{3}$ | $-5.42\times10^{-4}$ | $9.3\times10^{-5}$ | $9.3\times10^{-8}$ | $2.5\times10^{5}$ |
| $\sum$ | | | $5.67\times10^{-1}$ | | $5.9\times10^{-7}$ | $8.7\times10^{7}$ |

## 2.5 Combined correlation, $\varepsilon = 0.1$

Table 107: $\varepsilon = 0.1$, $\Delta t_1 = 1.00 \times 10^{-2}$

| $\ell$ | $\Delta t_\ell$ | $P_\ell$ | $\mathbb{E}[\hat{F}_\ell - \hat{F}_{\ell-1}]$ | $\mathbb{V}[\hat{F}_\ell - \hat{F}_{\ell-1}]$ | $\mathbb{V}[\hat{Y}_\ell]$ | $P_\ell C_\ell$ |
|---|---|---|---|---|---|---|
| 0 | $5.0\times10^{-1}$ | $5.1\times10^{8}$ | $9.90\times10^{-1}$ | $2.0\times10^{0}$ | $3.9\times10^{-9}$ | $1.0\times10^{7}$ |
| 1 | $1.0\times10^{-2}$ | $2.1\times10^{7}$ | $-1.25\times10^{-1}$ | $1.7\times10^{-1}$ | $8.0\times10^{-9}$ | $2.1\times10^{7}$ |
| 2 | $5.0\times10^{-3}$ | $2.0\times10^{7}$ | $1.04\times10^{-2}$ | $4.7\times10^{-1}$ | $2.3\times10^{-8}$ | $6.1\times10^{7}$ |
| 3 | $2.5\times10^{-3}$ | $1.4\times10^{7}$ | $2.84\times10^{-2}$ | $4.4\times10^{-1}$ | $3.2\times10^{-8}$ | $8.3\times10^{7}$ |
| 4 | $1.3\times10^{-3}$ | $8.5\times10^{6}$ | $2.88\times10^{-2}$ | $3.3\times10^{-1}$ | $3.9\times10^{-8}$ | $1.0\times10^{8}$ |
| 5 | $6.3\times10^{-4}$ | $4.9\times10^{6}$ | $2.08\times10^{-2}$ | $2.1\times10^{-1}$ | $4.4\times10^{-8}$ | $1.2\times10^{8}$ |
| 6 | $3.1\times10^{-4}$ | $2.6\times10^{6}$ | $1.22\times10^{-2}$ | $1.2\times10^{-1}$ | $4.7\times10^{-8}$ | $1.2\times10^{8}$ |
| 7 | $1.6\times10^{-4}$ | $1.3\times10^{6}$ | $6.87\times10^{-3}$ | $6.5\times10^{-2}$ | $4.9\times10^{-8}$ | $1.3\times10^{8}$ |
| 8 | $7.8\times10^{-5}$ | $6.8\times10^{5}$ | $3.65\times10^{-3}$ | $3.4\times10^{-2}$ | $5.0\times10^{-8}$ | $1.3\times10^{8}$ |
| 9 | $3.9\times10^{-5}$ | $3.5\times10^{5}$ | $2.22\times10^{-3}$ | $1.8\times10^{-2}$ | $5.2\times10^{-8}$ | $1.4\times10^{8}$ |
| 10 | $2.0\times10^{-5}$ | $3.8\times10^{5}$ | $1.03\times10^{-3}$ | $8.6\times10^{-3}$ | $2.3\times10^{-8}$ | $2.9\times10^{8}$ |
| 11 | $9.8\times10^{-6}$ | $8.2\times10^{4}$ | $4.10\times10^{-4}$ | $4.7\times10^{-3}$ | $5.8\times10^{-8}$ | $1.3\times10^{8}$ |
| 12 | $4.9\times10^{-6}$ | $4.8\times10^{4}$ | $3.27\times10^{-4}$ | $2.3\times10^{-3}$ | $4.8\times10^{-8}$ | $1.5\times10^{8}$ |
| 13 | $2.4\times10^{-6}$ | $1.0\times10^{3}$ | $3.91\times10^{-4}$ | $1.8\times10^{-4}$ | $1.8\times10^{-7}$ | $6.1\times10^{6}$ |
| $\sum$ | | | $9.81\times10^{-1}$ | | $6.6\times10^{-7}$ | $1.5\times10^{9}$ |

Table 108: $\varepsilon = 0.1$, $\Delta t_1 = 5.00 \times 10^{-3}$

| $\ell$ | $\Delta t_\ell$ | $P_\ell$ | $\mathbb{E}[\hat{F}_\ell - \hat{F}_{\ell-1}]$ | $\mathbb{V}[\hat{F}_\ell - \hat{F}_{\ell-1}]$ | $\mathbb{V}[\hat{Y}_\ell]$ | $P_\ell C_\ell$ |
|---|---|---|---|---|---|---|
| 0 | $5.0\times10^{-1}$ | $4.6\times10^{8}$ | $9.90\times10^{-1}$ | $2.0\times10^{0}$ | $4.3\times10^{-9}$ | $9.2\times10^{6}$ |
| 1 | $5.0\times10^{-3}$ | $1.5\times10^{7}$ | $-1.14\times10^{-1}$ | $2.0\times10^{-1}$ | $1.4\times10^{-8}$ | $2.9\times10^{7}$ |
| 2 | $2.5\times10^{-3}$ | $1.2\times10^{7}$ | $2.84\times10^{-2}$ | $4.4\times10^{-1}$ | $3.5\times10^{-8}$ | $7.5\times10^{7}$ |
| 3 | $1.3\times10^{-3}$ | $7.7\times10^{6}$ | $2.92\times10^{-2}$ | $3.3\times10^{-1}$ | $4.3\times10^{-8}$ | $9.2\times10^{7}$ |
| 4 | $6.3\times10^{-4}$ | $4.4\times10^{6}$ | $2.06\times10^{-2}$ | $2.1\times10^{-1}$ | $4.9\times10^{-8}$ | $1.0\times10^{8}$ |
| 5 | $3.1\times10^{-4}$ | $2.3\times10^{6}$ | $1.27\times10^{-2}$ | $1.2\times10^{-1}$ | $5.3\times10^{-8}$ | $1.1\times10^{8}$ |
| 6 | $1.6\times10^{-4}$ | $1.2\times10^{6}$ | $6.56\times10^{-3}$ | $6.6\times10^{-2}$ | $5.5\times10^{-8}$ | $1.2\times10^{8}$ |
| 7 | $7.8\times10^{-5}$ | $6.1\times10^{5}$ | $3.60\times10^{-3}$ | $3.4\times10^{-2}$ | $5.5\times10^{-8}$ | $1.2\times10^{8}$ |
| 8 | $3.9\times10^{-5}$ | $3.2\times10^{5}$ | $2.19\times10^{-3}$ | $1.8\times10^{-2}$ | $5.7\times10^{-8}$ | $1.2\times10^{8}$ |
| 9 | $2.0\times10^{-5}$ | $1.6\times10^{5}$ | $9.86\times10^{-4}$ | $8.9\times10^{-3}$ | $5.7\times10^{-8}$ | $1.2\times10^{8}$ |
| 10 | $9.8\times10^{-6}$ | $7.8\times10^{4}$ | $5.25\times10^{-4}$ | $4.1\times10^{-3}$ | $5.3\times10^{-8}$ | $1.2\times10^{8}$ |
| 11 | $4.9\times10^{-6}$ | $1.6\times10^{4}$ | $-2.84\times10^{-4}$ | $1.5\times10^{-3}$ | $9.3\times10^{-8}$ | $4.8\times10^{7}$ |
| 12 | $2.4\times10^{-6}$ | $1.0\times10^{3}$ | $6.09\times10^{-4}$ | $1.4\times10^{-4}$ | $1.4\times10^{-7}$ | $6.1\times10^{6}$ |
| $\sum$ | | | $9.81\times10^{-1}$ | | $7.1\times10^{-7}$ | $1.1\times10^{9}$ |

Table 109: $\varepsilon = 0.1$, $\Delta t_1 = 2.50 \times 10^{-3}$

| $\ell$ | $\Delta t_\ell$ | $P_\ell$ | $\mathbb{E}[\hat{F}_\ell - \hat{F}_{\ell-1}]$ | $\mathbb{V}[\hat{F}_\ell - \hat{F}_{\ell-1}]$ | $\mathbb{V}[\hat{Y}_\ell]$ | $P_\ell C_\ell$ |
|---|---|---|---|---|---|---|
| 0 | $5.0\times10^{-1}$ | $4.6\times10^{8}$ | $9.90\times10^{-1}$ | $2.0\times10^{0}$ | $4.3\times10^{-9}$ | $9.2\times10^{6}$ |
| 1 | $2.5\times10^{-3}$ | $1.1\times10^{7}$ | $-8.62\times10^{-2}$ | $2.3\times10^{-1}$ | $2.1\times10^{-8}$ | $4.4\times10^{7}$ |
| 2 | $1.3\times10^{-3}$ | $7.7\times10^{6}$ | $2.88\times10^{-2}$ | $3.3\times10^{-1}$ | $4.3\times10^{-8}$ | $9.3\times10^{7}$ |
| 3 | $6.3\times10^{-4}$ | $4.4\times10^{6}$ | $2.08\times10^{-2}$ | $2.1\times10^{-1}$ | $4.9\times10^{-8}$ | $1.1\times10^{8}$ |
| 4 | $3.1\times10^{-4}$ | $2.4\times10^{6}$ | $1.26\times10^{-2}$ | $1.2\times10^{-1}$ | $5.2\times10^{-8}$ | $1.1\times10^{8}$ |
| 5 | $1.6\times10^{-4}$ | $1.2\times10^{6}$ | $6.44\times10^{-3}$ | $6.6\times10^{-2}$ | $5.4\times10^{-8}$ | $1.2\times10^{8}$ |
| 6 | $7.8\times10^{-5}$ | $6.2\times10^{5}$ | $3.57\times10^{-3}$ | $3.4\times10^{-2}$ | $5.5\times10^{-8}$ | $1.2\times10^{8}$ |
| 7 | $3.9\times10^{-5}$ | $3.1\times10^{5}$ | $1.71\times10^{-3}$ | $1.7\times10^{-2}$ | $5.4\times10^{-8}$ | $1.2\times10^{8}$ |
| 8 | $2.0\times10^{-5}$ | $1.5\times10^{5}$ | $8.92\times10^{-4}$ | $8.0\times10^{-3}$ | $5.3\times10^{-8}$ | $1.2\times10^{8}$ |
| 9 | $9.8\times10^{-6}$ | $8.0\times10^{4}$ | $4.59\times10^{-4}$ | $4.0\times10^{-3}$ | $5.0\times10^{-8}$ | $1.2\times10^{8}$ |
| 10 | $4.9\times10^{-6}$ | $4.3\times10^{4}$ | $3.95\times10^{-5}$ | $1.8\times10^{-3}$ | $4.1\times10^{-8}$ | $1.3\times10^{8}$ |
| 11 | $2.4\times10^{-6}$ | $1.0\times10^{3}$ | $4.06\times10^{-5}$ | $8.3\times10^{-4}$ | $8.3\times10^{-7}$ | $6.1\times10^{6}$ |
| $\sum$ | | | $9.79\times10^{-1}$ | | $1.3\times10^{-6}$ | $1.1\times10^{9}$ |

Table 110: $\varepsilon = 0.1$, $\Delta t_1 = 1.25 \times 10^{-3}$

| $\ell$ | $\Delta t_\ell$ | $P_\ell$ | $\mathbb{E}[\hat{F}_\ell - \hat{F}_{\ell-1}]$ | $\mathbb{V}[\hat{F}_\ell - \hat{F}_{\ell-1}]$ | $\mathbb{V}[\hat{Y}_\ell]$ | $P_\ell C_\ell$ |
|---|---|---|---|---|---|---|
| 0 | $5.0\times10^{-1}$ | $4.8\times10^{8}$ | $9.90\times10^{-1}$ | $2.0\times10^{0}$ | $4.1\times10^{-9}$ | $9.6\times10^{6}$ |
| 1 | $1.3\times10^{-3}$ | $8.4\times10^{6}$ | $-5.71\times10^{-2}$ | $2.4\times10^{-1}$ | $2.9\times10^{-8}$ | $6.7\times10^{7}$ |
| 2 | $6.3\times10^{-4}$ | $4.5\times10^{6}$ | $2.07\times10^{-2}$ | $2.1\times10^{-1}$ | $4.7\times10^{-8}$ | $1.1\times10^{8}$ |
| 3 | $3.1\times10^{-4}$ | $2.4\times10^{6}$ | $1.28\times10^{-2}$ | $1.2\times10^{-1}$ | $5.0\times10^{-8}$ | $1.2\times10^{8}$ |
| 4 | $1.6\times10^{-4}$ | $1.3\times10^{6}$ | $6.82\times10^{-3}$ | $6.5\times10^{-2}$ | $5.2\times10^{-8}$ | $1.2\times10^{8}$ |
| 5 | $7.8\times10^{-5}$ | $6.4\times10^{5}$ | $3.55\times10^{-3}$ | $3.3\times10^{-2}$ | $5.2\times10^{-8}$ | $1.2\times10^{8}$ |
| 6 | $3.9\times10^{-5}$ | $3.2\times10^{5}$ | $1.70\times10^{-3}$ | $1.7\times10^{-2}$ | $5.4\times10^{-8}$ | $1.2\times10^{8}$ |
| 7 | $2.0\times10^{-5}$ | $1.6\times10^{5}$ | $1.09\times10^{-3}$ | $8.9\times10^{-3}$ | $5.4\times10^{-8}$ | $1.3\times10^{8}$ |
| 8 | $9.8\times10^{-6}$ | $8.4\times10^{4}$ | $8.01\times10^{-4}$ | $4.5\times10^{-3}$ | $5.4\times10^{-8}$ | $1.3\times10^{8}$ |
| 9 | $4.9\times10^{-6}$ | $7.2\times10^{4}$ | $2.07\times10^{-4}$ | $2.9\times10^{-3}$ | $4.1\times10^{-8}$ | $2.2\times10^{8}$ |
| 10 | $2.4\times10^{-6}$ | $1.6\times10^{4}$ | $-1.16\times10^{-4}$ | $8.1\times10^{-4}$ | $5.2\times10^{-8}$ | $9.6\times10^{7}$ |
| 11 | $1.2\times10^{-6}$ | $1.0\times10^{3}$ | $1.25\times10^{-4}$ | $9.9\times10^{-5}$ | $9.9\times10^{-8}$ | $1.2\times10^{7}$ |
| $\sum$ | | | $9.80\times10^{-1}$ | | $5.9\times10^{-7}$ | $1.3\times10^{9}$ |

Table 111: $\varepsilon = 0.1$, $\Delta t_1 = 6.25 \times 10^{-4}$

| $\ell$ | $\Delta t_\ell$ | $P_\ell$ | $\mathbb{E}[\hat{F}_\ell - \hat{F}_{\ell-1}]$ | $\mathbb{V}[\hat{F}_\ell - \hat{F}_{\ell-1}]$ | $\mathbb{V}[\hat{Y}_\ell]$ | $P_\ell C_\ell$ |
|---|---|---|---|---|---|---|
| 0 | $5.0\times10^{-1}$ | $4.3\times10^{8}$ | $9.90\times10^{-1}$ | $2.0\times10^{0}$ | $4.6\times10^{-9}$ | $8.6\times10^{6}$ |
| 1 | $6.3\times10^{-4}$ | $5.5\times10^{6}$ | $-3.65\times10^{-2}$ | $2.5\times10^{-1}$ | $4.6\times10^{-8}$ | $8.8\times10^{7}$ |
| 2 | $3.1\times10^{-4}$ | $2.2\times10^{6}$ | $1.23\times10^{-2}$ | $1.2\times10^{-1}$ | $5.6\times10^{-8}$ | $1.1\times10^{8}$ |
| 3 | $1.6\times10^{-4}$ | $1.1\times10^{6}$ | $6.66\times10^{-3}$ | $6.6\times10^{-2}$ | $5.8\times10^{-8}$ | $1.1\times10^{8}$ |
| 4 | $7.8\times10^{-5}$ | $5.8\times10^{5}$ | $3.44\times10^{-3}$ | $3.5\times10^{-2}$ | $6.0\times10^{-8}$ | $1.1\times10^{8}$ |
| 5 | $3.9\times10^{-5}$ | $3.0\times10^{5}$ | $1.29\times10^{-3}$ | $1.8\times10^{-2}$ | $6.2\times10^{-8}$ | $1.1\times10^{8}$ |
| 6 | $2.0\times10^{-5}$ | $1.4\times10^{5}$ | $6.80\times10^{-4}$ | $8.6\times10^{-3}$ | $6.1\times10^{-8}$ | $1.1\times10^{8}$ |
| 7 | $9.8\times10^{-6}$ | $6.8\times10^{4}$ | $4.20\times10^{-4}$ | $5.4\times10^{-3}$ | $8.0\times10^{-8}$ | $1.0\times10^{8}$ |
| 8 | $4.9\times10^{-6}$ | $6.3\times10^{4}$ | $1.80\times10^{-4}$ | $2.6\times10^{-3}$ | $4.1\times10^{-8}$ | $1.9\times10^{8}$ |
| 9 | $2.4\times10^{-6}$ | $1.0\times10^{3}$ | $6.53\times10^{-4}$ | $1.3\times10^{-3}$ | $1.3\times10^{-6}$ | $6.1\times10^{6}$ |
| $\sum$ | | | $9.79\times10^{-1}$ | | $1.8\times10^{-6}$ | $9.5\times10^{8}$ |

Table 112: $\varepsilon = 0.1$, $\Delta t_1 = 3.13 \times 10^{-4}$

| $\ell$ | $\Delta t_\ell$ | $P_\ell$ | $\mathbb{E}[\hat{F}_\ell - \hat{F}_{\ell-1}]$ | $\mathbb{V}[\hat{F}_\ell - \hat{F}_{\ell-1}]$ | $\mathbb{V}[\hat{Y}_\ell]$ | $P_\ell C_\ell$ |
|---|---|---|---|---|---|---|
| 0 | $5.0\times10^{-1}$ | $4.1\times10^{8}$ | $9.90\times10^{-1}$ | $2.0\times10^{0}$ | $4.8\times10^{-9}$ | $8.1\times10^{6}$ |
| 1 | $3.1\times10^{-4}$ | $3.7\times10^{6}$ | $-2.39\times10^{-2}$ | $2.6\times10^{-1}$ | $7.1\times10^{-8}$ | $1.2\times10^{8}$ |
| 2 | $1.6\times10^{-4}$ | $1.1\times10^{6}$ | $6.89\times10^{-3}$ | $6.7\times10^{-2}$ | $6.2\times10^{-8}$ | $1.0\times10^{8}$ |
| 3 | $7.8\times10^{-5}$ | $5.4\times10^{5}$ | $3.07\times10^{-3}$ | $3.4\times10^{-2}$ | $6.3\times10^{-8}$ | $1.0\times10^{8}$ |
| 4 | $3.9\times10^{-5}$ | $2.7\times10^{5}$ | $1.89\times10^{-3}$ | $1.7\times10^{-2}$ | $6.2\times10^{-8}$ | $1.0\times10^{8}$ |
| 5 | $2.0\times10^{-5}$ | $1.3\times10^{5}$ | $1.32\times10^{-3}$ | $8.5\times10^{-3}$ | $6.3\times10^{-8}$ | $1.0\times10^{8}$ |
| 6 | $9.8\times10^{-6}$ | $6.3\times10^{4}$ | $5.73\times10^{-4}$ | $3.5\times10^{-3}$ | $5.6\times10^{-8}$ | $9.7\times10^{7}$ |
| 7 | $4.9\times10^{-6}$ | $2.9\times10^{4}$ | $3.18\times10^{-4}$ | $1.7\times10^{-3}$ | $5.8\times10^{-8}$ | $8.9\times10^{7}$ |
| 8 | $2.4\times10^{-6}$ | $1.8\times10^{4}$ | $1.58\times10^{-4}$ | $6.3\times10^{-4}$ | $3.4\times10^{-8}$ | $1.1\times10^{8}$ |
| 9 | $1.2\times10^{-6}$ | $1.0\times10^{3}$ | $3.81\times10^{-4}$ | $8.9\times10^{-5}$ | $8.9\times10^{-8}$ | $1.2\times10^{7}$ |
| $\sum$ | | | $9.81\times10^{-1}$ | | $5.6\times10^{-7}$ | $8.5\times10^{8}$ |

Table 113: $\varepsilon = 0.1$, $\Delta t_1 = 1.56 \times 10^{-4}$

| $\ell$ | $\Delta t_\ell$ | $P_\ell$ | $\mathbb{E}[\hat{F}_\ell - \hat{F}_{\ell-1}]$ | $\mathbb{V}[\hat{F}_\ell - \hat{F}_{\ell-1}]$ | $\mathbb{V}[\hat{Y}_\ell]$ | $P_\ell C_\ell$ |
|---|---|---|---|---|---|---|
| 0 | $5.0\times10^{-1}$ | $3.7\times10^{8}$ | $9.90\times10^{-1}$ | $2.0\times10^{0}$ | $5.3\times10^{-9}$ | $7.4\times10^{6}$ |
| 1 | $1.6\times10^{-4}$ | $2.4\times10^{6}$ | $-1.76\times10^{-2}$ | $2.7\times10^{-1}$ | $1.1\times10^{-7}$ | $1.5\times10^{8}$ |
| 2 | $7.8\times10^{-5}$ | $4.9\times10^{5}$ | $3.33\times10^{-3}$ | $3.3\times10^{-2}$ | $6.7\times10^{-8}$ | $9.4\times10^{7}$ |
| 3 | $3.9\times10^{-5}$ | $2.6\times10^{5}$ | $2.37\times10^{-3}$ | $1.8\times10^{-2}$ | $7.0\times10^{-8}$ | $9.9\times10^{7}$ |
| 4 | $2.0\times10^{-5}$ | $1.3\times10^{5}$ | $8.88\times10^{-4}$ | $9.7\times10^{-3}$ | $7.3\times10^{-8}$ | $1.0\times10^{8}$ |
| 5 | $9.8\times10^{-6}$ | $5.5\times10^{4}$ | $4.89\times10^{-4}$ | $3.1\times10^{-3}$ | $5.6\times10^{-8}$ | $8.5\times10^{7}$ |
| 6 | $4.9\times10^{-6}$ | $2.6\times10^{4}$ | $4.53\times10^{-4}$ | $2.1\times10^{-3}$ | $8.0\times10^{-8}$ | $8.0\times10^{7}$ |
| 7 | $2.4\times10^{-6}$ | $1.3\times10^{4}$ | $4.67\times10^{-4}$ | $8.5\times10^{-4}$ | $6.6\times10^{-8}$ | $7.9\times10^{7}$ |
| 8 | $1.2\times10^{-6}$ | $1.0\times10^{3}$ | $-3.57\times10^{-5}$ | $9.4\times10^{-5}$ | $9.4\times10^{-8}$ | $1.2\times10^{7}$ |
| $\sum$ | | | $9.80\times10^{-1}$ | | $6.2\times10^{-7}$ | $7.1\times10^{8}$ |

Table 114: $\varepsilon = 0.1$, $\Delta t_1 = 7.81 \times 10^{-5}$

| $\ell$ | $\Delta t_\ell$ | $P_\ell$ | $\mathbb{E}[\hat{F}_\ell - \hat{F}_{\ell-1}]$ | $\mathbb{V}[\hat{F}_\ell - \hat{F}_{\ell-1}]$ | $\mathbb{V}[\hat{Y}_\ell]$ | $P_\ell C_\ell$ |
|---|---|---|---|---|---|---|
| 0 | $5.0\times10^{-1}$ | $3.5\times10^{8}$ | $9.90\times10^{-1}$ | $2.0\times10^{0}$ | $5.5\times10^{-9}$ | $7.1\times10^{6}$ |
| 1 | $7.8\times10^{-5}$ | $1.6\times10^{6}$ | $-1.34\times10^{-2}$ | $2.7\times10^{-1}$ | $1.6\times10^{-7}$ | $2.1\times10^{8}$ |
| 2 | $3.9\times10^{-5}$ | $2.4\times10^{5}$ | $1.66\times10^{-3}$ | $1.7\times10^{-2}$ | $7.0\times10^{-8}$ | $9.1\times10^{7}$ |
| 3 | $2.0\times10^{-5}$ | $1.3\times10^{5}$ | $5.31\times10^{-4}$ | $9.6\times10^{-3}$ | $7.6\times10^{-8}$ | $9.7\times10^{7}$ |
| 4 | $9.8\times10^{-6}$ | $6.6\times10^{4}$ | $7.28\times10^{-4}$ | $4.9\times10^{-3}$ | $7.5\times10^{-8}$ | $1.0\times10^{8}$ |
| 5 | $4.9\times10^{-6}$ | $3.0\times10^{4}$ | $3.17\times10^{-4}$ | $2.7\times10^{-3}$ | $9.2\times10^{-8}$ | $9.1\times10^{7}$ |
| 6 | $2.4\times10^{-6}$ | $7.3\times10^{3}$ | $-1.49\times10^{-4}$ | $1.8\times10^{-3}$ | $2.5\times10^{-7}$ | $4.5\times10^{7}$ |
| 7 | $1.2\times10^{-6}$ | $1.0\times10^{3}$ | $-2.45\times10^{-4}$ | $3.2\times10^{-4}$ | $3.2\times10^{-7}$ | $1.2\times10^{7}$ |
| $\sum$ | | | $9.79\times10^{-1}$ | | $1.1\times10^{-6}$ | $6.5\times10^{8}$ |

Table 115: $\varepsilon = 0.1$, $\Delta t_1 = 3.91 \times 10^{-5}$

| $\ell$ | $\Delta t_\ell$ | $P_\ell$ | $\mathbb{E}[\hat{F}_\ell - \hat{F}_{\ell-1}]$ | $\mathbb{V}[\hat{F}_\ell - \hat{F}_{\ell-1}]$ | $\mathbb{V}[\hat{Y}_\ell]$ | $P_\ell C_\ell$ |
|---|---|---|---|---|---|---|
| 0 | $5.0\times10^{-1}$ | $3.5\times10^{8}$ | $9.90\times10^{-1}$ | $2.0\times10^{0}$ | $5.5\times10^{-9}$ | $7.1\times10^{6}$ |
| 1 | $3.9\times10^{-5}$ | $1.2\times10^{6}$ | $-1.17\times10^{-2}$ | $2.7\times10^{-1}$ | $2.3\times10^{-7}$ | $3.0\times10^{8}$ |
| 2 | $2.0\times10^{-5}$ | $1.2\times10^{5}$ | $7.53\times10^{-4}$ | $8.6\times10^{-3}$ | $7.2\times10^{-8}$ | $9.2\times10^{7}$ |
| 3 | $9.8\times10^{-6}$ | $6.2\times10^{4}$ | $4.54\times10^{-4}$ | $4.5\times10^{-3}$ | $7.3\times10^{-8}$ | $9.5\times10^{7}$ |
| 4 | $4.9\times10^{-6}$ | $2.2\times10^{4}$ | $1.61\times10^{-4}$ | $1.1\times10^{-3}$ | $5.2\times10^{-8}$ | $6.7\times10^{7}$ |
| 5 | $2.4\times10^{-6}$ | $1.3\times10^{4}$ | $4.18\times10^{-4}$ | $1.4\times10^{-3}$ | $1.1\times10^{-7}$ | $7.9\times10^{7}$ |
| 6 | $1.2\times10^{-6}$ | $1.0\times10^{3}$ | $4.58\times10^{-5}$ | $7.2\times10^{-5}$ | $7.2\times10^{-8}$ | $1.2\times10^{7}$ |
| $\sum$ | | | $9.80\times10^{-1}$ | | $6.1\times10^{-7}$ | $6.5\times10^{8}$ |

Table 116: $\varepsilon = 0.1$, $\Delta t_1 = 1.95 \times 10^{-5}$

| $\ell$ | $\Delta t_\ell$ | $P_\ell$ | $\mathbb{E}[\hat{F}_\ell - \hat{F}_{\ell-1}]$ | $\mathbb{V}[\hat{F}_\ell - \hat{F}_{\ell-1}]$ | $\mathbb{V}[\hat{Y}_\ell]$ | $P_\ell C_\ell$ |
|---|---|---|---|---|---|---|
| 0 | $5.0\times10^{-1}$ | $3.6\times10^{8}$ | $9.90\times10^{-1}$ | $2.0\times10^{0}$ | $5.5\times10^{-9}$ | $7.1\times10^{6}$ |
| 1 | $2.0\times10^{-5}$ | $8.3\times10^{5}$ | $-1.12\times10^{-2}$ | $2.7\times10^{-1}$ | $3.3\times10^{-7}$ | $4.3\times10^{8}$ |
| 2 | $9.8\times10^{-6}$ | $5.4\times10^{4}$ | $8.53\times10^{-4}$ | $3.5\times10^{-3}$ | $6.5\times10^{-8}$ | $8.3\times10^{7}$ |
| 3 | $4.9\times10^{-6}$ | $3.1\times10^{4}$ | $2.60\times10^{-4}$ | $2.3\times10^{-3}$ | $7.3\times10^{-8}$ | $9.7\times10^{7}$ |
| 4 | $2.4\times10^{-6}$ | $6.2\times10^{3}$ | $4.44\times10^{-4}$ | $5.3\times10^{-4}$ | $8.7\times10^{-8}$ | $3.8\times10^{7}$ |
| 5 | $1.2\times10^{-6}$ | $1.0\times10^{3}$ | $1.33\times10^{-4}$ | $2.1\times10^{-4}$ | $2.1\times10^{-7}$ | $1.2\times10^{7}$ |
| $\sum$ | | | $9.81\times10^{-1}$ | | $7.6\times10^{-7}$ | $6.6\times10^{8}$ |

## 2.6 Combined correlation, $\varepsilon = 0.05$

Table 117: $\varepsilon = 0.05$, $\Delta t_1 = 2.50 \times 10^{-3}$

| $\ell$ | $\Delta t_\ell$ | $P_\ell$ | $\mathbb{E}[\hat{F}_\ell - \hat{F}_{\ell-1}]$ | $\mathbb{V}[\hat{F}_\ell - \hat{F}_{\ell-1}]$ | $\mathbb{V}[\hat{Y}_\ell]$ | $P_\ell C_\ell$ |
|---|---|---|---|---|---|---|
| 0 | $5.0\times10^{-1}$ | $1.1\times10^{9}$ | $9.98\times10^{-1}$ | $2.0\times10^{0}$ | $1.9\times10^{-9}$ | $2.1\times10^{7}$ |
| 1 | $2.5\times10^{-3}$ | $1.4\times10^{7}$ | $-1.25\times10^{-1}$ | $6.6\times10^{-2}$ | $4.8\times10^{-9}$ | $5.5\times10^{7}$ |
| 2 | $1.3\times10^{-3}$ | $2.1\times10^{7}$ | $1.31\times10^{-2}$ | $4.8\times10^{-1}$ | $2.2\times10^{-8}$ | $2.6\times10^{8}$ |
| 3 | $6.3\times10^{-4}$ | $1.5\times10^{7}$ | $3.05\times10^{-2}$ | $4.5\times10^{-1}$ | $3.0\times10^{-8}$ | $3.5\times10^{8}$ |
| 4 | $3.1\times10^{-4}$ | $9.0\times10^{6}$ | $3.00\times10^{-2}$ | $3.4\times10^{-1}$ | $3.8\times10^{-8}$ | $4.3\times10^{8}$ |
| 5 | $1.6\times10^{-4}$ | $5.1\times10^{6}$ | $2.15\times10^{-2}$ | $2.2\times10^{-1}$ | $4.2\times10^{-8}$ | $4.9\times10^{8}$ |
| 6 | $7.8\times10^{-5}$ | $2.7\times10^{6}$ | $1.31\times10^{-2}$ | $1.3\times10^{-1}$ | $4.6\times10^{-8}$ | $5.3\times10^{8}$ |
| 7 | $3.9\times10^{-5}$ | $1.4\times10^{6}$ | $7.00\times10^{-3}$ | $6.7\times10^{-2}$ | $4.7\times10^{-8}$ | $5.5\times10^{8}$ |
| 8 | $2.0\times10^{-5}$ | $7.2\times10^{5}$ | $3.99\times10^{-3}$ | $3.5\times10^{-2}$ | $4.8\times10^{-8}$ | $5.6\times10^{8}$ |
| 9 | $9.8\times10^{-6}$ | $3.7\times10^{5}$ | $1.75\times10^{-3}$ | $1.8\times10^{-2}$ | $4.9\times10^{-8}$ | $5.6\times10^{8}$ |
| 10 | $4.9\times10^{-6}$ | $1.9\times10^{5}$ | $8.12\times10^{-4}$ | $9.2\times10^{-3}$ | $4.9\times10^{-8}$ | $5.7\times10^{8}$ |
| 11 | $2.4\times10^{-6}$ | $9.1\times10^{4}$ | $7.86\times10^{-4}$ | $4.4\times10^{-3}$ | $4.9\times10^{-8}$ | $5.6\times10^{8}$ |
| 12 | $1.2\times10^{-6}$ | $6.1\times10^{4}$ | $3.70\times10^{-4}$ | $1.8\times10^{-3}$ | $3.0\times10^{-8}$ | $7.4\times10^{8}$ |
| 13 | $6.1\times10^{-7}$ | $1.3\times10^{4}$ | $9.19\times10^{-6}$ | $6.8\times10^{-4}$ | $5.1\times10^{-8}$ | $3.3\times10^{8}$ |
| 14 | $3.1\times10^{-7}$ | $1.0\times10^{3}$ | $7.65\times10^{-5}$ | $3.3\times10^{-4}$ | $3.3\times10^{-7}$ | $4.9\times10^{7}$ |
| $\sum$ | | | $9.96\times10^{-1}$ | | $8.4\times10^{-7}$ | $6.1\times10^{9}$ |

Table 118: $\varepsilon = 0.05$, $\Delta t_1 = 1.25 \times 10^{-3}$

| $\ell$ | $\Delta t_\ell$ | $P_\ell$ | $\mathbb{E}[\hat{F}_\ell - \hat{F}_{\ell-1}]$ | $\mathbb{V}[\hat{F}_\ell - \hat{F}_{\ell-1}]$ | $\mathbb{V}[\hat{Y}_\ell]$ | $P_\ell C_\ell$ |
|---|---|---|---|---|---|---|
| 0 | $5.0\times10^{-1}$ | $1.1\times10^{9}$ | $9.98\times10^{-1}$ | $2.0\times10^{0}$ | $1.8\times10^{-9}$ | $2.2\times10^{7}$ |
| 1 | $1.3\times10^{-3}$ | $1.0\times10^{7}$ | $-1.12\times10^{-1}$ | $7.0\times10^{-2}$ | $6.8\times10^{-9}$ | $8.3\times10^{7}$ |
| 2 | $6.3\times10^{-4}$ | $1.5\times10^{7}$ | $3.08\times10^{-2}$ | $4.5\times10^{-1}$ | $3.0\times10^{-8}$ | $3.6\times10^{8}$ |
| 3 | $3.1\times10^{-4}$ | $9.2\times10^{6}$ | $3.02\times10^{-2}$ | $3.4\times10^{-1}$ | $3.7\times10^{-8}$ | $4.4\times10^{8}$ |
| 4 | $1.6\times10^{-4}$ | $5.2\times10^{6}$ | $2.19\times10^{-2}$ | $2.2\times10^{-1}$ | $4.2\times10^{-8}$ | $5.0\times10^{8}$ |
| 5 | $7.8\times10^{-5}$ | $2.8\times10^{6}$ | $1.30\times10^{-2}$ | $1.2\times10^{-1}$ | $4.4\times10^{-8}$ | $5.4\times10^{8}$ |
| 6 | $3.9\times10^{-5}$ | $1.5\times10^{6}$ | $7.11\times10^{-3}$ | $6.8\times10^{-2}$ | $4.6\times10^{-8}$ | $5.6\times10^{8}$ |
| 7 | $2.0\times10^{-5}$ | $7.5\times10^{5}$ | $3.39\times10^{-3}$ | $3.6\times10^{-2}$ | $4.8\times10^{-8}$ | $5.7\times10^{8}$ |
| 8 | $9.8\times10^{-6}$ | $3.8\times10^{5}$ | $2.35\times10^{-3}$ | $1.8\times10^{-2}$ | $4.8\times10^{-8}$ | $5.8\times10^{8}$ |
| 9 | $4.9\times10^{-6}$ | $1.9\times10^{5}$ | $1.18\times10^{-3}$ | $9.4\times10^{-3}$ | $5.0\times10^{-8}$ | $5.8\times10^{8}$ |
| 10 | $2.4\times10^{-6}$ | $9.5\times10^{4}$ | $3.56\times10^{-4}$ | $4.5\times10^{-3}$ | $4.7\times10^{-8}$ | $5.9\times10^{8}$ |
| 11 | $1.2\times10^{-6}$ | $4.8\times10^{4}$ | $4.08\times10^{-4}$ | $2.2\times10^{-3}$ | $4.6\times10^{-8}$ | $5.8\times10^{8}$ |
| 12 | $6.1\times10^{-7}$ | $2.6\times10^{4}$ | $-1.47\times10^{-4}$ | $1.4\times10^{-3}$ | $5.2\times10^{-8}$ | $6.5\times10^{8}$ |
| 13 | $3.1\times10^{-7}$ | $1.0\times10^{3}$ | $-9.86\times10^{-5}$ | $5.7\times10^{-4}$ | $5.7\times10^{-7}$ | $4.9\times10^{7}$ |
| $\sum$ | | | $9.96\times10^{-1}$ | | $1.1\times10^{-6}$ | $6.1\times10^{9}$ |

Table 119: $\varepsilon = 0.05$, $\Delta t_1 = 6.25 \times 10^{-4}$

| $\ell$ | $\Delta t_\ell$ | $P_\ell$ | $\mathbb{E}[\hat{F}_\ell - \hat{F}_{\ell-1}]$ | $\mathbb{V}[\hat{F}_\ell - \hat{F}_{\ell-1}]$ | $\mathbb{V}[\hat{Y}_\ell]$ | $P_\ell C_\ell$ |
|---|---|---|---|---|---|---|
| 0 | $5.0\times10^{-1}$ | $9.5\times10^{8}$ | $9.98\times10^{-1}$ | $2.0\times10^{0}$ | $2.1\times10^{-9}$ | $1.9\times10^{7}$ |
| 1 | $6.3\times10^{-4}$ | $6.2\times10^{6}$ | $-8.16\times10^{-2}$ | $6.8\times10^{-2}$ | $1.1\times10^{-8}$ | $9.9\times10^{7}$ |
| 2 | $3.1\times10^{-4}$ | $8.0\times10^{6}$ | $3.04\times10^{-2}$ | $3.4\times10^{-1}$ | $4.2\times10^{-8}$ | $3.8\times10^{8}$ |
| 3 | $1.6\times10^{-4}$ | $4.5\times10^{6}$ | $2.14\times10^{-2}$ | $2.2\times10^{-1}$ | $4.8\times10^{-8}$ | $4.3\times10^{8}$ |
| 4 | $7.8\times10^{-5}$ | $2.4\times10^{6}$ | $1.29\times10^{-2}$ | $1.2\times10^{-1}$ | $5.1\times10^{-8}$ | $4.7\times10^{8}$ |
| 5 | $3.9\times10^{-5}$ | $1.3\times10^{6}$ | $6.91\times10^{-3}$ | $6.8\times10^{-2}$ | $5.4\times10^{-8}$ | $4.8\times10^{8}$ |
| 6 | $2.0\times10^{-5}$ | $6.4\times10^{5}$ | $3.80\times10^{-3}$ | $3.5\times10^{-2}$ | $5.4\times10^{-8}$ | $4.9\times10^{8}$ |
| 7 | $9.8\times10^{-6}$ | $3.3\times10^{5}$ | $2.57\times10^{-3}$ | $1.9\times10^{-2}$ | $5.6\times10^{-8}$ | $5.1\times10^{8}$ |
| 8 | $4.9\times10^{-6}$ | $1.6\times10^{5}$ | $1.13\times10^{-3}$ | $8.7\times10^{-3}$ | $5.4\times10^{-8}$ | $5.0\times10^{8}$ |
| 9 | $2.4\times10^{-6}$ | $8.2\times10^{4}$ | $5.34\times10^{-4}$ | $4.6\times10^{-3}$ | $5.6\times10^{-8}$ | $5.1\times10^{8}$ |
| 10 | $1.2\times10^{-6}$ | $5.1\times10^{4}$ | $2.67\times10^{-4}$ | $2.4\times10^{-3}$ | $4.6\times10^{-8}$ | $6.3\times10^{8}$ |
| 11 | $6.1\times10^{-7}$ | $1.0\times10^{3}$ | $-3.94\times10^{-4}$ | $3.6\times10^{-4}$ | $3.6\times10^{-7}$ | $2.5\times10^{7}$ |
| $\sum$ | | | $9.95\times10^{-1}$ | | $8.4\times10^{-7}$ | $4.5\times10^{9}$ |

Table 120: $\varepsilon = 0.05$, $\Delta t_1 = 3.13 \times 10^{-4}$

| $\ell$ | $\Delta t_\ell$ | $P_\ell$ | $\mathbb{E}[\hat{F}_\ell - \hat{F}_{\ell-1}]$ | $\mathbb{V}[\hat{F}_\ell - \hat{F}_{\ell-1}]$ | $\mathbb{V}[\hat{Y}_\ell]$ | $P_\ell C_\ell$ |
|---|---|---|---|---|---|---|
| 0 | $5.0\times10^{-1}$ | $9.3\times10^{8}$ | $9.98\times10^{-1}$ | $2.0\times10^{0}$ | $2.1\times10^{-9}$ | $1.9\times10^{7}$ |
| 1 | $3.1\times10^{-4}$ | $4.3\times10^{6}$ | $-5.13\times10^{-2}$ | $6.6\times10^{-2}$ | $1.6\times10^{-8}$ | $1.4\times10^{8}$ |
| 2 | $1.6\times10^{-4}$ | $4.5\times10^{6}$ | $2.12\times10^{-2}$ | $2.2\times10^{-1}$ | $4.9\times10^{-8}$ | $4.3\times10^{8}$ |
| 3 | $7.8\times10^{-5}$ | $2.4\times10^{6}$ | $1.27\times10^{-2}$ | $1.2\times10^{-1}$ | $5.2\times10^{-8}$ | $4.6\times10^{8}$ |
| 4 | $3.9\times10^{-5}$ | $1.2\times10^{6}$ | $7.28\times10^{-3}$ | $6.7\times10^{-2}$ | $5.4\times10^{-8}$ | $4.8\times10^{8}$ |
| 5 | $2.0\times10^{-5}$ | $6.4\times10^{5}$ | $3.65\times10^{-3}$ | $3.5\times10^{-2}$ | $5.6\times10^{-8}$ | $4.9\times10^{8}$ |
| 6 | $9.8\times10^{-6}$ | $3.2\times10^{5}$ | $2.15\times10^{-3}$ | $1.7\times10^{-2}$ | $5.5\times10^{-8}$ | $4.9\times10^{8}$ |
| 7 | $4.9\times10^{-6}$ | $1.6\times10^{5}$ | $9.01\times10^{-4}$ | $8.8\times10^{-3}$ | $5.6\times10^{-8}$ | $4.9\times10^{8}$ |
| 8 | $2.4\times10^{-6}$ | $8.6\times10^{4}$ | $-1.94\times10^{-6}$ | $5.0\times10^{-3}$ | $5.8\times10^{-8}$ | $5.3\times10^{8}$ |
| 9 | $1.2\times10^{-6}$ | $4.7\times10^{4}$ | $-6.14\times10^{-5}$ | $3.9\times10^{-3}$ | $8.2\times10^{-8}$ | $5.8\times10^{8}$ |
| 10 | $6.1\times10^{-7}$ | $1.2\times10^{4}$ | $3.23\times10^{-4}$ | $1.3\times10^{-3}$ | $1.1\times10^{-7}$ | $3.1\times10^{8}$ |
| 11 | $3.1\times10^{-7}$ | $1.0\times10^{3}$ | $-5.19\times10^{-4}$ | $2.3\times10^{-4}$ | $2.3\times10^{-7}$ | $4.9\times10^{7}$ |
| $\sum$ | | | $9.94\times10^{-1}$ | | $8.2\times10^{-7}$ | $4.4\times10^{9}$ |

Table 121: $\varepsilon = 0.05$, $\Delta t_1 = 1.56 \times 10^{-4}$

| $\ell$ | $\Delta t_\ell$ | $P_\ell$ | $\mathbb{E}[\hat{F}_\ell - \hat{F}_{\ell-1}]$ | $\mathbb{V}[\hat{F}_\ell - \hat{F}_{\ell-1}]$ | $\mathbb{V}[\hat{Y}_\ell]$ | $P_\ell C_\ell$ |
|---|---|---|---|---|---|---|
| 0 | $5.0\times10^{-1}$ | $1.0\times10^{9}$ | $9.98\times10^{-1}$ | $2.0\times10^{0}$ | $2.0\times10^{-9}$ | $2.0\times10^{7}$ |
| 1 | $1.6\times10^{-4}$ | $3.2\times10^{6}$ | $-3.02\times10^{-2}$ | $6.6\times10^{-2}$ | $2.1\times10^{-8}$ | $2.1\times10^{8}$ |
| 2 | $7.8\times10^{-5}$ | $2.6\times10^{6}$ | $1.28\times10^{-2}$ | $1.3\times10^{-1}$ | $4.9\times10^{-8}$ | $4.9\times10^{8}$ |
| 3 | $3.9\times10^{-5}$ | $1.3\times10^{6}$ | $6.94\times10^{-3}$ | $6.8\times10^{-2}$ | $5.1\times10^{-8}$ | $5.1\times10^{8}$ |
| 4 | $2.0\times10^{-5}$ | $6.8\times10^{5}$ | $3.58\times10^{-3}$ | $3.5\times10^{-2}$ | $5.2\times10^{-8}$ | $5.2\times10^{8}$ |
| 5 | $9.8\times10^{-6}$ | $3.5\times10^{5}$ | $1.93\times10^{-3}$ | $1.8\times10^{-2}$ | $5.2\times10^{-8}$ | $5.3\times10^{8}$ |
| 6 | $4.9\times10^{-6}$ | $1.7\times10^{5}$ | $1.04\times10^{-3}$ | $9.0\times10^{-3}$ | $5.2\times10^{-8}$ | $5.3\times10^{8}$ |
| 7 | $2.4\times10^{-6}$ | $9.2\times10^{4}$ | $4.36\times10^{-4}$ | $5.1\times10^{-3}$ | $5.6\times10^{-8}$ | $5.7\times10^{8}$ |
| 8 | $1.2\times10^{-6}$ | $4.4\times10^{4}$ | $2.87\times10^{-4}$ | $2.3\times10^{-3}$ | $5.2\times10^{-8}$ | $5.3\times10^{8}$ |
| 9 | $6.1\times10^{-7}$ | $2.0\times10^{4}$ | $-6.32\times10^{-6}$ | $9.3\times10^{-4}$ | $4.6\times10^{-8}$ | $5.0\times10^{8}$ |
| 10 | $3.1\times10^{-7}$ | $1.3\times10^{4}$ | $-1.26\times10^{-4}$ | $3.9\times10^{-4}$ | $3.0\times10^{-8}$ | $6.2\times10^{8}$ |
| 11 | $1.5\times10^{-7}$ | $1.0\times10^{3}$ | $-1.19\times10^{-4}$ | $1.1\times10^{-4}$ | $1.1\times10^{-7}$ | $9.8\times10^{7}$ |
| $\sum$ | | | $9.94\times10^{-1}$ | | $5.7\times10^{-7}$ | $5.1\times10^{9}$ |

Table 122: $\varepsilon = 0.05$, $\Delta t_1 = 7.81 \times 10^{-5}$

| $\ell$ | $\Delta t_\ell$ | $P_\ell$ | $\mathbb{E}[\hat{F}_\ell - \hat{F}_{\ell-1}]$ | $\mathbb{V}[\hat{F}_\ell - \hat{F}_{\ell-1}]$ | $\mathbb{V}[\hat{Y}_\ell]$ | $P_\ell C_\ell$ |
|---|---|---|---|---|---|---|
| 0 | $5.0\times10^{-1}$ | $7.9\times10^{8}$ | $9.98\times10^{-1}$ | $2.0\times10^{0}$ | $2.5\times10^{-9}$ | $1.6\times10^{7}$ |
| 1 | $7.8\times10^{-5}$ | $1.8\times10^{6}$ | $-1.68\times10^{-2}$ | $6.8\times10^{-2}$ | $3.7\times10^{-8}$ | $2.3\times10^{8}$ |
| 2 | $3.9\times10^{-5}$ | $1.0\times10^{6}$ | $6.90\times10^{-3}$ | $6.7\times10^{-2}$ | $6.4\times10^{-8}$ | $4.0\times10^{8}$ |
| 3 | $2.0\times10^{-5}$ | $5.4\times10^{5}$ | $3.27\times10^{-3}$ | $3.6\times10^{-2}$ | $6.6\times10^{-8}$ | $4.2\times10^{8}$ |
| 4 | $9.8\times10^{-6}$ | $2.7\times10^{5}$ | $1.72\times10^{-3}$ | $1.7\times10^{-2}$ | $6.5\times10^{-8}$ | $4.1\times10^{8}$ |
| 5 | $4.9\times10^{-6}$ | $1.4\times10^{5}$ | $7.61\times10^{-4}$ | $9.4\times10^{-3}$ | $6.7\times10^{-8}$ | $4.3\times10^{8}$ |
| 6 | $2.4\times10^{-6}$ | $6.9\times10^{4}$ | $9.36\times10^{-4}$ | $4.8\times10^{-3}$ | $6.9\times10^{-8}$ | $4.3\times10^{8}$ |
| 7 | $1.2\times10^{-6}$ | $3.6\times10^{4}$ | $5.32\times10^{-4}$ | $2.4\times10^{-3}$ | $6.8\times10^{-8}$ | $4.4\times10^{8}$ |
| 8 | $6.1\times10^{-7}$ | $1.5\times10^{4}$ | $2.03\times10^{-4}$ | $1.0\times10^{-3}$ | $6.9\times10^{-8}$ | $3.6\times10^{8}$ |
| 9 | $3.1\times10^{-7}$ | $1.0\times10^{3}$ | $-5.85\times10^{-4}$ | $3.0\times10^{-4}$ | $3.0\times10^{-7}$ | $4.9\times10^{7}$ |
| $\sum$ | | | $9.94\times10^{-1}$ | | $8.1\times10^{-7}$ | $3.2\times10^{9}$ |

Table 123: $\varepsilon = 0.05$, $\Delta t_1 = 3.91 \times 10^{-5}$

| $\ell$ | $\Delta t_\ell$ | $P_\ell$ | $\mathbb{E}[\hat{F}_\ell - \hat{F}_{\ell-1}]$ | $\mathbb{V}[\hat{F}_\ell - \hat{F}_{\ell-1}]$ | $\mathbb{V}[\hat{Y}_\ell]$ | $P_\ell C_\ell$ |
|---|---|---|---|---|---|---|
| 0 | $5.0\times10^{-1}$ | $7.7\times10^{8}$ | $9.98\times10^{-1}$ | $2.0\times10^{0}$ | $2.6\times10^{-9}$ | $1.5\times10^{7}$ |
| 1 | $3.9\times10^{-5}$ | $1.3\times10^{6}$ | $-1.00\times10^{-2}$ | $6.9\times10^{-2}$ | $5.5\times10^{-8}$ | $3.2\times10^{8}$ |
| 2 | $2.0\times10^{-5}$ | $5.2\times10^{5}$ | $3.70\times10^{-3}$ | $3.5\times10^{-2}$ | $6.8\times10^{-8}$ | $4.0\times10^{8}$ |
| 3 | $9.8\times10^{-6}$ | $2.6\times10^{5}$ | $1.95\times10^{-3}$ | $1.8\times10^{-2}$ | $6.8\times10^{-8}$ | $4.0\times10^{8}$ |
| 4 | $4.9\times10^{-6}$ | $1.3\times10^{5}$ | $1.35\times10^{-3}$ | $8.8\times10^{-3}$ | $6.7\times10^{-8}$ | $4.0\times10^{8}$ |
| 5 | $2.4\times10^{-6}$ | $7.0\times10^{4}$ | $6.91\times10^{-4}$ | $4.9\times10^{-3}$ | $7.1\times10^{-8}$ | $4.3\times10^{8}$ |
| 6 | $1.2\times10^{-6}$ | $3.4\times10^{4}$ | $-5.27\times10^{-6}$ | $2.2\times10^{-3}$ | $6.4\times10^{-8}$ | $4.2\times10^{8}$ |
| 7 | $6.1\times10^{-7}$ | $2.4\times10^{4}$ | $5.26\times10^{-4}$ | $1.4\times10^{-3}$ | $5.8\times10^{-8}$ | $5.9\times10^{8}$ |
| 8 | $3.1\times10^{-7}$ | $1.0\times10^{3}$ | $5.28\times10^{-4}$ | $9.8\times10^{-5}$ | $9.8\times10^{-8}$ | $4.9\times10^{7}$ |
| $\sum$ | | | $9.96\times10^{-1}$ | | $5.5\times10^{-7}$ | $3.0\times10^{9}$ |

Table 124: $\varepsilon = 0.05$, $\Delta t_1 = 1.95 \times 10^{-5}$

| $\ell$ | $\Delta t_\ell$ | $P_\ell$ | $\mathbb{E}[\hat{F}_\ell - \hat{F}_{\ell-1}]$ | $\mathbb{V}[\hat{F}_\ell - \hat{F}_{\ell-1}]$ | $\mathbb{V}[\hat{Y}_\ell]$ | $P_\ell C_\ell$ |
|---|---|---|---|---|---|---|
| 0 | $5.0\times10^{-1}$ | $9.6\times10^{8}$ | $9.97\times10^{-1}$ | $2.0\times10^{0}$ | $2.1\times10^{-9}$ | $1.9\times10^{7}$ |
| 1 | $2.0\times10^{-5}$ | $1.1\times10^{6}$ | $-6.45\times10^{-3}$ | $6.9\times10^{-2}$ | $6.2\times10^{-8}$ | $5.7\times10^{8}$ |
| 2 | $9.8\times10^{-6}$ | $3.3\times10^{5}$ | $1.89\times10^{-3}$ | $1.8\times10^{-2}$ | $5.5\times10^{-8}$ | $5.1\times10^{8}$ |
| 3 | $4.9\times10^{-6}$ | $1.6\times10^{5}$ | $1.06\times10^{-3}$ | $9.4\times10^{-3}$ | $5.8\times10^{-8}$ | $5.0\times10^{8}$ |
| 4 | $2.4\times10^{-6}$ | $7.7\times10^{4}$ | $4.14\times10^{-4}$ | $4.9\times10^{-3}$ | $6.4\times10^{-8}$ | $4.7\times10^{8}$ |
| 5 | $1.2\times10^{-6}$ | $4.3\times10^{4}$ | $2.92\times10^{-4}$ | $2.4\times10^{-3}$ | $5.5\times10^{-8}$ | $5.3\times10^{8}$ |
| 6 | $6.1\times10^{-7}$ | $2.6\times10^{4}$ | $5.23\times10^{-4}$ | $1.4\times10^{-3}$ | $5.5\times10^{-8}$ | $6.3\times10^{8}$ |
| 7 | $3.1\times10^{-7}$ | $2.8\times10^{4}$ | $-2.19\times10^{-4}$ | $5.6\times10^{-4}$ | $2.0\times10^{-8}$ | $1.4\times10^{9}$ |
| 8 | $1.5\times10^{-7}$ | $1.0\times10^{3}$ | $-6.50\times10^{-5}$ | $4.4\times10^{-5}$ | $4.4\times10^{-8}$ | $9.8\times10^{7}$ |
| $\sum$ | | | $9.95\times10^{-1}$ | | $4.2\times10^{-7}$ | $4.7\times10^{9}$ |

Table 125: $\varepsilon = 0.05$, $\Delta t_1 = 9.77 \times 10^{-6}$

| $\ell$ | $\Delta t_\ell$ | $P_\ell$ | $\mathbb{E}[\hat{F}_\ell - \hat{F}_{\ell-1}]$ | $\mathbb{V}[\hat{F}_\ell - \hat{F}_{\ell-1}]$ | $\mathbb{V}[\hat{Y}_\ell]$ | $P_\ell C_\ell$ |
|---|---|---|---|---|---|---|
| 0 | $5.0\times10^{-1}$ | $6.9\times10^{8}$ | $9.97\times10^{-1}$ | $2.0\times10^{0}$ | $2.9\times10^{-9}$ | $1.4\times10^{7}$ |
| 1 | $9.8\times10^{-6}$ | $5.7\times10^{5}$ | $-4.60\times10^{-3}$ | $7.1\times10^{-2}$ | $1.2\times10^{-7}$ | $5.9\times10^{8}$ |
| 2 | $4.9\times10^{-6}$ | $1.2\times10^{5}$ | $1.02\times10^{-3}$ | $9.0\times10^{-3}$ | $7.6\times10^{-8}$ | $3.7\times10^{8}$ |
| 3 | $2.4\times10^{-6}$ | $6.3\times10^{4}$ | $7.15\times10^{-4}$ | $5.0\times10^{-3}$ | $8.0\times10^{-8}$ | $3.9\times10^{8}$ |
| 4 | $1.2\times10^{-6}$ | $2.9\times10^{4}$ | $1.76\times10^{-4}$ | $2.3\times10^{-3}$ | $7.8\times10^{-8}$ | $3.6\times10^{8}$ |
| 5 | $6.1\times10^{-7}$ | $1.7\times10^{4}$ | $1.27\times10^{-4}$ | $1.5\times10^{-3}$ | $8.7\times10^{-8}$ | $4.2\times10^{8}$ |
| 6 | $3.1\times10^{-7}$ | $5.6\times10^{3}$ | $-6.95\times10^{-5}$ | $3.0\times10^{-4}$ | $5.3\times10^{-8}$ | $2.8\times10^{8}$ |
| 7 | $1.5\times10^{-7}$ | $1.0\times10^{3}$ | $1.46\times10^{-4}$ | $4.3\times10^{-5}$ | $4.3\times10^{-8}$ | $9.8\times10^{7}$ |
| $\sum$ | | | $9.95\times10^{-1}$ | | $5.4\times10^{-7}$ | $2.5\times10^{9}$ |

Table 126: $\varepsilon = 0.05$, $\Delta t_1 = 4.88 \times 10^{-6}$

| $\ell$ | $\Delta t_\ell$ | $P_\ell$ | $\mathbb{E}[\hat{F}_\ell - \hat{F}_{\ell-1}]$ | $\mathbb{V}[\hat{F}_\ell - \hat{F}_{\ell-1}]$ | $\mathbb{V}[\hat{Y}_\ell]$ | $P_\ell C_\ell$ |
|---|---|---|---|---|---|---|
| 0 | $5.0\times10^{-1}$ | $5.1\times10^{8}$ | $9.98\times10^{-1}$ | $2.0\times10^{0}$ | $3.9\times10^{-9}$ | $1.0\times10^{7}$ |
| 1 | $4.9\times10^{-6}$ | $3.0\times10^{5}$ | $-3.60\times10^{-3}$ | $6.9\times10^{-2}$ | $2.3\times10^{-7}$ | $6.1\times10^{8}$ |
| 2 | $2.4\times10^{-6}$ | $4.4\times10^{4}$ | $-9.33\times10^{-7}$ | $4.3\times10^{-3}$ | $9.9\times10^{-8}$ | $2.7\times10^{8}$ |
| 3 | $1.2\times10^{-6}$ | $2.3\times10^{4}$ | $5.32\times10^{-4}$ | $2.4\times10^{-3}$ | $1.0\times10^{-7}$ | $2.9\times10^{8}$ |
| 4 | $6.1\times10^{-7}$ | $6.0\times10^{3}$ | $3.15\times10^{-5}$ | $7.8\times10^{-4}$ | $1.3\times10^{-7}$ | $1.5\times10^{8}$ |
| 5 | $3.1\times10^{-7}$ | $1.0\times10^{3}$ | $-2.59\times10^{-4}$ | $9.2\times10^{-5}$ | $9.2\times10^{-8}$ | $4.9\times10^{7}$ |
| $\sum$ | | | $9.94\times10^{-1}$ | | $6.6\times10^{-7}$ | $1.4\times10^{9}$ |

Table 127: $\varepsilon = 0.05$, $\Delta t_1 = 2.44 \times 10^{-6}$

| $\ell$ | $\Delta t_\ell$ | $P_\ell$ | $\mathbb{E}[\hat{F}_\ell - \hat{F}_{\ell-1}]$ | $\mathbb{V}[\hat{F}_\ell - \hat{F}_{\ell-1}]$ | $\mathbb{V}[\hat{Y}_\ell]$ | $P_\ell C_\ell$ |
|---|---|---|---|---|---|---|
| 0 | $5.0\times10^{-1}$ | $6.5\times10^{8}$ | $9.97\times10^{-1}$ | $2.0\times10^{0}$ | $3.0\times10^{-9}$ | $1.3\times10^{7}$ |
| 1 | $2.4\times10^{-6}$ | $2.7\times10^{5}$ | $-3.00\times10^{-3}$ | $7.0\times10^{-2}$ | $2.6\times10^{-7}$ | $1.1\times10^{9}$ |
| 2 | $1.2\times10^{-6}$ | $2.7\times10^{4}$ | $2.88\times10^{-4}$ | $2.1\times10^{-3}$ | $7.8\times10^{-8}$ | $3.3\times10^{8}$ |
| 3 | $6.1\times10^{-7}$ | $2.2\times10^{4}$ | $2.39\times10^{-4}$ | $1.7\times10^{-3}$ | $7.8\times10^{-8}$ | $5.4\times10^{8}$ |
| 4 | $3.1\times10^{-7}$ | $5.3\times10^{3}$ | $-2.66\times10^{-4}$ | $5.6\times10^{-4}$ | $1.1\times10^{-7}$ | $2.6\times10^{8}$ |
| 5 | $1.5\times10^{-7}$ | $1.0\times10^{3}$ | $5.52\times10^{-4}$ | $4.5\times10^{-4}$ | $4.5\times10^{-7}$ | $9.8\times10^{7}$ |
| $\sum$ | | | $9.95\times10^{-1}$ | | $9.7\times10^{-7}$ | $2.4\times10^{9}$ |

Table 128: $\varepsilon = 0.05$, $\Delta t_1 = 1.22 \times 10^{-6}$

| $\ell$ | $\Delta t_\ell$ | $P_\ell$ | $\mathbb{E}[\hat{F}_\ell - \hat{F}_{\ell-1}]$ | $\mathbb{V}[\hat{F}_\ell - \hat{F}_{\ell-1}]$ | $\mathbb{V}[\hat{Y}_\ell]$ | $P_\ell C_\ell$ |
|---|---|---|---|---|---|---|
| 0 | $5.0\times10^{-1}$ | $7.2\times10^{8}$ | $9.98\times10^{-1}$ | $2.0\times10^{0}$ | $2.7\times10^{-9}$ | $1.4\times10^{7}$ |
| 1 | $1.2\times10^{-6}$ | $2.1\times10^{5}$ | $-3.30\times10^{-3}$ | $7.0\times10^{-2}$ | $3.3\times10^{-7}$ | $1.7\times10^{9}$ |
| 2 | $6.1\times10^{-7}$ | $1.4\times10^{4}$ | $3.06\times10^{-4}$ | $7.1\times10^{-4}$ | $5.1\times10^{-8}$ | $3.5\times10^{8}$ |
| 3 | $3.1\times10^{-7}$ | $1.1\times10^{4}$ | $-7.21\times10^{-5}$ | $4.6\times10^{-4}$ | $4.3\times10^{-8}$ | $5.3\times10^{8}$ |
| 4 | $1.5\times10^{-7}$ | $1.0\times10^{3}$ | $-2.50\times10^{-4}$ | $1.2\times10^{-4}$ | $1.2\times10^{-7}$ | $9.8\times10^{7}$ |
| $\sum$ | | | $9.94\times10^{-1}$ | | $5.5\times10^{-7}$ | $2.7\times10^{9}$ |
